# Supplementary material for: Communication-Efficient Federated Learning with Accelerated Client Gradient
Source: arXiv:2201.03172 source file (2024-04-01)
Supplement: Supplementary file 1 [file appendix.tex]

% !TEX root = ../main.tex
\appendix
\onecolumn

\iffalse
Moreover, we have compared FedACG (without local regularization) with FedAvgM, and FedCM (correction with global momentum for each local iteration) in terms of loss surface.
Figure~\ref{fig:loss_landscape} illustrates that FedACG's local models better generalize to the overall data distribution in contrast to standard momentum-based methods, which partly illustrates that the accelerated client gradient in FedACG effectively mitigates client drift stemming from data heterogeneity.
\fi

\section{Experiments}
\label{sec:hyperparameter}

In this section, we provide the detailed experimental setups used in our study.
This outlines the evaluation metrics, implementation details, choices of hyperparameters, and additional experiments.

\subsection{Setups}
\label{sec:setups}

\paragraph{Evaluation metrics}
To evaluate the generalization performance of the methods, we use the entire test set of CIFAR-10, CIFAR-100, and Tiny-ImageNet.
Since both the training speed as well as the final accuracy are important factors in federated learning, we measure: (i) the performance achieved at a specified number of rounds and (ii) the number of rounds required for an algorithm to attain the desired level of target accuracy, following~\citet{al2020federated}.
For the target accuracies, we first select the median of all the compared methods at round 1000 and another representative value lower than the median.
For the methods that could not achieve the target accuracies within the maximum communication round, we append a $+$ sign to the communication round number.

\paragraph{Implementation details}
We adopt PyTorch~\citep{paszke2019pytorch} to implement FedACG and the other baselines.
We follow the evaluation protocol of~\citet{acar2021federated} and~\citet{xu2021fedcm}.
For local updates, we use the SGD optimizer with a learning rate of $0.1$ for all approaches on the three benchmarks.
%We apply an exponential decay on the local learning rate, and the decay parameter is selected from $\{1.0, 0.998, 0.995\}$.
We apply no momentum to the local SGD, but incorporate the weight decay of $0.001$ to prevent overfitting.
We also employ gradient clipping to increase the stability of the algorithms.
%The number of local training epochs for each client update is set to 5, and the batch size is determined to make the number of local iterations $50$ in all experiments.
%We set the global learning rate as $1$ for all methods except for FedADAM, which is set to $0.01$.

For the experiments on CIFAR-10 and CIFAR-100, we choose 5 as the number of local training epochs (50 iterations) and 0.1 as the local learning rate.
We set the batch size of the local update to 50 and 10 for the 100 and 500 client participation, respectively.
The learning rate decay parameter of each algorithm is selected from \{0.995, 0.998, 1\} to achieve the best performance.
The global learning rate is set to 1, except for FedAdam, which is tested with 0.01. \iffalse set to 1.0 except for FedAdam, which is set to 0.01.\fi

For the experiments on Tiny-ImageNet, we match the total local iterations of local updates with other benchmarks by setting the batch size of local updates as 100 and 20 for the 100 and 500 client participation, respectively.

\paragraph{Hyperparameter selection}
For the hyperparameter selection, we assume the scenario that the server can compute the validation accuracy through communication with clients at the early stages, which is common to all algorithms.
$\alpha$ in FedCM is selected from \{0.1, 0.3, 0.5\}, $\alpha$ in FedDyn is selected from \{0.001, 0.01,  0.1\}, and $\alpha$ in FedDC is set to 0.01.
 $\tau$ in FedAdam is set to 0.001 while $\mu$ in MOON is set to 1.
$\beta$ in FedAvgM is selected from \{0.4, 0.6, 0.8\}, $\beta$ in FedProx and FedACG is selected from \{0.1, 0.01, 0.001\}, and $\lambda$ in FedACG is selected from \{0.8, 0.85, 0.9\}.

\subsection{Additional analysis for the effect of accelerated client gradient}
\label{sec:additional_ablation}

FedACG uses a lookahead model, $\theta ^{t-1} + \lambda m^{t-1}$, to start local training. 
This helps clients match their local solutions with the global loss, ensuring consistent updates.
We observe more empirical evidence that supports our claim.

Figure~\ref{fig:acc_acg_avgM} shows the convergence curves of FedACG and FedAvgM on CIFAR-10 in the moderate-scale setting without smoothing. 
%we compare the learning curves of FedACG and FedAvgM on CIFAR-10 in the moderate-scale setting without smoothing (exponential moving average) in Figure~\ref{fig:acc_acg_avgM}. 
For the experiments, we set the momentum coefficient to 0.85 for both algorithms. 
We observe that FedACG consistently outperforms FedAvgM and has a smaller accuracy variation throughout the training procedure.
Specifically, when we compute the average squared difference between the accuracy at time step $t$ without smoothing ($\text{Acc}^t$) and the accuracy given by the simple moving average ($\text{Acc}^t_{\text{SMA}}$) over 1,000 rounds of communication, \ie $\frac{1}{T} \sum_{t=0}^{T-1} (\text{Acc}^t-\text{Acc}^t_{\text{SMA}})^2$, the differences are 2.26 and 10.30 for FedACG and FedAvgM, respectively. 
We believe that this is partly because the proposed accelerated gradient allows each client's update to compensate for the potential noise in momentum, which is possible because the local updates start from the anticipated point, $\theta^{t-1} + \lambda m^{t-1}$.

\begin{figure}[h!]
\centering
\includegraphics[width=0.5\linewidth]{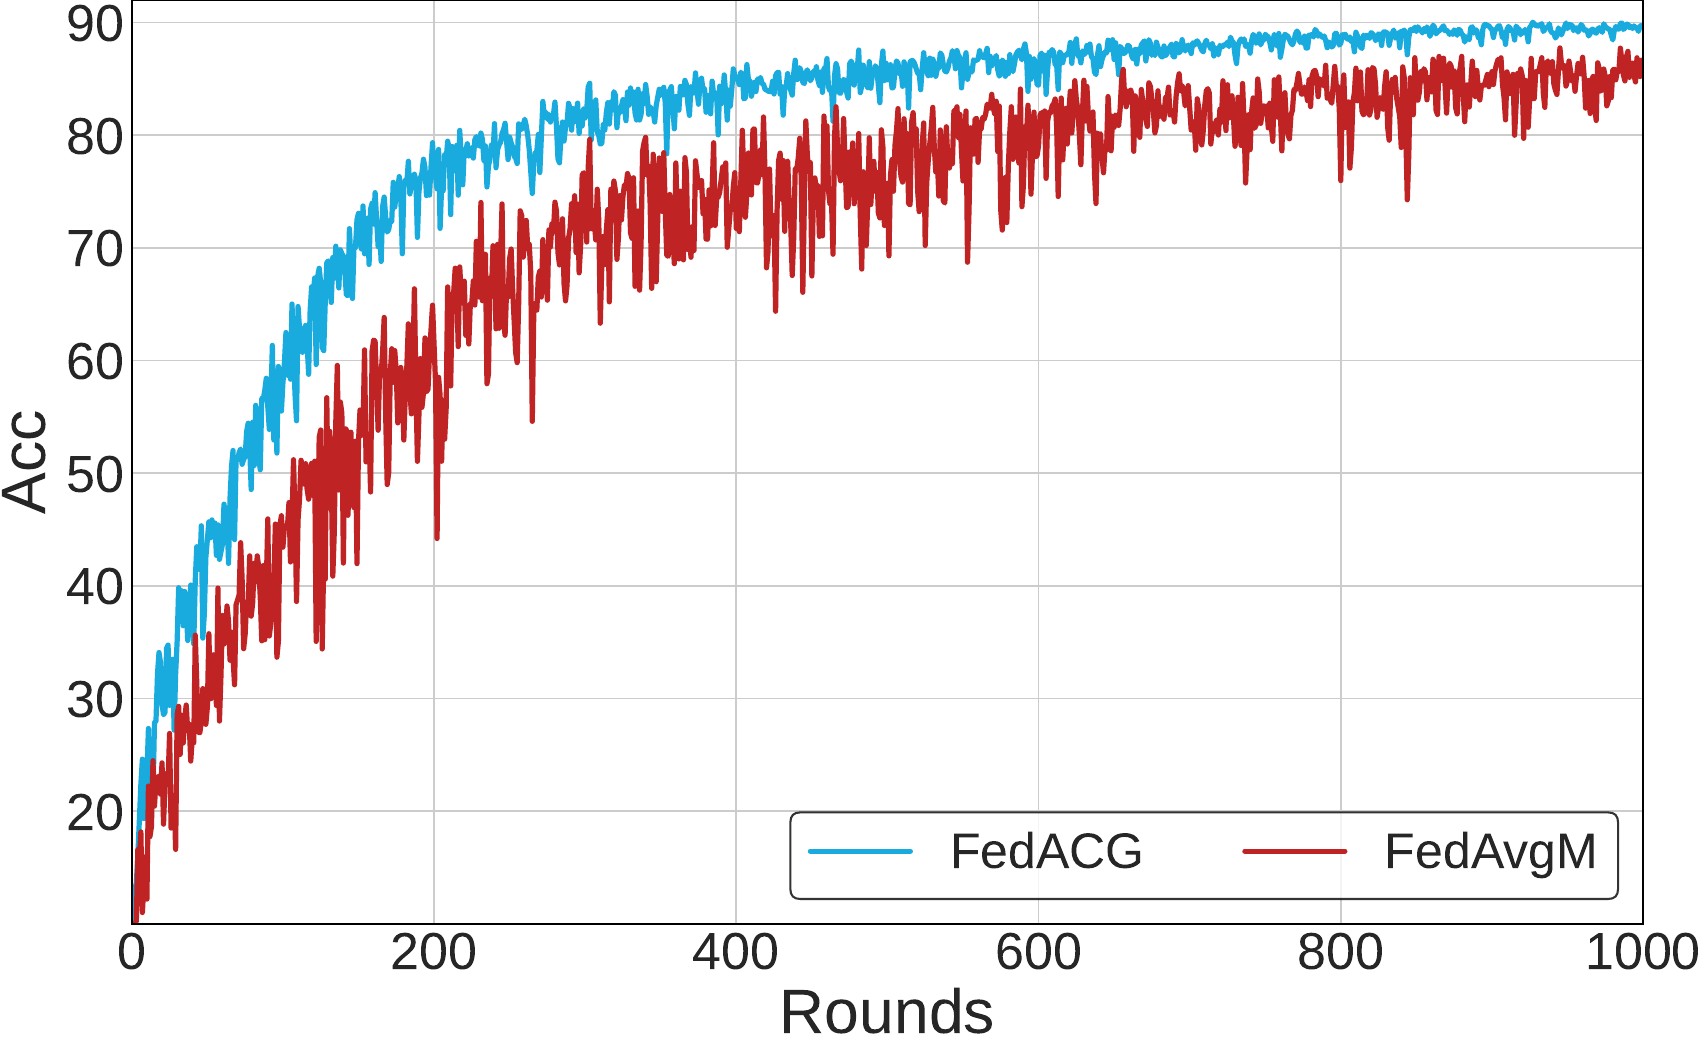}
%t-SNE hyperparameters are consistent in all three visualizations.}
%%\vspace{-0.1cm}
%\end{figure}
%\captionof{figure}{Training curves of FedACG and FedAvgM on CIFAR-10 in a moderate-scale setting.}
\caption{Training curves of FedACG and FedAvgM on CIFAR-10 in a moderate-scale setting without smoothing (exponential moving average).}
\label{fig:acc_acg_avgM}
\end{figure}

\subsection{FedACG with other local objectives}
In Table~\ref{tab:fedmlb}, we incorporate accelerated client gradient into a client-side optimization technique, FedMLB~\citep{kim2022multi}, to test its benefits.
"+ACG" means adopting the relaxed initialization.
It shows that the relaxed initialization helps client-side optimization approaches achieve significant improvements without any additional communication costs.

%%%%%%%%%%%%%%%%%%%%%%%%%% Other local objectives %%%%%%%%%%%%%%%%%%%%%%%%%%%%%%%
\begin{table*}[h!]
\caption{We incorporated accelerated client gradient (ACG) into client-side optimization technique on CIFAR-100 and Tiny-ImageNet.
%Accuracies at the target round and the communication round to reach target test accuracy are based on running exponential moving averages with parameter $0.9$.
%The arrows indicate whether higher ($\uparrow$) or lower ($\downarrow$) is better.
%The best performance in each column is denoted in {\bf bold}.
%FedCM$^\dagger$ and FedDC$^\ddagger$ require 50\% and 100\% additional communication costs at each communication round, respectively.
}
\label{tab:fedmlb}
\begin{subtable}[t]{1\textwidth}
\begin{center}
\captionof{table}{100 clients, 5\% participation, Dirichlet (0.3)}
\scalebox{0.85}{
%\setlength\tabcolsep{3pt}
%\hspace{-0.2cm}
\begin{tabular}{lcccccccc} 
\toprule
\multirow{3}{*}{Method}    & \multicolumn{4}{c}{CIFAR-100}                                                                     & \multicolumn{4}{c}{Tiny-ImageNet}  \\ 
%\cline{2-9}
\cmidrule(lr){2-9}
 & \multicolumn{2}{c}{Acc. (\%, $\uparrow$)} & \multicolumn{2}{c}{Rounds ($\downarrow$)} & \multicolumn{2}{c}{Acc. (\%, $\uparrow$)} & \multicolumn{2}{c}{Rounds ($\downarrow$)}  \\
                                          & \multicolumn{1}{c}{500R}           & \multicolumn{1}{c}{1000R}     & 47\%         & 55\%                            & 500R           & \multicolumn{1}{c}{1000R}    & 35\%         & 38\%                                     \\ 
%\cline{1-9}
%\cmidrule(lr){2-9}
\midrule
FedMLB~\citep{kim2022multi}                       & {47.39} &  {54.58} & 488 & 1000+ &{37.20} &{40.16} & {414}&  {539}\\
FedMLB + ACG                 & \bf{61.32} &  \bf{65.67} & \bf{216} & \bf{316} &\bf{46.11} &\bf{50.54} & \bf{205}&  \bf{260}\\

%\cline{1-9}
\bottomrule
%\label{tab:clients100_prate5}
\end{tabular}}
\end{center}
\end{subtable}
%\vspace{-0.3cm}

\begin{center}
\begin{subtable}[t]{1\textwidth}
\centering
\captionof{table}{500 clients, 2\% participation, Dirichlet (0.3)}
\scalebox{0.85}{
%\setlength\tabcolsep{3pt}
%\hspace{-0.2cm}
\begin{tabular}{lcccccccc} 
\toprule
\multirow{3}{*}{Method}    & \multicolumn{4}{c}{CIFAR-100}                                                                     & \multicolumn{4}{c}{Tiny-ImageNet}  \\ 
%\cline{2-9}
\cmidrule(lr){2-9}
 & \multicolumn{2}{c}{Acc. (\%, $\uparrow$)} & \multicolumn{2}{c}{Rounds ($\downarrow$)} & \multicolumn{2}{c}{Acc. (\%, $\uparrow$)} & \multicolumn{2}{c}{Rounds ($\downarrow$)}  \\
                                          & \multicolumn{1}{c}{500R}           & \multicolumn{1}{c}{1000R}     & 36\%         & 40\%                            & 500R           & \multicolumn{1}{c}{1000R}    & 24\%         & 30\%                                     \\ 
%\cline{1-9}
%\cmidrule(lr){2-9}
\midrule
FedMLB~\citep{kim2022multi}                       & {32.30} &  {42.61} & 642 & 800 &{28.39} &{33.67} & {384}&  {489}\\
FedMLB + ACG                 & \bf{41.10} &  \bf{55.27} & \bf{402} & \bf{479} &\bf{35.92} &\bf{43.85} & \bf{209}&  \bf{313}\\

%\cline{1-9}
\bottomrule
%\label{tab:clients100_prate5}
\end{tabular}}
\end{subtable}
\end{center}
\end{table*}
%%%%%%%%%%%%%%%%%%%%%%%%%%%%%%%%%%%%%%%%%%%%%%%%%%%%%%%%%%%%%%%%%%%%%%%%%%%%%%%

\subsection{Evaluation on Various Data Heterogeneity}
Tables~\ref{tab:dir06} and~\ref{tab:iid} show that FedACG matches or outperforms the performance of competitive methods when data heterogeneity is not severe (Dirichlet 0.6) or very low (\textit{i.i.d.}) on CIFAR-10 in most cases. 
Note that, while the compared methods show performance degradation as the participation rate decreases, FedACG shows little degradation as the participation rate decreases for both data splits.
This implies that FedACG is more robust for low participation rates than other baselines.
This is partly because low client heterogeneity reduces noise in the momentum of the global gradient, which attributes to the smooth trajectory of global updates.
Since FedACG effectively incorporates the momentum for local updates, FedACG is relatively unaffected by the partial participation of federated learning.

%We present the performance of the proposed approach, FedACG, and other federated learning algorithms with various data heterogeneity on CIFAR-10 and CIFAR-100 for two different participation rates. 
%Table~\ref{tab:cifar100_d_0.6_iid} shows that FedACG outperforms the baselines in terms of accuracy and convergence speed with large margins for most cases.
%Note that FedACG shows a larger gain when the participation rate decreases regardless of data heterogeneity, which demonstrates the robustness of FedACG to communication constraints of federated learning.

%%%%%%%%%%%%%%%%%%%%%%%%%% Dir06 %%%%%%%%%%%%%%%%%%%%%%%%%%%%%%%
\begin{table*}[h!]
\caption{Results with Dirichlet (0.6) data on CIFAR-10 and CIFAR-100 for two different settings. 
%Accuracies at the target round and the communication round to reach target test accuracy are based on running exponential moving averages with parameter $0.9$.
%The arrows indicate whether higher ($\uparrow$) or lower ($\downarrow$) is better.
%The best performance in each column is denoted in {\bf bold}.
%FedCM$^\dagger$ and FedDC$^\ddagger$ require 50\% and 100\% additional communication costs at each communication round, respectively.
}
\label{tab:dir06}
\begin{subtable}[t]{1\textwidth}
\begin{center}
\captionof{table}{Dirichlet (0.6), 100 clients, 5\% participation}
\scalebox{0.85}{
%\setlength\tabcolsep{3pt}
%\hspace{-0.2cm}
\begin{tabular}{lcccccccc} 
\toprule
\multirow{3}{*}{Method}                                   & \multicolumn{4}{c}{CIFAR-10}                                                                     & \multicolumn{4}{c}{CIFAR-100}                                                                 \\ 
%\cline{2-9}
\cmidrule(lr){2-9}
 & \multicolumn{2}{c}{Acc. (\%, $\uparrow$)} & \multicolumn{2}{c}{Rounds ($\downarrow$)} & \multicolumn{2}{c}{Acc. (\%, $\uparrow$)} & \multicolumn{2}{c}{Rounds ($\downarrow$)}  \\
                                          & \multicolumn{1}{c}{500R}           & \multicolumn{1}{c}{1000R}     & 81\%         & 87\%                            & 500R           & \multicolumn{1}{c}{1000R}    & 50\%         & 56\%                                     \\ 
%\cline{1-9}
%\cmidrule(lr){2-9}
\midrule
FedAvg~\citep{mcmahan2017communication}  &80.56 & 85.97& 520 & 1000+ & 43.91 & 49.18 & 1000+ & 1000+ \\
FedProx~\citep{li2018federated}        & 80.39 & 85.53 & 524 & 1000+ & 43.15 &48.45 &1000+ &  1000+ \\
FedAvgM~\citep{hsu2019measuring}      & 84.65 & 87.96 & 355 & 811 &46.66  & 52.49 & 735 & 1000+  \\
FedADAM~\citep{reddi2021adaptive}       & 80.25 & 83.52 &526& 1000+ &45.95 & 51.63 & 778& 1000+  \\
FedDyn~\citep{acar2021federated}      & 87.23 & 89.49 & 310 & 487 & 50.51 &56.78 & 488& 886    \\
MOON~\citep{li2021model}           & 84.95 & 87.99 & 272 & 728 & 55.76 & 61.42 & 338 & 527 \\ 
\rowcolor{Gray}
FedCM$^{\dagger}$~\citep{xu2021fedcm}           & 82.84 & 86.64 & 385  & 1000+ &53.75 &60.48 &331 & 468    \\
\rowcolor{Gray}
FedDC$^{\ddagger}$~\citep{gao2022feddc}           & \bf88.05 & 89.58 & 270 & {\bf437} & 56.00 & 60.58 & 347 & 491 \\ 
%FedSAM~\citep{qu2022generalized}           &76.87&86.30&625&851&43.52&50.60&1000+&1000+\\ 
FedACG (ours)                       & {87.57} &  \bf{90.56} & \bf{218} & 453 &\bf{58.82} &\bf{63.88} & \bf{243}&  \bf{396}\\
%\cline{1-9}
\bottomrule
%\label{tab:clients100_prate5}
\end{tabular}}
\end{center}
\end{subtable}
%\vspace{-0.3cm}

\begin{center}
\begin{subtable}[t]{1\textwidth}
\centering
\captionof{table}{Dirichlet (0.6), 500 clients, 2\% participation}
\scalebox{0.85}{
%\setlength\tabcolsep{3pt}
%\hspace{-0.2cm}
\begin{tabular}{lcccccccc} 
\toprule
\multirow{3}{*}{Method}                                   & \multicolumn{4}{c}{CIFAR-10}                                                                     & \multicolumn{4}{c}{CIFAR-100}                                                                 \\ 
%\cline{2-9}
\cmidrule(lr){2-9}
 & \multicolumn{2}{c}{acc. (\%, $\uparrow$)} & \multicolumn{2}{c}{rounds ($\downarrow$)} & \multicolumn{2}{c}{acc. (\%, $\uparrow$)} & \multicolumn{2}{c}{rounds ($\downarrow$)}  \\
                                          & \multicolumn{1}{c}{500R}           & \multicolumn{1}{c}{1000R}     & 69\%         & 80\%                            & 500R           & \multicolumn{1}{c}{1000R}    & 32\%         & 41\%                                     \\ 
%\cline{1-9}
\midrule
FedAvg~\citep{mcmahan2017communication}  & 62.79 & 75.17 & 671 &1000+  & 29.41 & 36.62 &648&1000+ \\
FedProx~\citep{li2018federated}          & 62.48 & 75.10 &688&1000+& 29.62 & 36.70 &647&1000+ \\
FedAvgM~\citep{hsu2019measuring}         & 69.10 & 80.26 &498&981& 32.78 & 41.93 &468  &942 \\
FedADAM~\citep{reddi2021adaptive}        & 68.48 & 78.92 &535&1000+& 37.57 & 48.29 &341&624 \\
FedDyn~\citep{acar2021federated}         & 68.53 & 80.33 &513&983& 32.06 & 43.28 &498& 917 \\
MOON~\citep{li2021model}                 & 74.29 & 80.66 & 368 & 921 & 31.64 & 41.61 & 515 & 931 \\ 
\rowcolor{Gray}
FedCM$^{\dagger}$~\citep{xu2021fedcm}                & 71.42 & 78.94 &429&1000+& 26.82 & 39.78 &714&1000+\\
\rowcolor{Gray}
FedDC$^{\ddagger}$~\citep{gao2022feddc}               & 77.74 & {\bf86.32} & 324 & 596 & 34.24 & 44.69 & 444 & 825\\ 
%FedSAM~\citep{qu2022generalized}         &57.41&71.51&&&29.02&36.71&&\\ 
FedACG (ours)                            & {\bf78.49} & 85.28 & {\bf289}& {\bf565} & {\bf39.61} & {\bf49.70} & {\bf304}& {\bf540}\\
%\cline{1-9}
\bottomrule
%\label{tab:clients100_prate5}
\end{tabular}}
\end{subtable}
\end{center}
\vspace{-0.4cm}
\end{table*}
%%%%%%%%%%%%%%%%%%%%%%%%%%%%%%%%%%%%%%%%%%%%%%%%%%%%%%%%%%%%%%%%%%%%%%%%%%%%%%%

%%%%%%%%%%%%%%%%%%%%%%%%%% IID %%%%%%%%%%%%%%%%%%%%%%%%%%%%%%%
\begin{table*}[h!]
\caption{Results with \textit{i.i.d.} data on CIFAR-10 and CIFAR-100 for two different settings. 
%Accuracies at the target round and the communication round to reach target test accuracy are based on running exponential moving averages with parameter $0.9$.
%The arrows indicate whether higher ($\uparrow$) or lower ($\downarrow$) is better.
%The best performance in each column is denoted in {\bf bold}.
%FedCM$^\dagger$ and FedDC$^\ddagger$ require 50\% and 100\% additional communication costs at each communication round, respectively.
}
\label{tab:iid}
\begin{subtable}[t]{1\textwidth}
\begin{center}
\captionof{table}{\textit{i.i.d.}, 100 clients, 5\% participation}
\scalebox{0.85}{
%\setlength\tabcolsep{3pt}
%\hspace{-0.2cm}
\begin{tabular}{lcccccccc} 
\toprule
\multirow{3}{*}{Method}                                   & \multicolumn{4}{c}{CIFAR-10}                                                                     & \multicolumn{4}{c}{CIFAR-100}                                                                 \\ 
%\cline{2-9}
\cmidrule(lr){2-9}
 & \multicolumn{2}{c}{acc. (\%, $\uparrow$)} & \multicolumn{2}{c}{rounds ($\downarrow$)} & \multicolumn{2}{c}{acc. (\%, $\uparrow$)} & \multicolumn{2}{c}{rounds ($\downarrow$)}  \\
                                          & \multicolumn{1}{c}{500R}           & \multicolumn{1}{c}{1000R}     & 82\%         & 89\%                            & 500R           & \multicolumn{1}{c}{1000R}    & 52\%         & 58\%                                     \\ 
%\cline{1-9}
\midrule
FedAvg~\citep{mcmahan2017communication}  & 85.28 &88.69 & 372 & 1000+ & 43.96 & 48.20 & 1000+ & 1000+ \\
FedProx~\citep{li2018federated}        & 84.79 & 87.99 & 384 & 1000+ & 43.57 & 47.75 & 1000+ & 1000+ \\
FedAvgM~\citep{hsu2019measuring}      & 87.67& 89.96 & 258 & 375 & 47.43 & 52.83 & 880 & 1000+  \\
FedADAM~\citep{reddi2021adaptive}       & 85.29 & 87.97 & 286 & 1000+ & 52.23 & 57.73 & 496 & 1000+   \\
FedDyn~\citep{acar2021federated}      & 89.19 & 90.70 & 269 & 492 & 50.37 & 56.88 & 592 &898  \\
MOON~\citep{li2021model}          & 88.24 & 89.96 & 207 & 628 & 58.50 & \bf64.73 & 311 & 484 \\ 
\rowcolor{Gray}
FedCM$^\dagger$~\citep{xu2021fedcm}           & 87.38 & 89.65 & 182 &  782 & 57.10 & {62.48} & 266 & 466 \\
\rowcolor{Gray}
FedDC$^\ddagger$~\citep{gao2022feddc}           & 90.07 & 90.80 & 194 & 425 & 55.17 &
61.00 & 400 & 633 \\ 
%FedSAM~\citep{qu2022generalized}           &84.42&89.61&425&573&45.36&50.74&1000+&1000+\\ 
FedACG (ours)                       & \bf{90.57} &  \bf{92.29} & \bf{157} & \bf{354} & \bf{59.82} & 64.08 &  \bf{244} & \bf{342} \\
%\cline{1-9}
\bottomrule
%\label{tab:clients100_prate5}
\end{tabular}}
\end{center}
\end{subtable}
%\vspace{-0.3cm}

\begin{center}
\begin{subtable}[t]{1\textwidth}
\centering
\captionof{table}{\textit{i.i.d.}, 500 clients, 2\% participation}
\scalebox{0.85}{
%\setlength\tabcolsep{3pt}
%\hspace{-0.2cm}
\begin{tabular}{lcccccccc} 
\toprule
\multirow{3}{*}{Method}                                   & \multicolumn{4}{c}{CIFAR-10}                                                                     & \multicolumn{4}{c}{CIFAR-100}                                                                 \\ 
%\cline{2-9}
\cmidrule(lr){2-9}
 & \multicolumn{2}{c}{acc. (\%, $\uparrow$)} & \multicolumn{2}{c}{rounds ($\downarrow$)} & \multicolumn{2}{c}{acc. (\%, $\uparrow$)} & \multicolumn{2}{c}{rounds ($\downarrow$)}  \\
                                          & \multicolumn{1}{c}{500R}           & \multicolumn{1}{c}{1000R}     & 75\%         & 83\%                            & 500R           & \multicolumn{1}{c}{1000R}    & 33\%         & 42\%                                     \\ 
%\cline{1-9}
\midrule
FedAvg~\citep{mcmahan2017communication}  & 68.70 & 78.21 & 652 & 1000+ & 30.71 & 37.85 & 664 & 1000+ \\
FedProx~\citep{li2018federated}       & 68.74 & 77.96 & 643 & 1000+ & 30.11 & 37.13 & 685 & 1000+ \\
FedAvgM~\citep{hsu2019measuring}      & 74.34 & 83.64 & 523 & 943 & 33.54 & 42.55 & 479 & 971\\
FedADAM~\citep{reddi2021adaptive}     & 75.32 & 84.01 & 491 & 915 & 38.74 & 48.94 & 328 & 636 \\
FedDyn~\citep{acar2021federated}      & 74.81 & 84.71 & 398 & 823 & 33.20 & 42.91 &  492 & 936  \\
MOON~\citep{li2021model}              & 69.86 & 81.89 & 586 & 1000+ & 28.82 & 41.26 & 649 & 1000+\\ 
\rowcolor{Gray}
FedCM$^\dagger$~\citep{xu2021fedcm}             & 77.84 & 83.26 & 491 & 959 & 29.59 & 42.04 & 653 & 991\\
\rowcolor{Gray}
FedDC$^\ddagger$~\citep{gao2022feddc}            & {\bf80.87} & {\bf87.53} & 358 & {\bf574} & 33.93 & 45.80 & 476 & 817 \\ 
%FedSAM~\citep{qu2022generalized}      &&&&&29.42&36.74&&\\ 
FedACG (ours)                         & 80.15 & 87.47 & {\bf316} & 578 & {\bf41.16} & {\bf49.10} & {\bf299} & {\bf525}\\
%\cline{1-9}
\bottomrule
%\label{tab:clients100_prate5}
\end{tabular}}
\end{subtable}
\end{center}
\end{table*}

\clearpage

\subsection{Convergence Plot}

\subsubsection{Evaluation on various federated learning scenarios}
\label{sec:plot_main}
{Figure~\ref{fig:convergence_cifar10} to Figure~\ref{fig:convergence_tiny} show the convergence of FedACG and the compared algorithms on CIFAR-10, CIFAR-100, and Tiny-ImageNet for various federated learning settings: varying the number of total clients, participation rates, data heterogeneity.}
{FedACG continuously matches or exceeds the performance of the most powerful of our competitors in most learning sections.}
%FedACG continuously outperforms baselines in most learning sections.
%Note that FedACG shows larger gains compared to baselines for the large-scale experiment, which implies the robustness of FedACG to data heterogeneity and partial participation.

Figure~\ref{fig:cifar_d_03} shows the convergence plots under massive clients, 1\% participation rate setting.
The result shows that FedACG takes the lead in most learning sections, which also demonstrates the effectiveness of FedACG.

\iffalse
%%%%%%%%%%%%%%%%%%%%%%%%%%%%%%%%%
\begin{figure*}[t]
\centering
\begin{subfigure}[b]{0.45\linewidth}
\centering
\includegraphics[width=1\linewidth]{figures/cifar100_low_500.pdf}
%\vspace{-0.4cm}
%\caption{2\% participation, 500 clients}
\caption{CIFAR-100}
\end{subfigure}
%\rulesep
\hspace{0.4cm}
\begin{subfigure}[b]{0.45\linewidth}
\centering
\includegraphics[width=1\linewidth]{figures/tiny_low_500.pdf}
%\vspace{-0.4cm}
%\caption{1\% participation, 100 clients}
\caption{Tiny-ImageNet}
\end{subfigure}
\caption{
The convergence plots of FedACG and comparison methods for the large-scale experiments on CIFAR-100, and Tiny-ImageNet.
}
%\vspace{-0.2cm}
\label{fig:large_curve}
%\vspace{-0.1cm}
\end{figure*}
%%%%%%%%%%%%%%%%%%%%%%%%%%%%%%%%%%%%%%%%%%%%%%%%%%%%%%%
\fi

%%%%%%%%%%%%%%%%%%%%%% Convergence Plots %%%%%%%%%%%%%%%%%%%%%%%%%%%%%%%%%%%%%%%%%%%%%%%%%%%%%%%%%%%%%%%%%%%%%%%%%%%%%

%%%%%%%%%%%%%% CIFAR-10 %%%%%%%%%%%%%%%%%%%%%%%%%%%%%%%%%%%%%%%%%%%%%%%%%%%%%
\begin{figure}[h!]
\centering
\begin{subfigure}[b]{0.45\linewidth}
\centering
\includegraphics[width=1\linewidth]{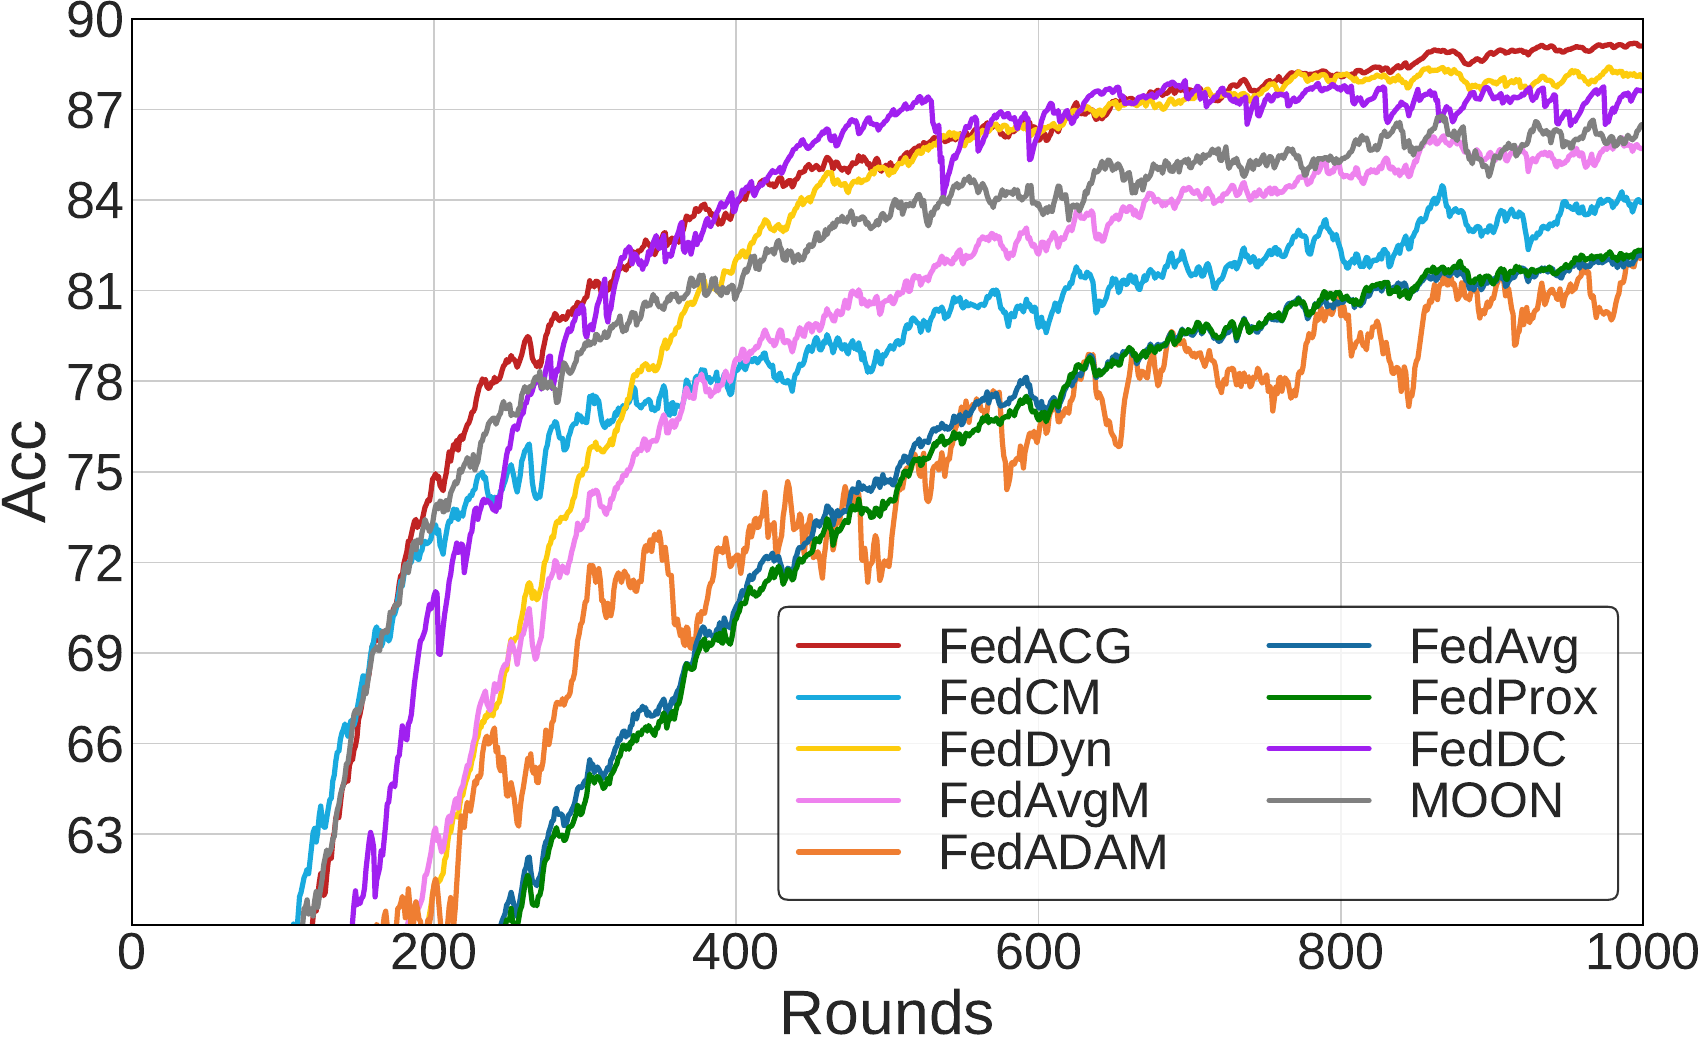}
%\includegraphics[width=1\linewidth]{figures/cifar100_mid_100.pdf}
%\vspace{-0.4cm}
\caption{Dirichlet (0.3), 100 clients, 5\% participation}
\end{subfigure}
%\rulesep
\hspace{0.4cm}
\begin{subfigure}[b]{0.45\linewidth}
\centering
\includegraphics[width=1\linewidth]{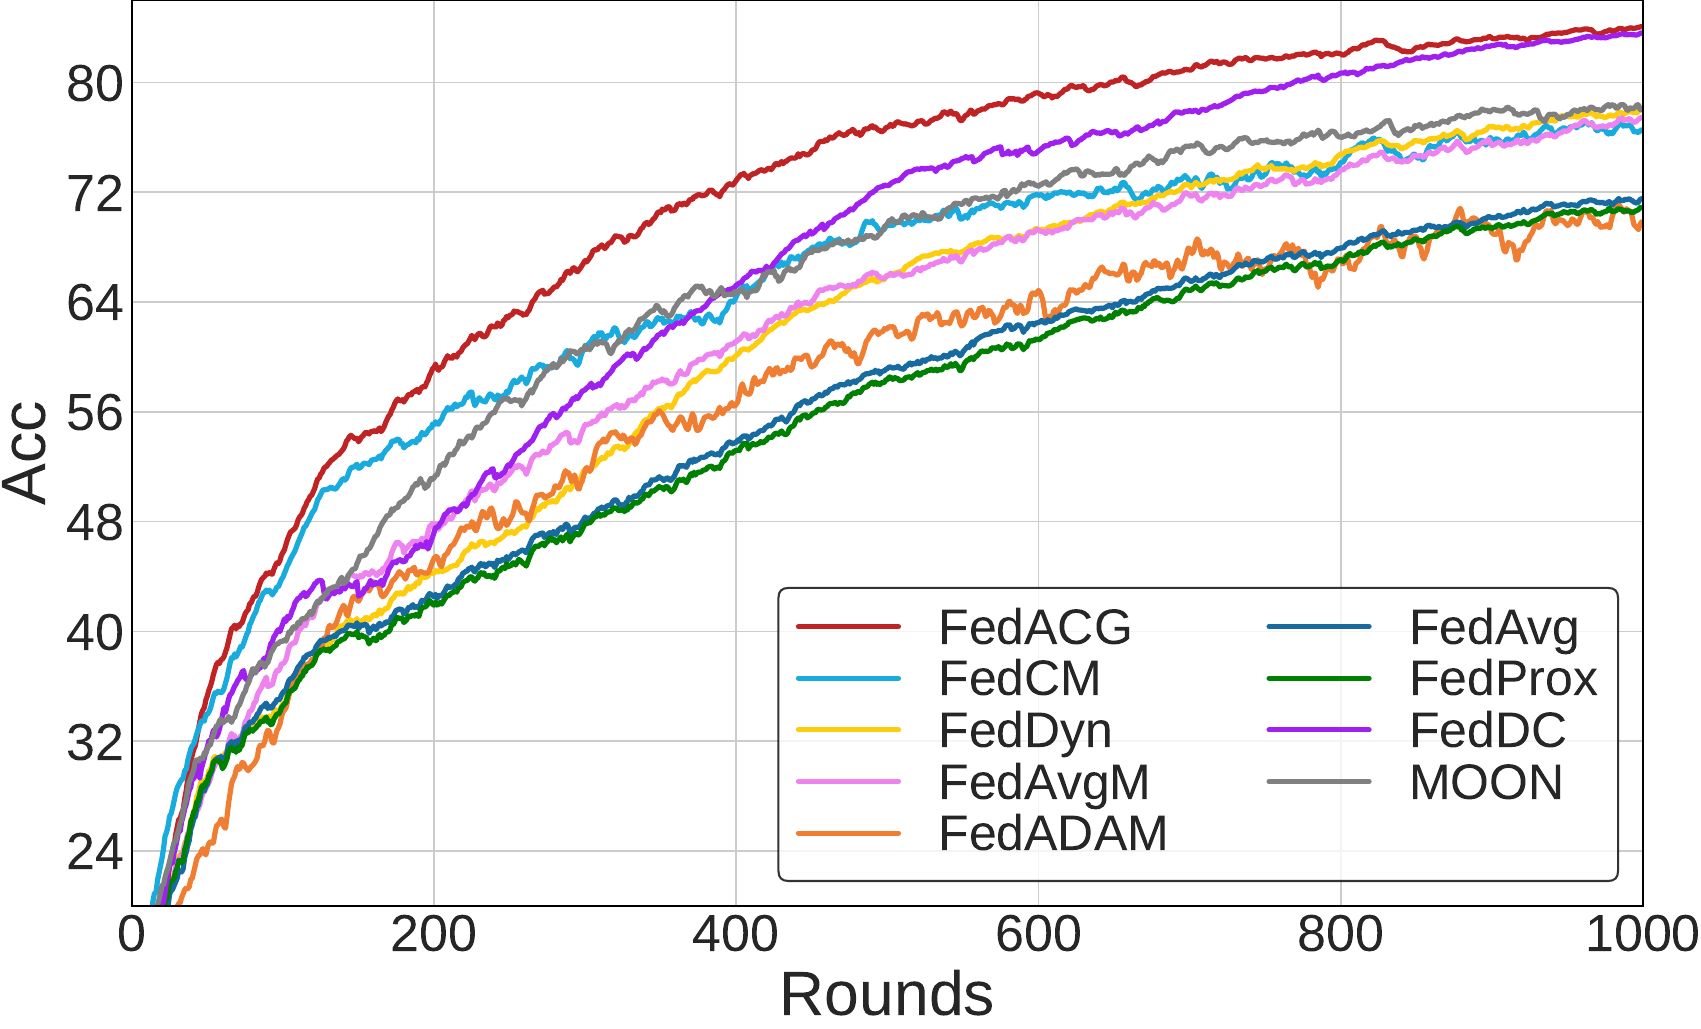}
%\includegraphics[width=1\linewidth]{figures/tiny_mid_100.pdf}
%\vspace{-0.4cm}
\caption{Dirichlet (0.3), 500 clients, 2\% participation}
%\caption{1\% participation, 100 clients}
\end{subfigure}

\vspace{0.6cm}

\begin{subfigure}[b]{0.45\linewidth}
\centering
\includegraphics[width=1\linewidth]{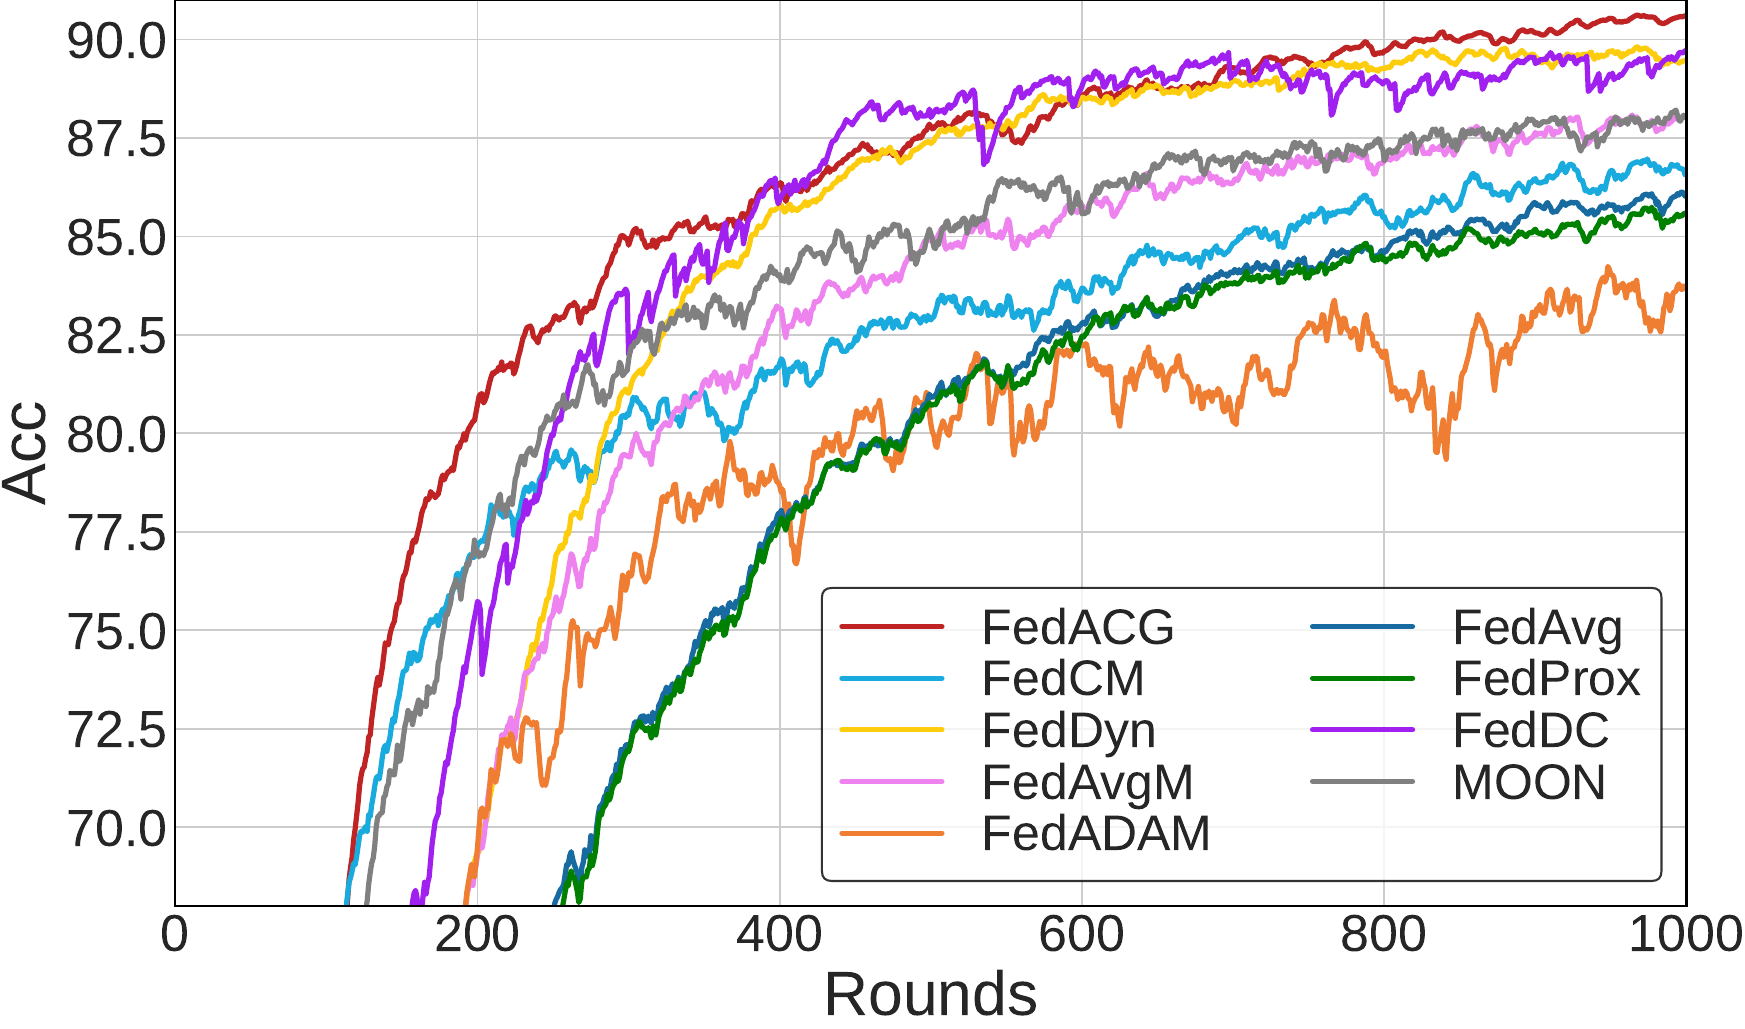}
%\vspace{-0.4cm}
\caption{Dirichlet (0.6), 100 clients, 5\% participation}
\end{subfigure}
%\rulesep
\hspace{0.4cm}
\begin{subfigure}[b]{0.45\linewidth}
\centering
\includegraphics[width=1\linewidth]{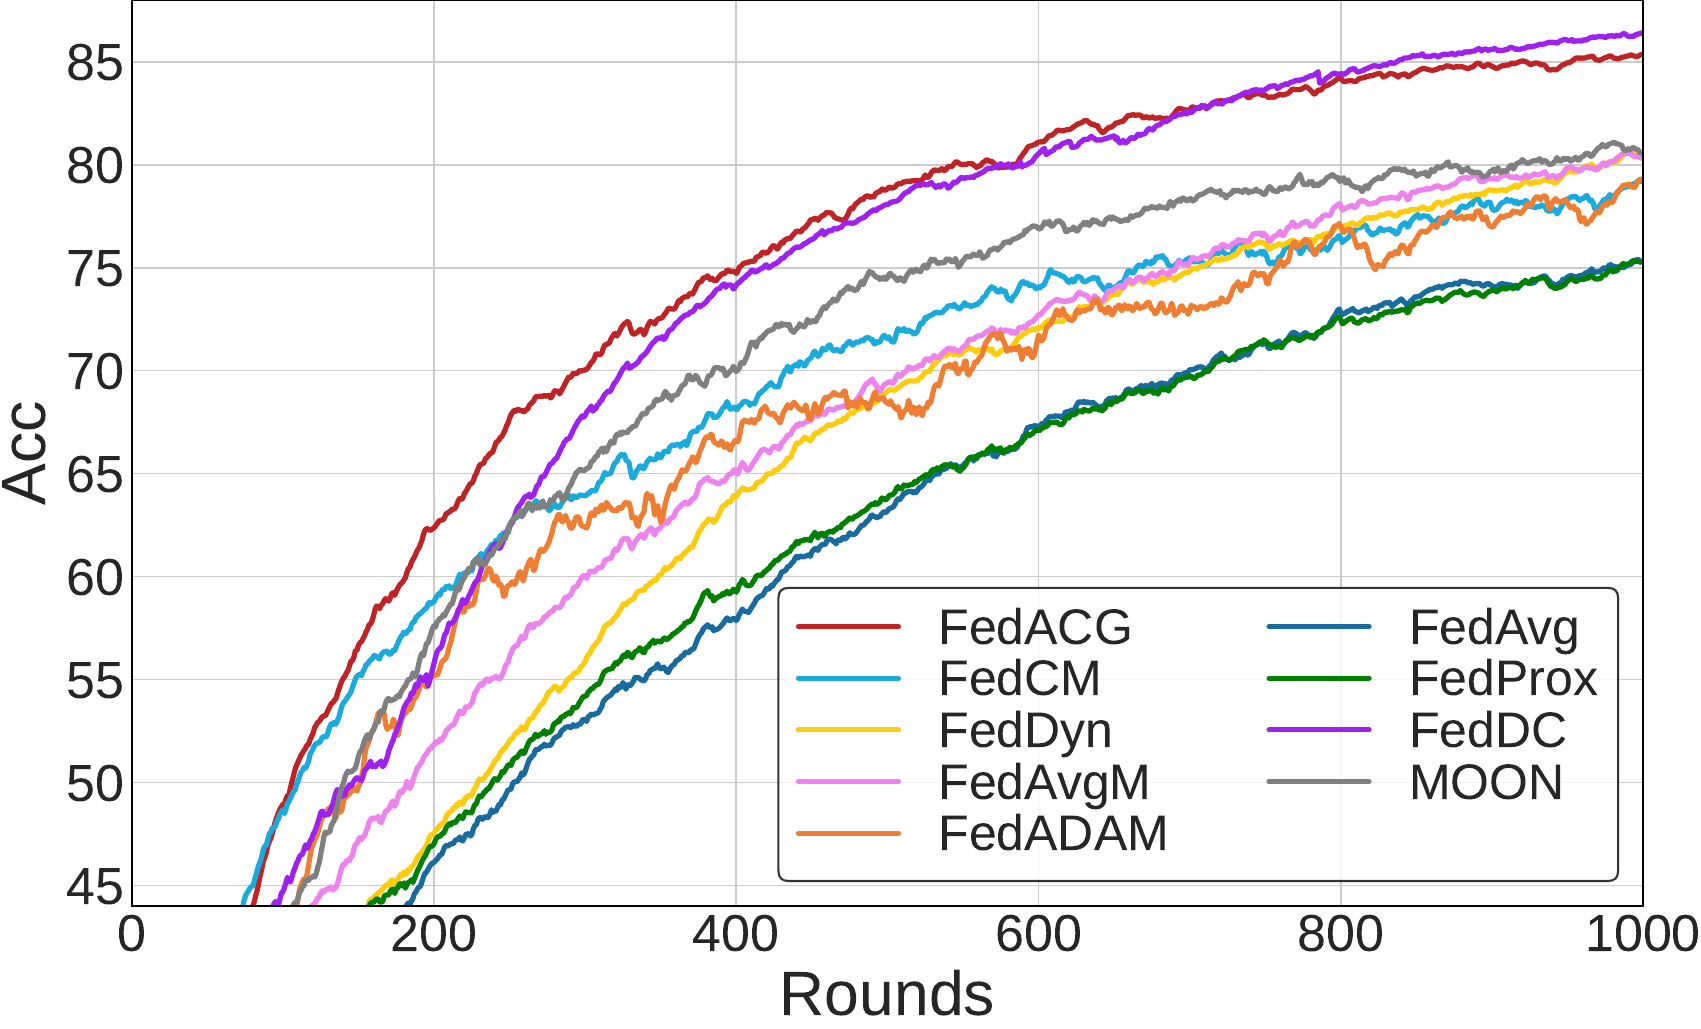}
%\vspace{-0.4cm}
\caption{Dirichlet (0.6), 500 clients, 2\% participation}
%\caption{1\% participation, 100 clients}
\end{subfigure}

\vspace{0.6cm}

\begin{subfigure}[b]{0.45\linewidth}
\centering
\includegraphics[width=1\linewidth]{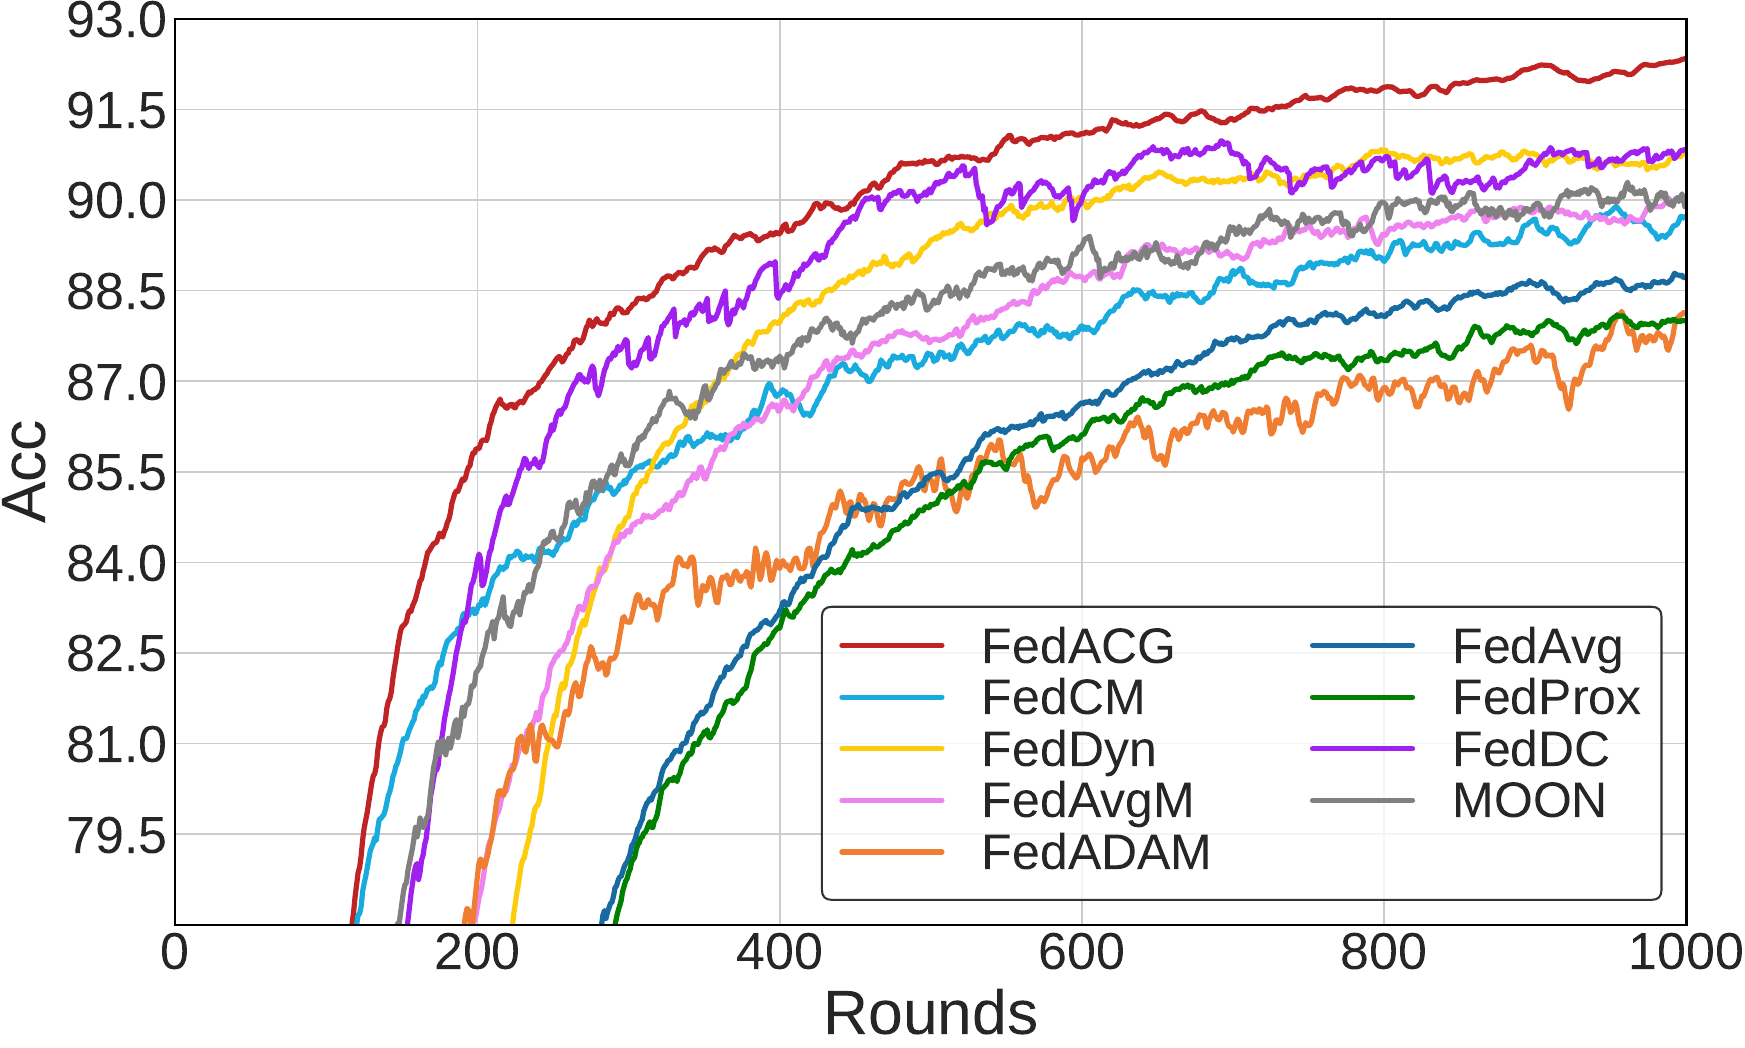}
%\vspace{-0.4cm}
\caption{\textit{i.i.d.}, 100 clients, 5\% participation}
\end{subfigure}
%\rulesep
\hspace{0.4cm}
\begin{subfigure}[b]{0.45\linewidth}
\centering
\includegraphics[width=1\linewidth]{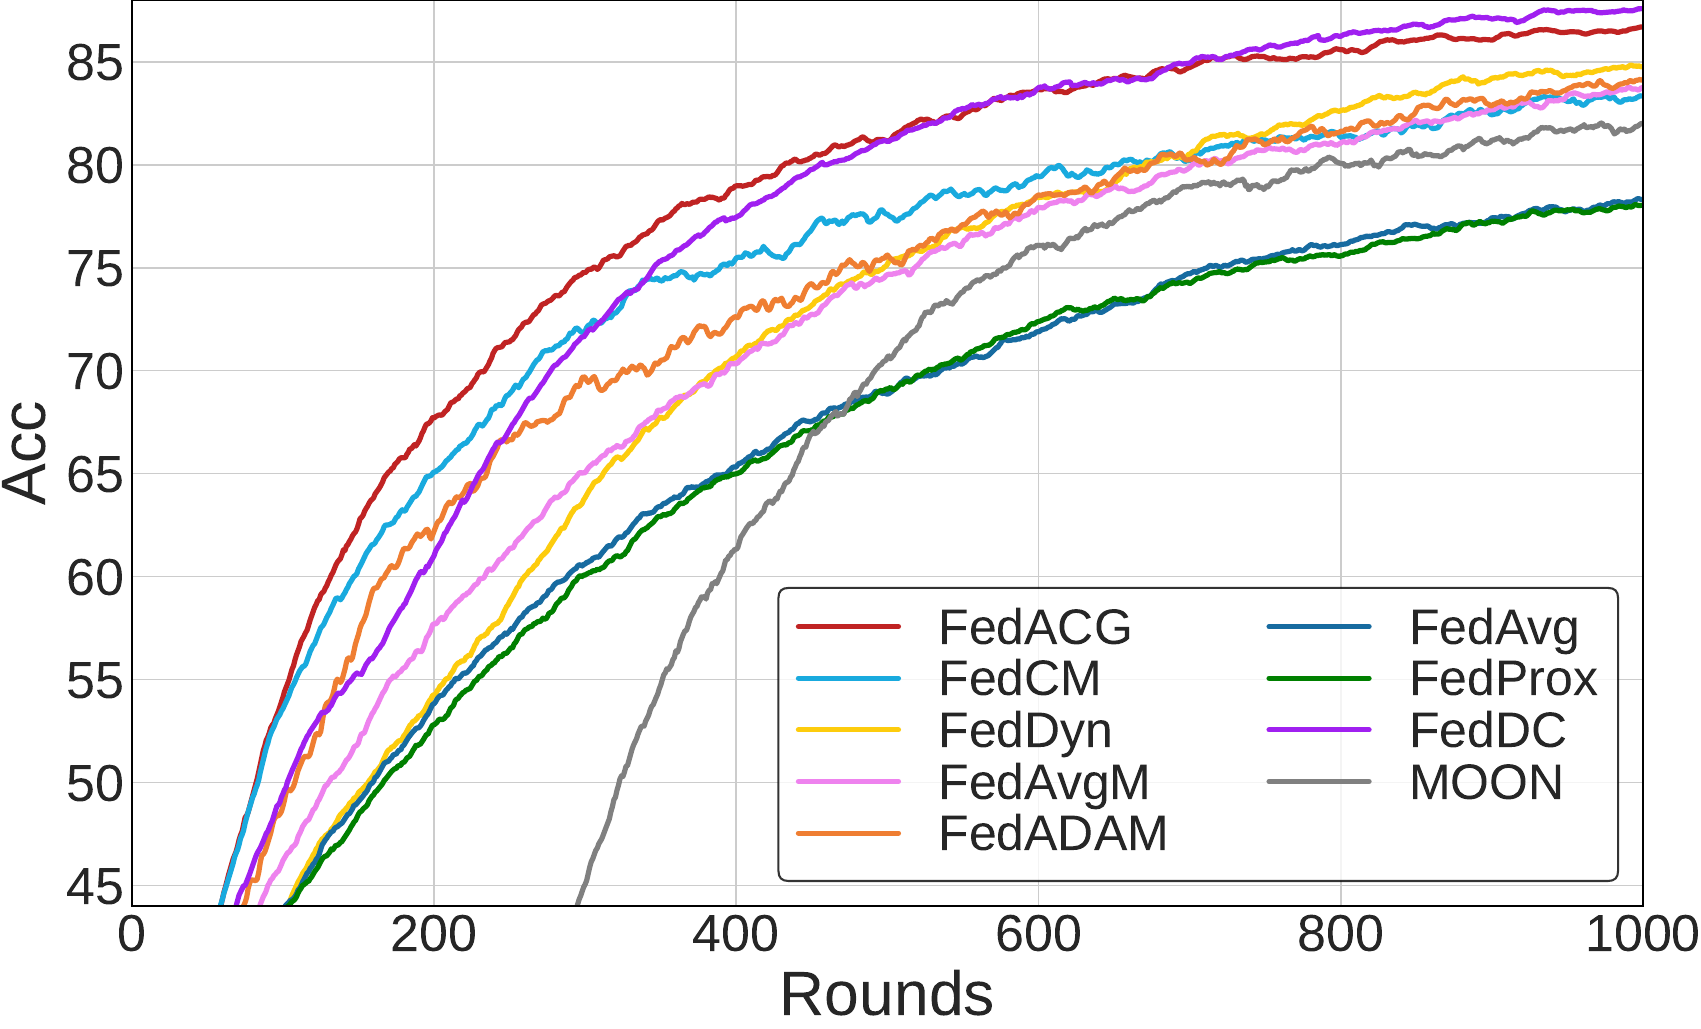}
%\vspace{-0.4cm}
\caption{\textit{i.i.d.}, 500 clients, 2\% participation}
%\caption{1\% participation, 100 clients}
\end{subfigure}
\caption{
The convergence plots of FedACG and the baselines on CIFAR-10 with different federated learning scenarios.
}
%\vspace{-0.8cm}
\label{fig:convergence_cifar10}
\end{figure}
%%%%%%%%%%%%%%%%%%%%%%%%%%%%%%%%%%%%%%%%%%%%%%%%%%%%%%%%%%%%%%%%%%%%%%%%%%%%%%%%%%%%%%%%%%%%%%%%%%%%%%%%%%%%%%%

%%%%%%%%%%%%%% CIFAR-100 %%%%%%%%%%%%%%%%%%%%%%%%%%%%%%%%%%%%%%%%%%%%%%%%%%%%%
\begin{figure}[h!]
\centering
\begin{subfigure}[b]{0.45\linewidth}
\centering
\includegraphics[width=1\linewidth]{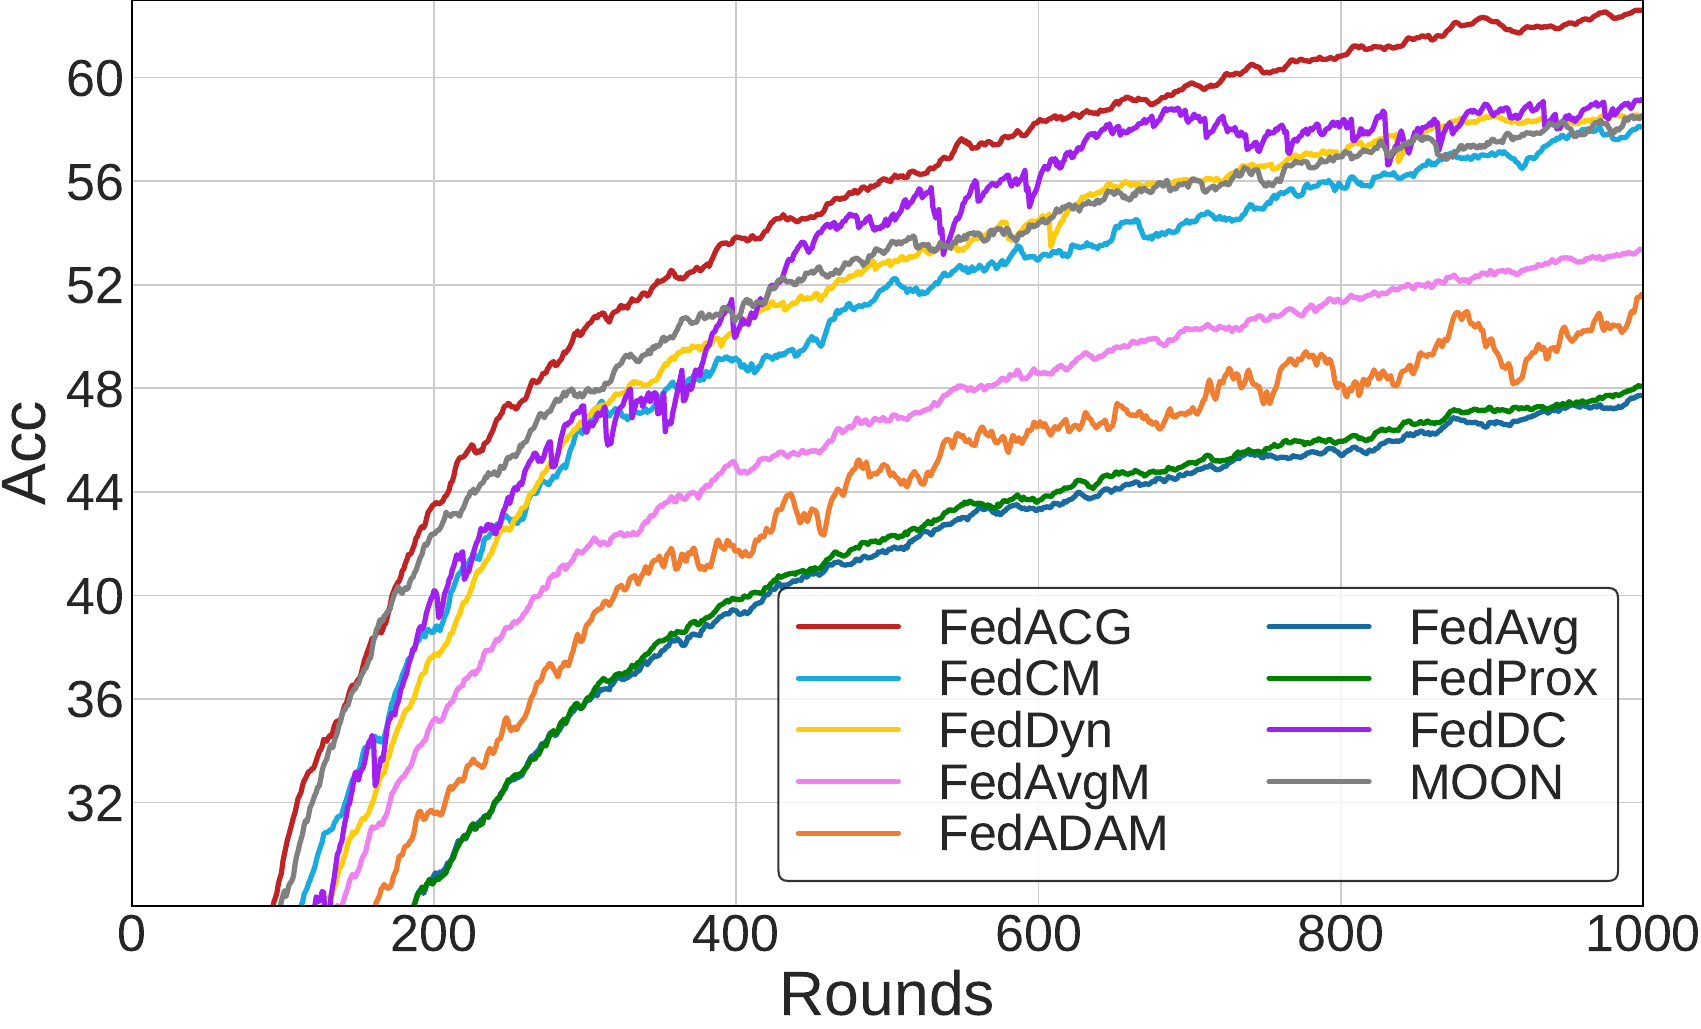}
%\includegraphics[width=1\linewidth]{figures/cifar100_mid_100.pdf}
%\vspace{-0.4cm}
\caption{Dirichlet (0.3), 100 clients, 5\% participation}
\end{subfigure}
%\rulesep
\hspace{0.4cm}
\begin{subfigure}[b]{0.45\linewidth}
\centering
\includegraphics[width=1\linewidth]{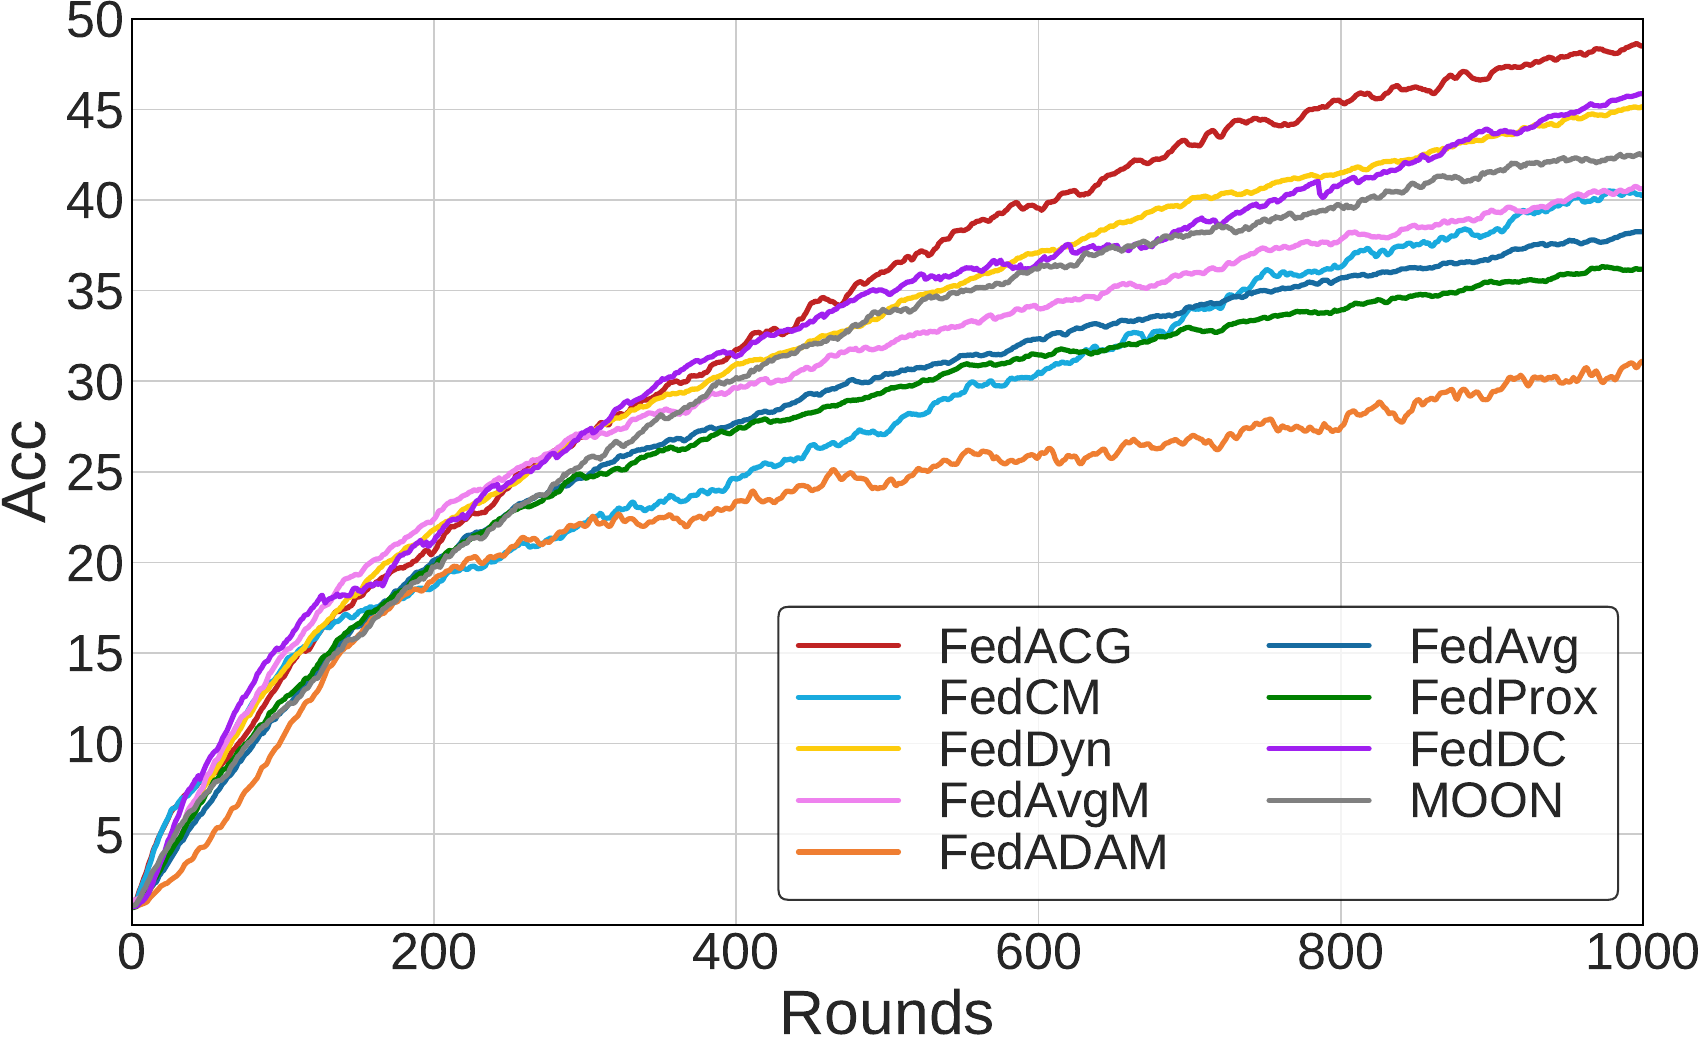}
%\includegraphics[width=1\linewidth]{figures/tiny_mid_100.pdf}
%\vspace{-0.4cm}
\caption{Dirichlet (0.3), 500 clients, 2\% participation}
%\caption{1\% participation, 100 clients}
\end{subfigure}

\vspace{0.6cm}

\begin{subfigure}[b]{0.45\linewidth}
\centering
\includegraphics[width=1\linewidth]{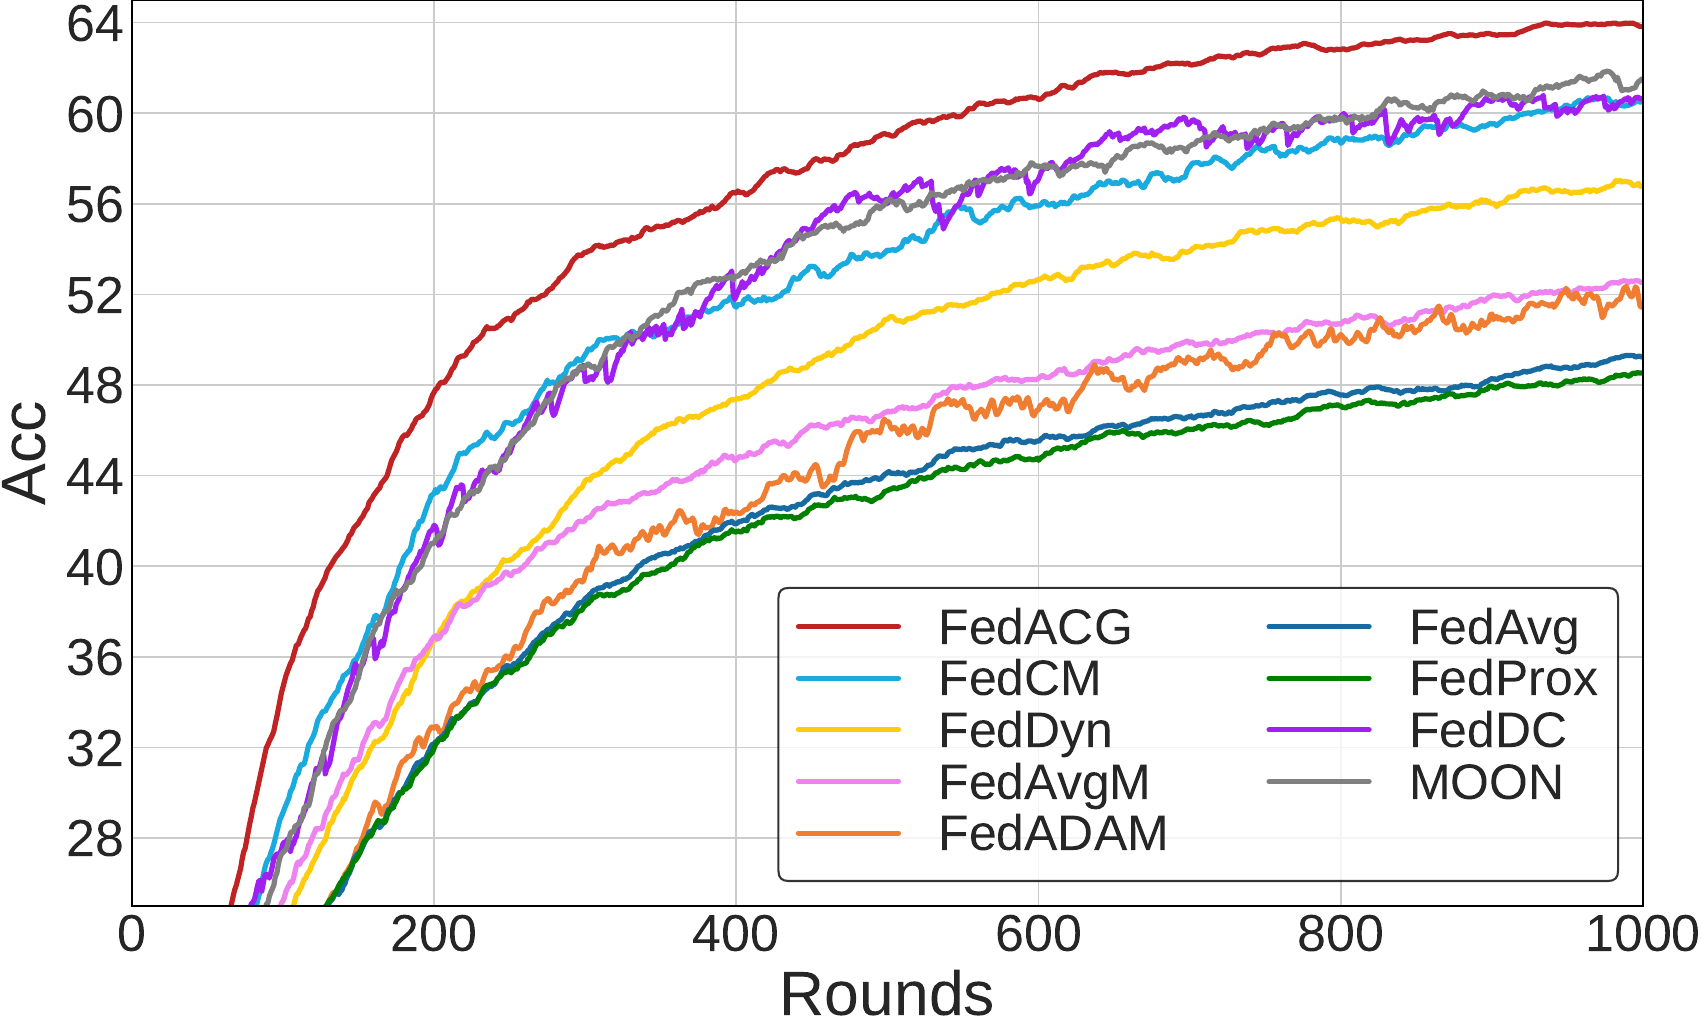}
%\vspace{-0.4cm}
\caption{Dirichlet (0.6), 100 clients, 5\% participation}
\end{subfigure}
%\rulesep
\hspace{0.4cm}
\begin{subfigure}[b]{0.45\linewidth}
\centering
\includegraphics[width=1\linewidth]{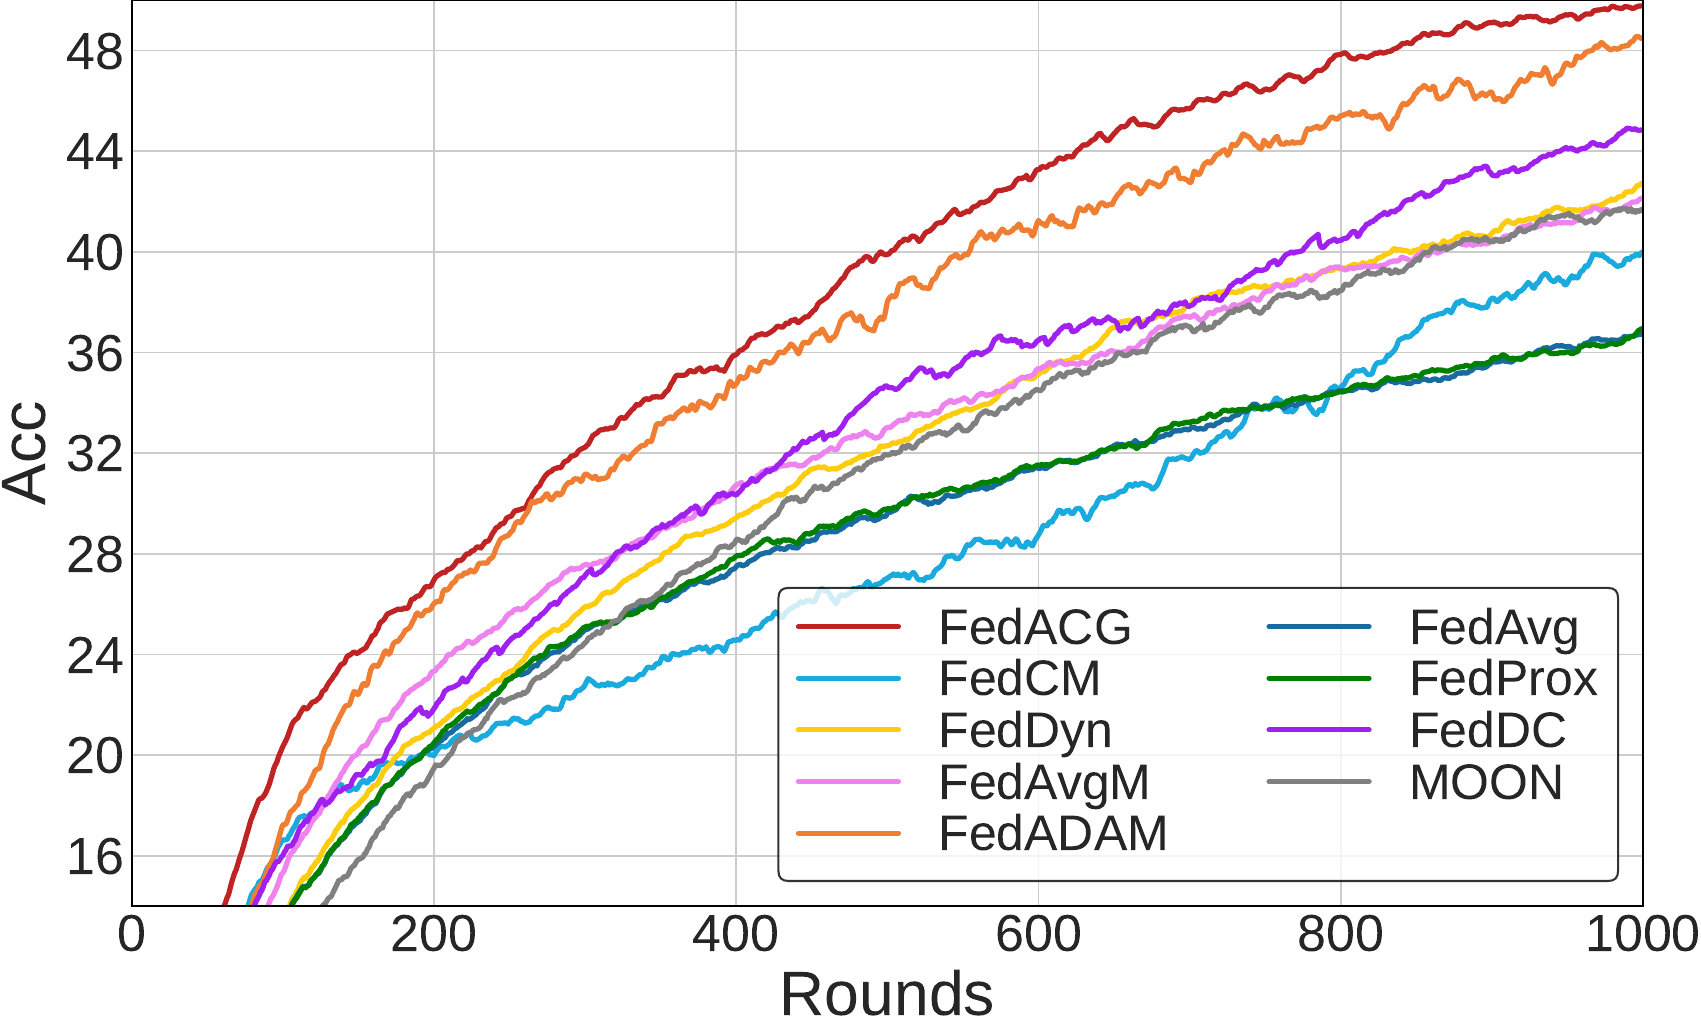}
%\vspace{-0.4cm}
\caption{Dirichlet (0.6), 500 clients, 2\% participation}
%\caption{1\% participation, 100 clients}
\end{subfigure}

\vspace{0.6cm}

\begin{subfigure}[b]{0.45\linewidth}
\centering
\includegraphics[width=1\linewidth]{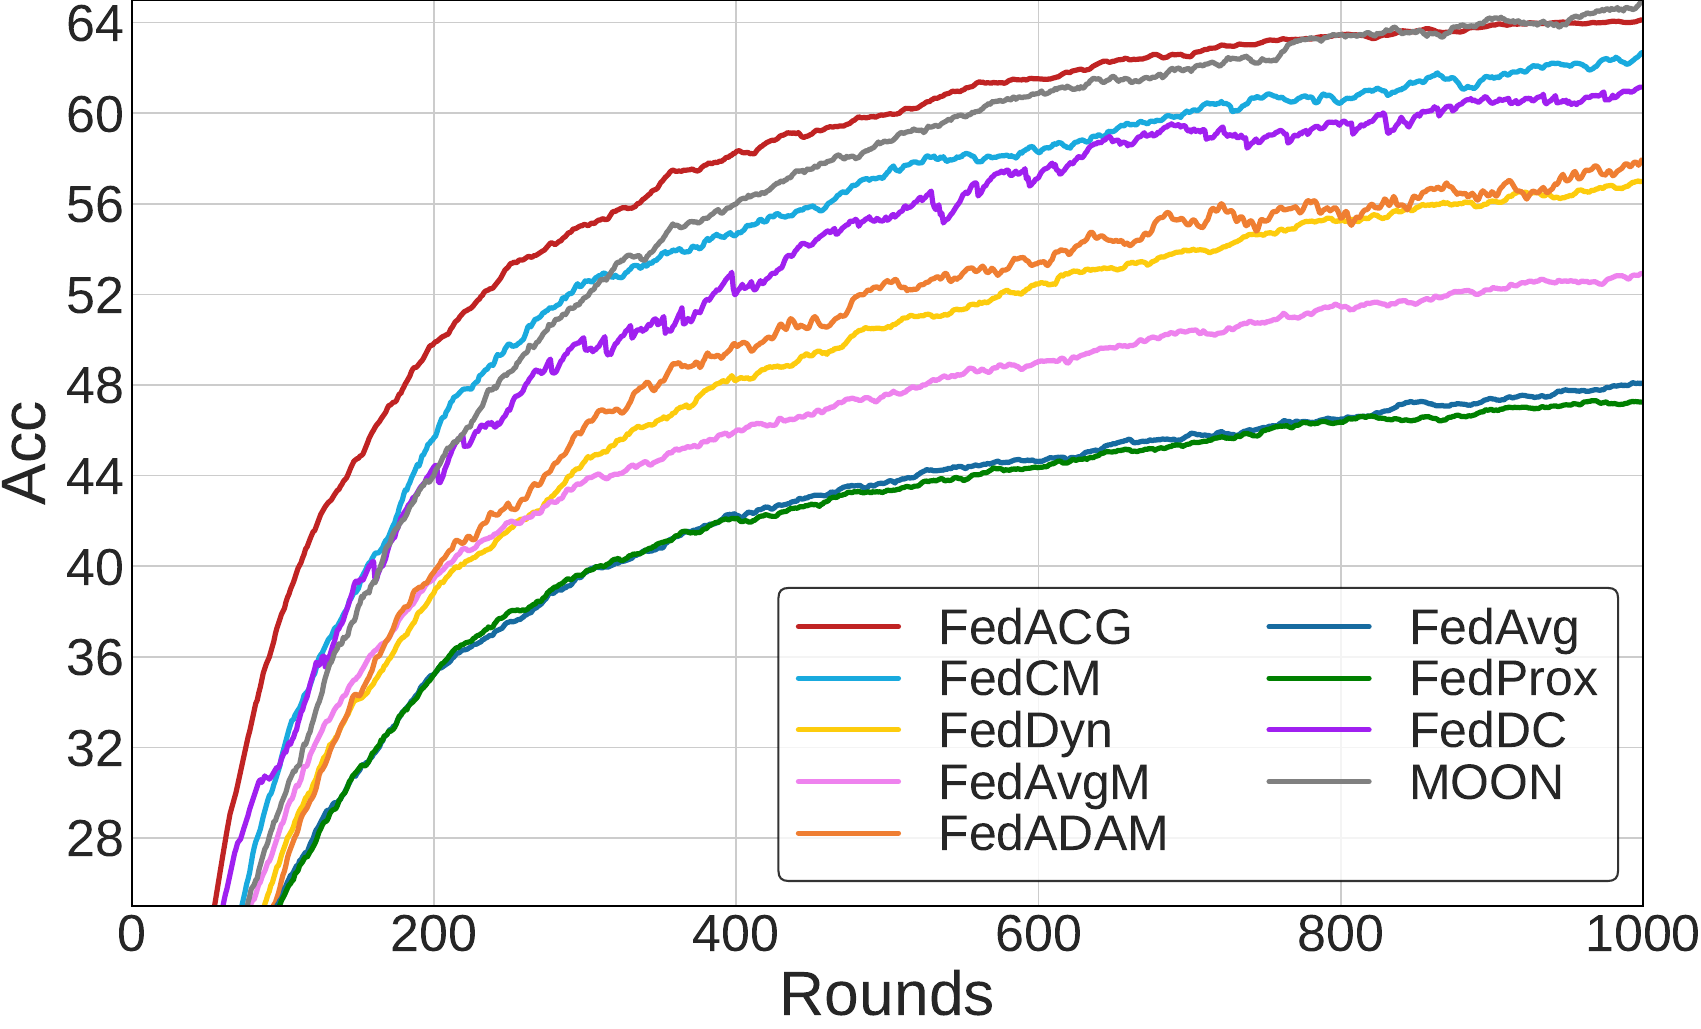}
%\vspace{-0.4cm}
\caption{\textit{i.i.d.}, 100 clients, 5\% participation}
\end{subfigure}
%\rulesep
\hspace{0.4cm}
\begin{subfigure}[b]{0.45\linewidth}
\centering
\includegraphics[width=1\linewidth]{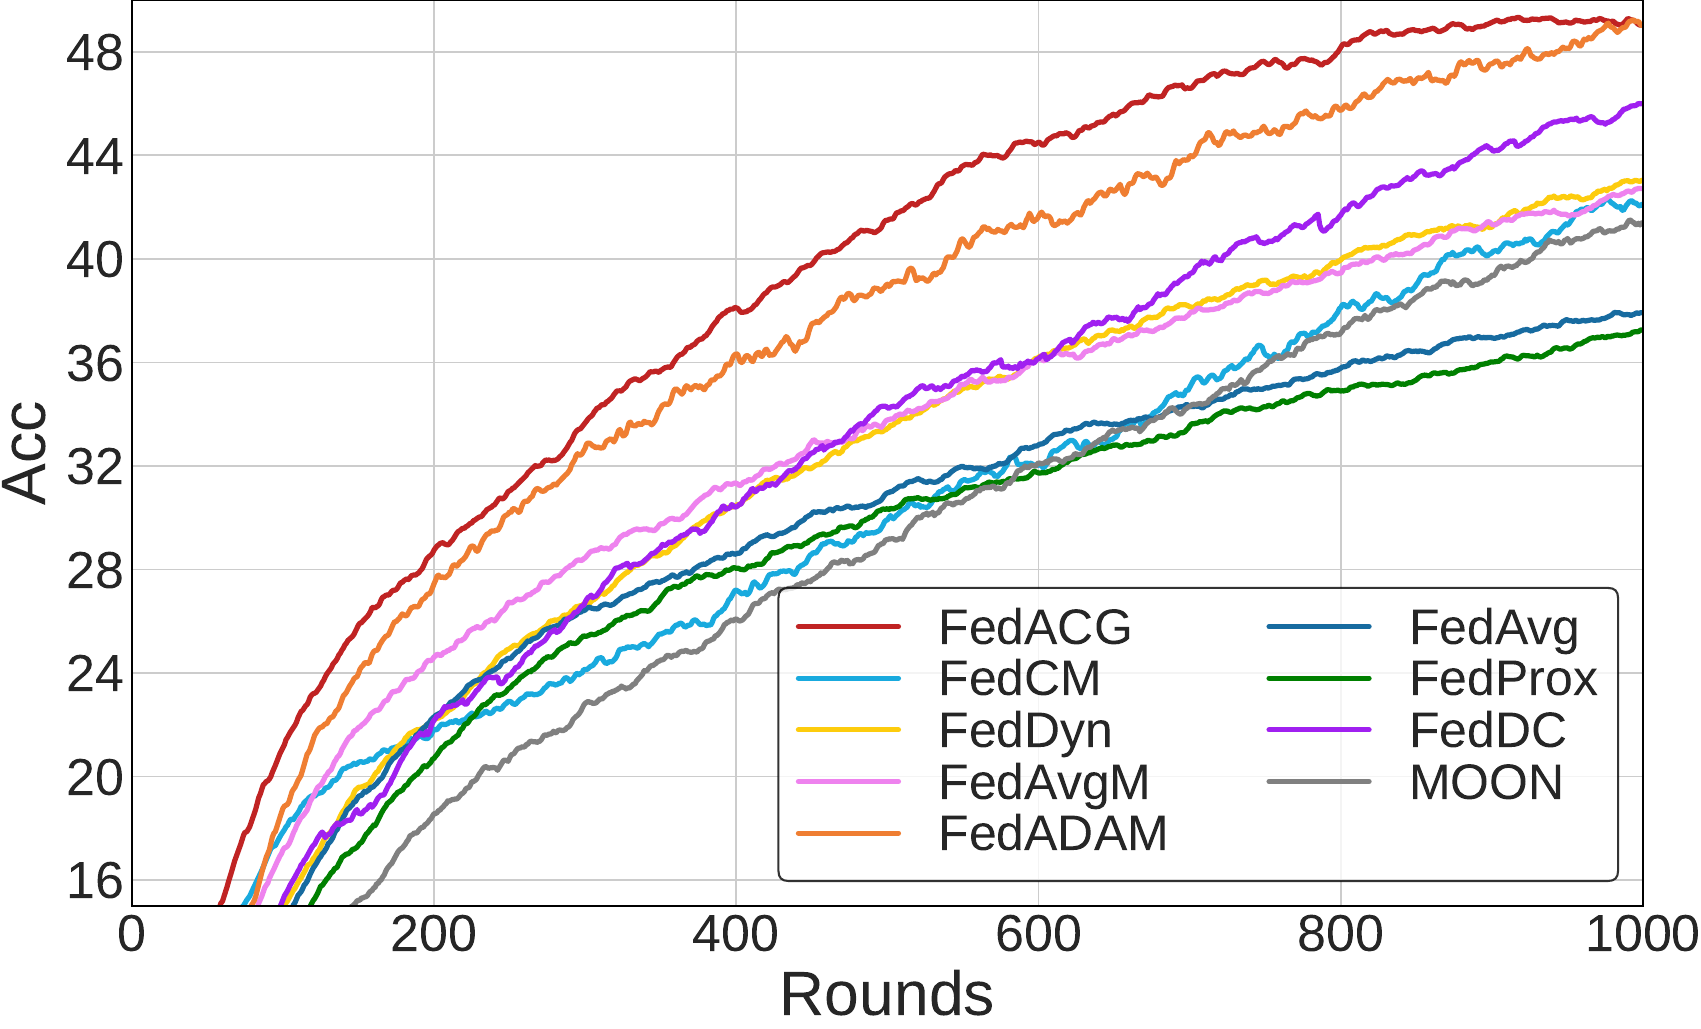}
%\vspace{-0.4cm}
\caption{\textit{i.i.d.}, 500 clients, 2\% participation}
%\caption{1\% participation, 100 clients}
\end{subfigure}
\caption{
The convergence plots of FedACG and the baselines on CIFAR-100 with different federated learning scenarios.
}
%\vspace{-0.8cm}
\label{fig:convergence_cifar100}
\end{figure}
%%%%%%%%%%%%%%%%%%%%%%%%%%%%%%%%%%%%%%%%%%%%%%%%%%%%%%%%%%%%%%%%%%%%%%%%%%%%%%%%%%%%%%%%%%%%%%%%%%%%%%%%%%%%%%%

%%%%%%%%%%%%%% Tiny-ImageNet %%%%%%%%%%%%%%%%%%%%%%%%%%%%%%%%%%%%%%%%%%%%%%%%%%%%%
\begin{figure}[h!]
\centering
\begin{subfigure}[b]{0.45\linewidth}
\centering
\includegraphics[width=1\linewidth]{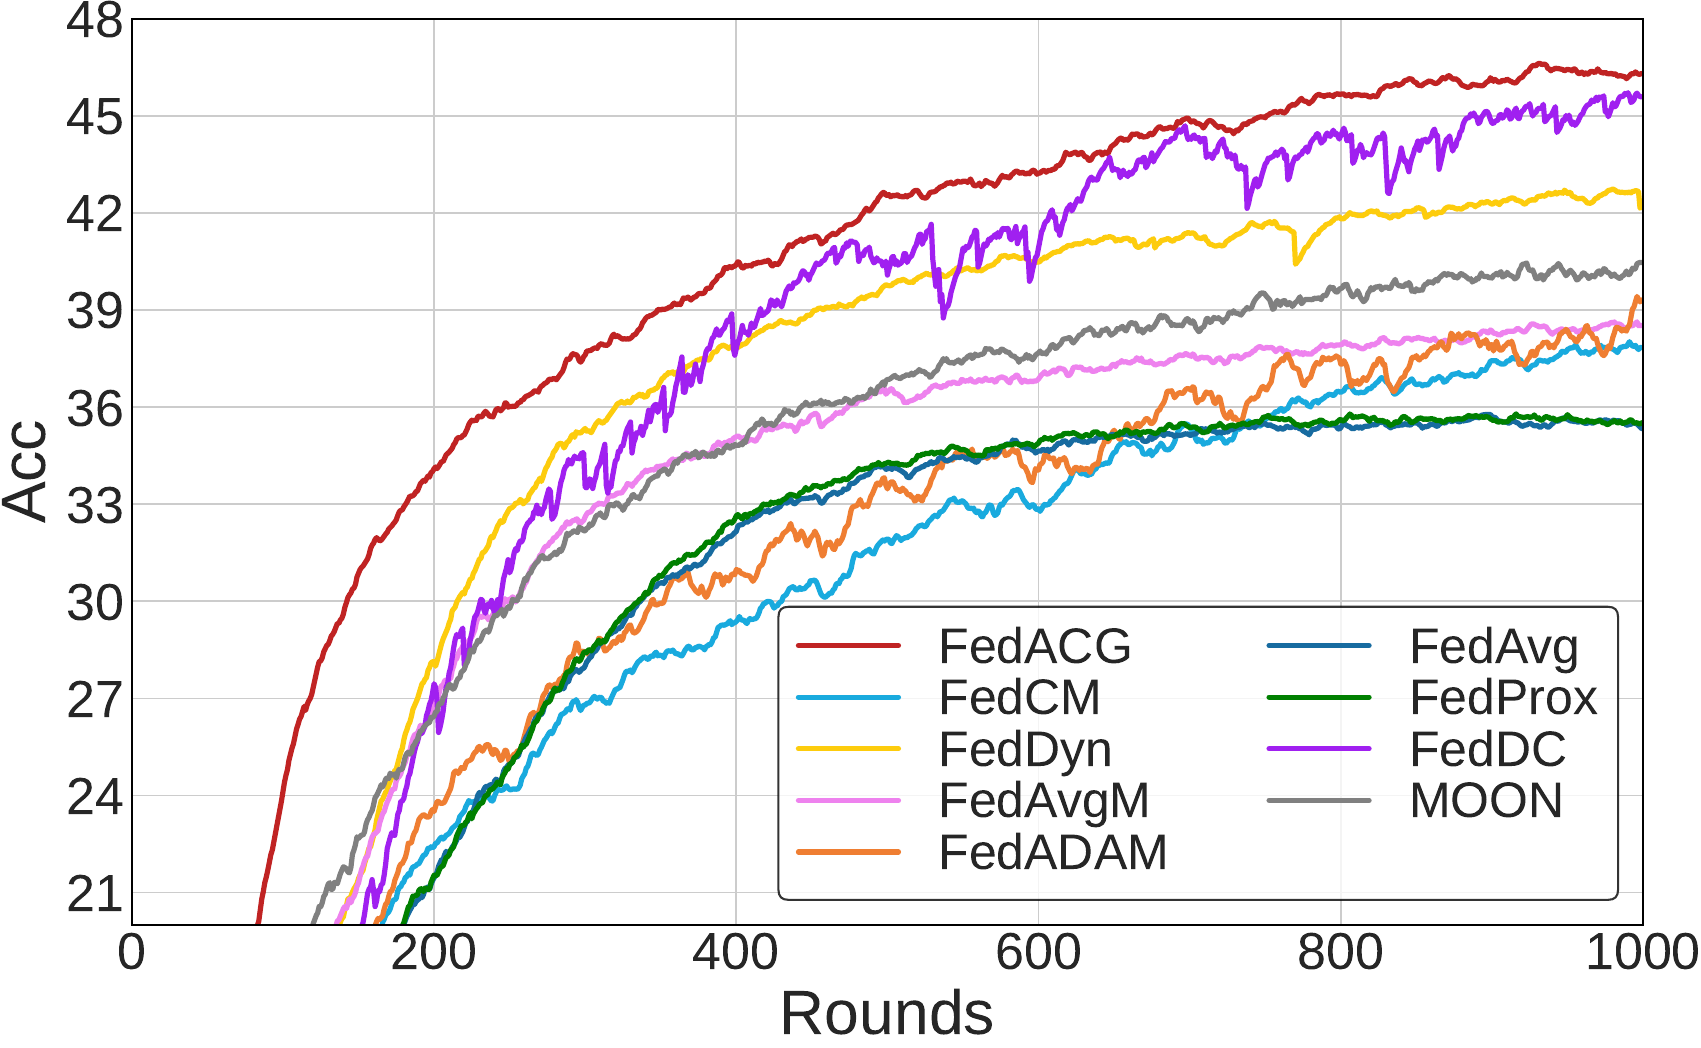}
%\includegraphics[width=1\linewidth]{figures/cifar100_mid_100.pdf}
%\vspace{-0.4cm}
\caption{Dirichlet (0.3), 100 clients, 5\% participation}
\end{subfigure}
%\rulesep
\hspace{0.4cm}
\begin{subfigure}[b]{0.45\linewidth}
\centering
\includegraphics[width=1\linewidth]{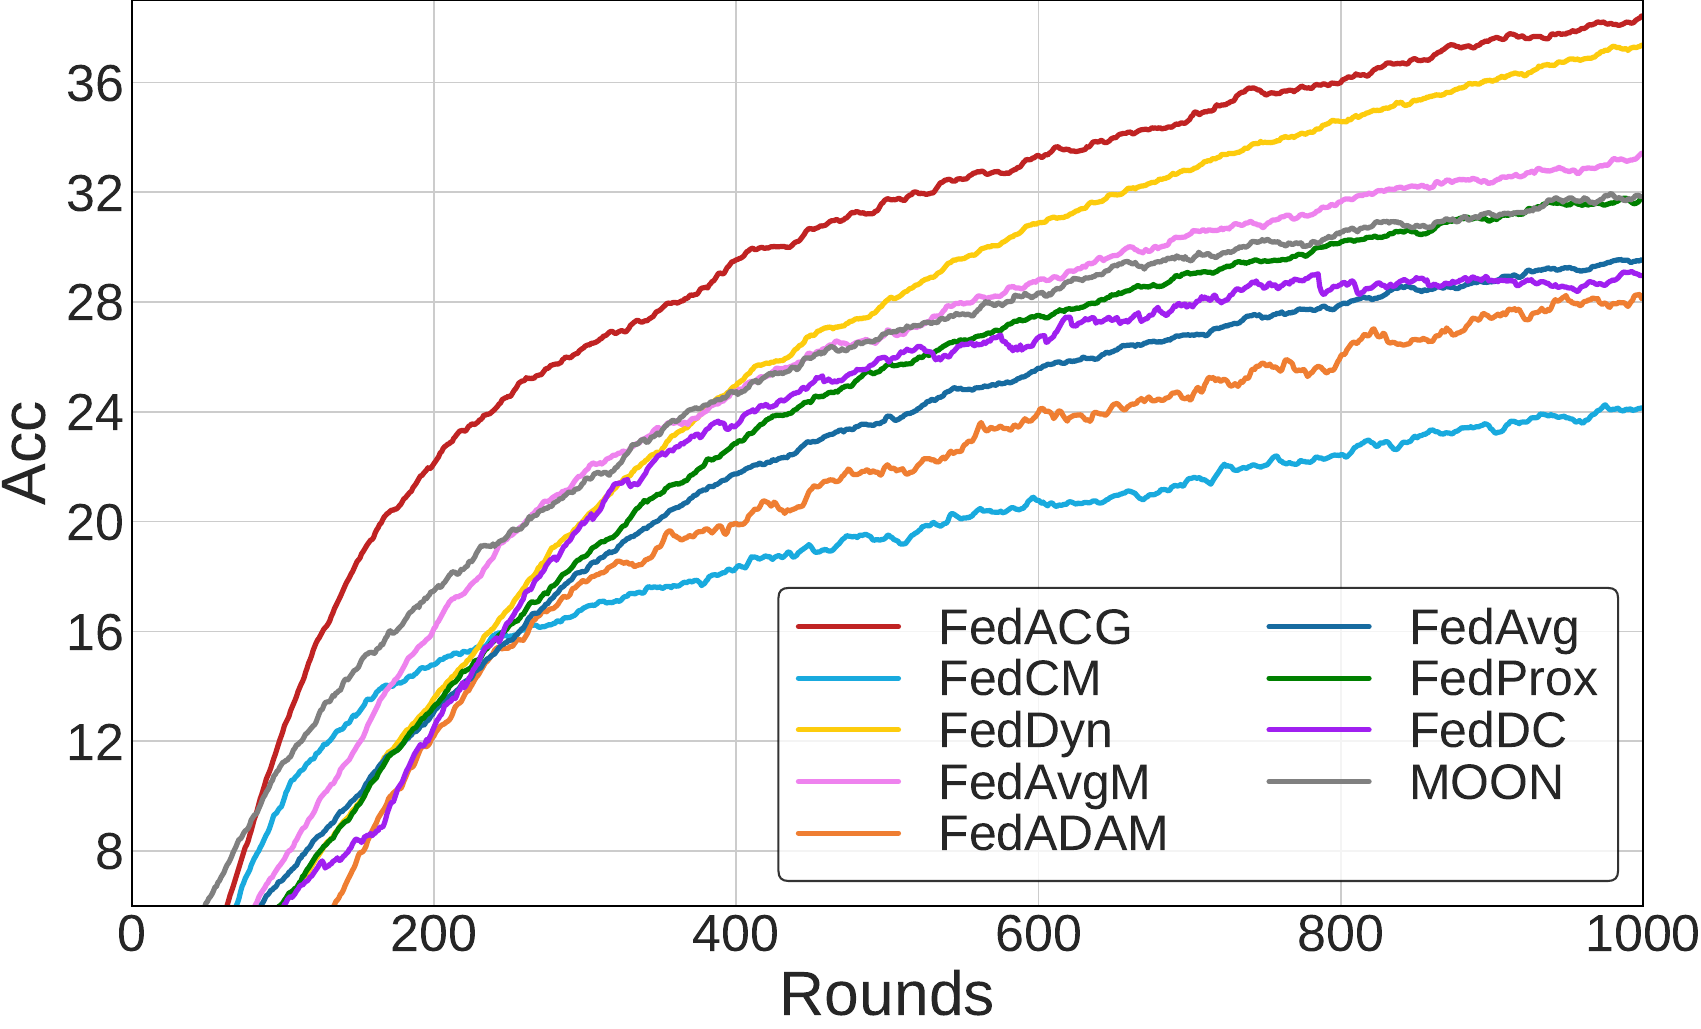}
%\includegraphics[width=1\linewidth]{figures/tiny_mid_100.pdf}
%\vspace{-0.4cm}
\caption{Dirichlet (0.3), 500 clients, 2\% participation}
%\caption{1\% participation, 100 clients}
\end{subfigure}

\caption{
The convergence plots of FedACG and the baselines on Tiny-ImageNet with different federated learning scenarios.
}
%\vspace{-0.8cm}
\label{fig:convergence_tiny}
\end{figure}
%%%%%%%%%%%%%%%%%%%%%%%%%%%%%%%%%%%%%%%%%%%%%%%%%%%%%%%%%%%%%%%%%%%%%%%%%%%%%%%%%%%%%%%%%%%%%%%%%%%%%%%%%%%%%%%

\clearpage

%%%%%%%%%%%%%%500 Clients 1% participation%%%%%%%%%%%%%%%%%%%%%%%%%%%%%%%%%%%%%%%%%%%%%%%%%%%%%%%%%%%%%%%%%%%%%%%%%%
\begin{figure}[t]
\centering
\begin{subfigure}[b]{0.45\linewidth}
\centering
\includegraphics[width=1\linewidth]{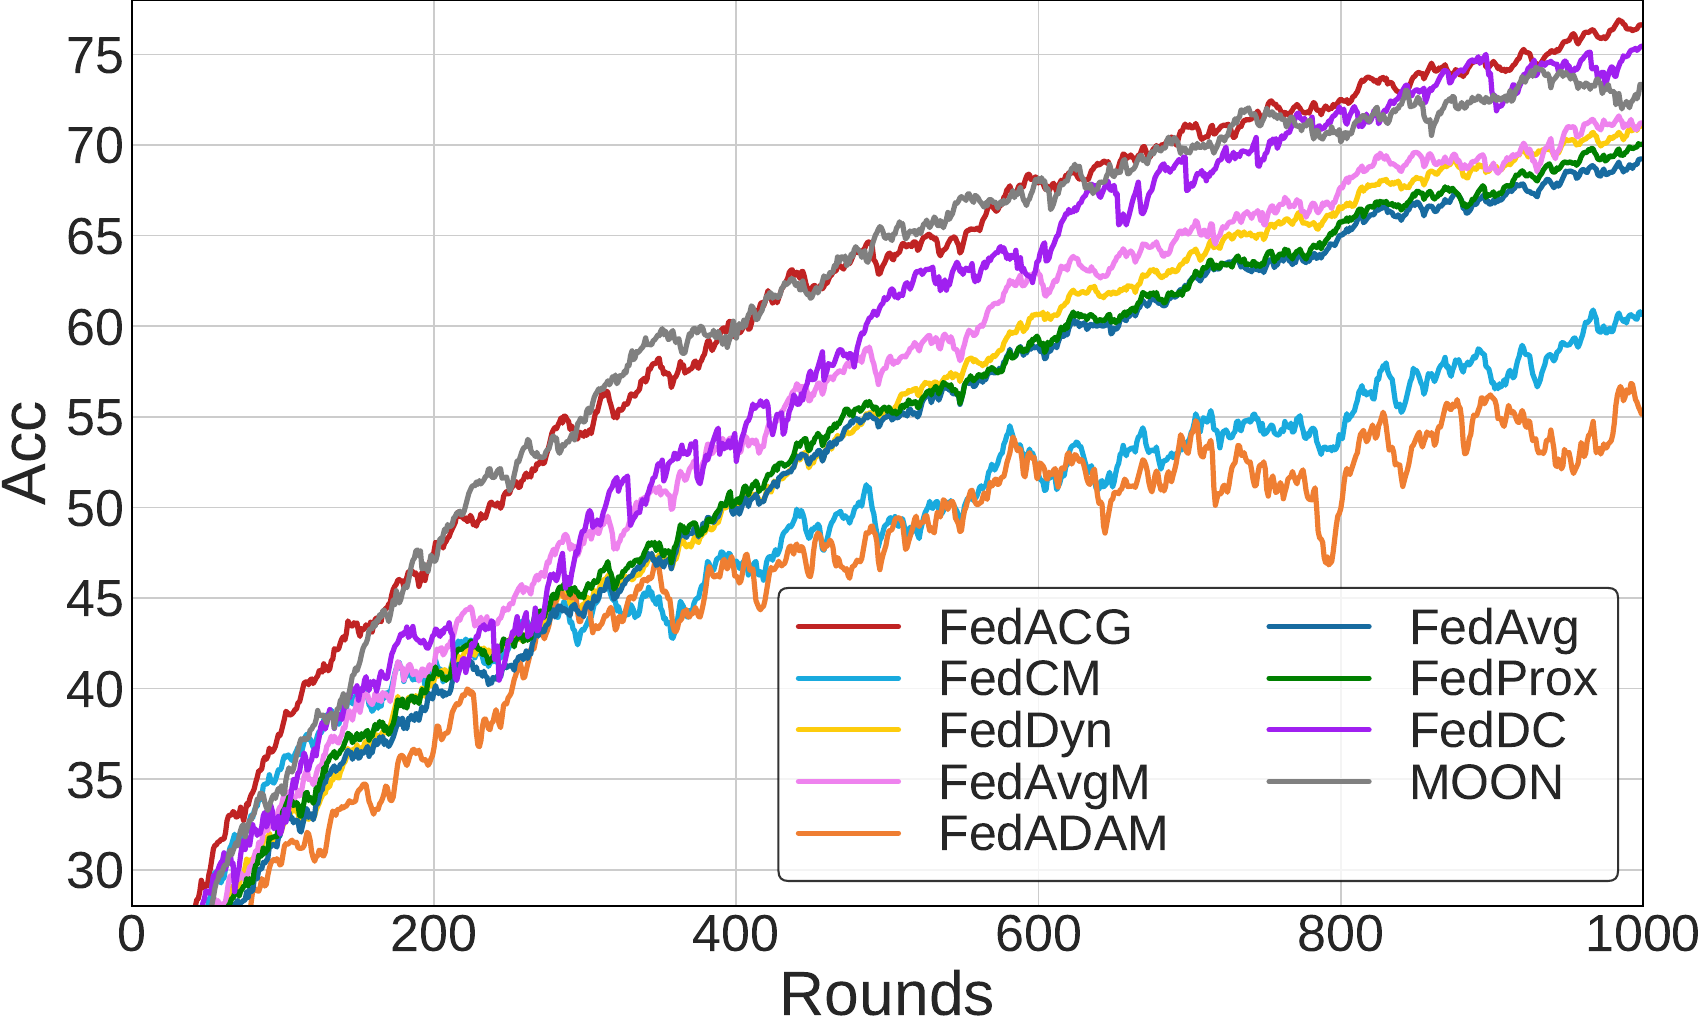}
%\includegraphics[width=1\linewidth]{figures/cifar100_mid_100.pdf}
%\vspace{-0.4cm}
\caption{CIFAR-10}
\end{subfigure}
%\rulesep
\hspace{0.4cm}
\begin{subfigure}[b]{0.45\linewidth}
\centering
\includegraphics[width=1\linewidth]{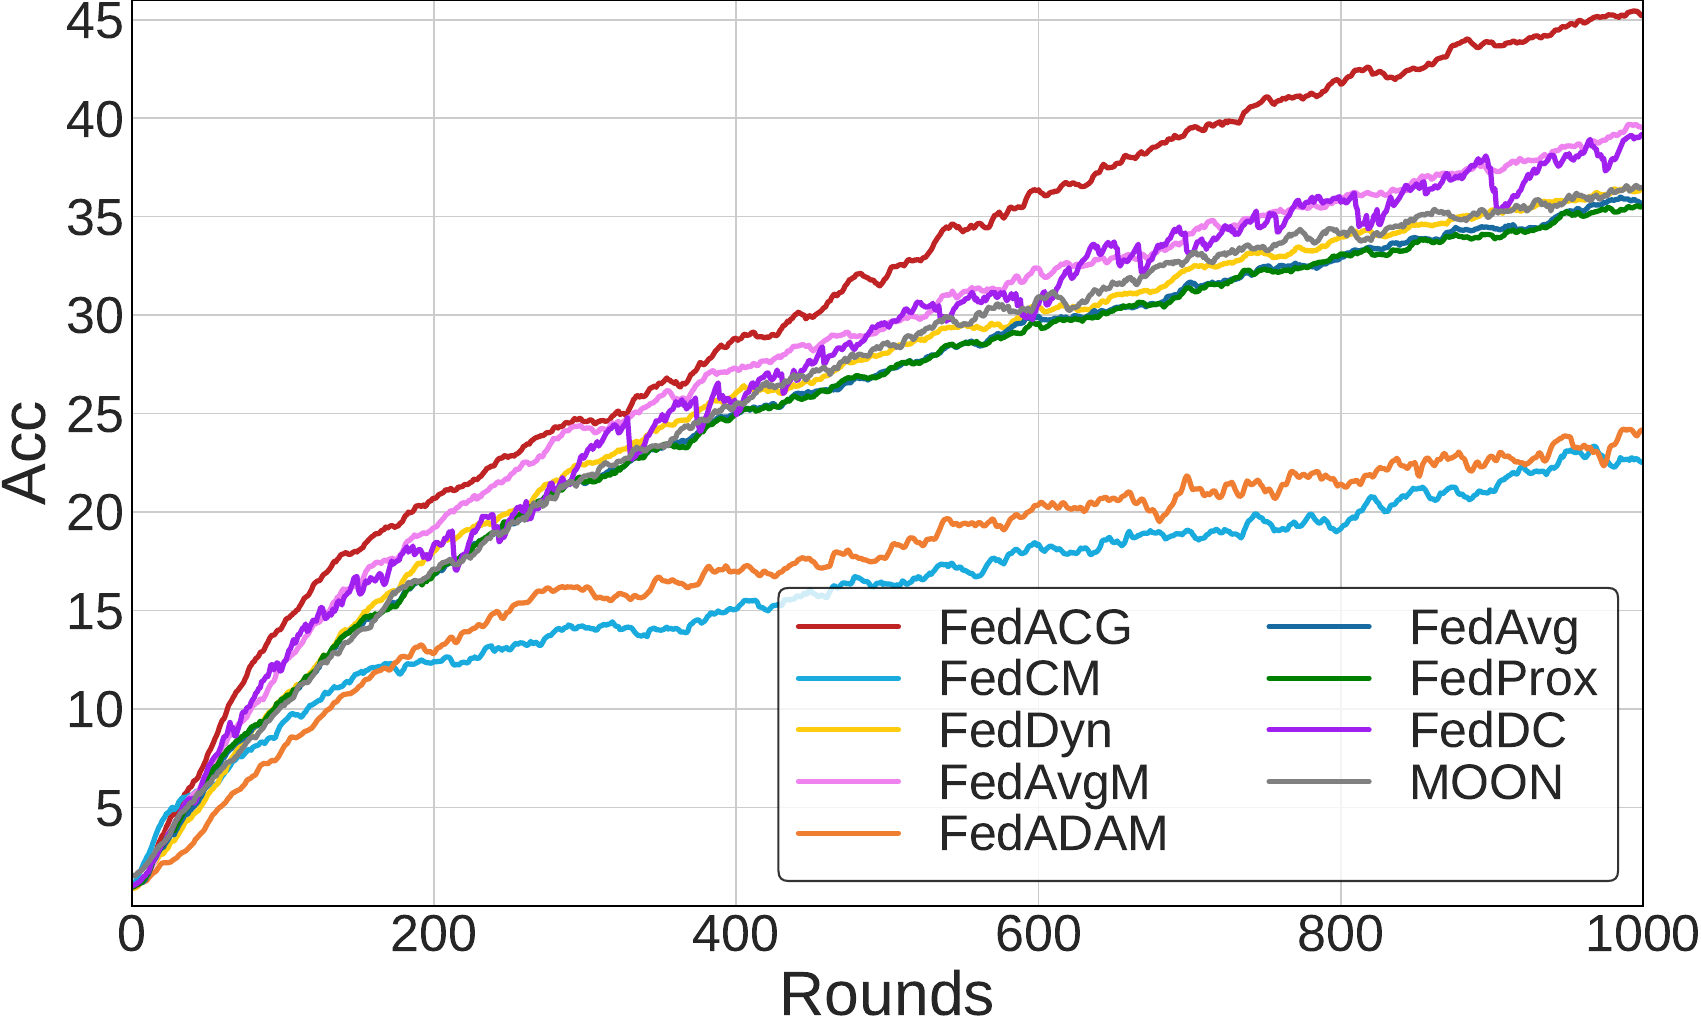}
%\includegraphics[width=1\linewidth]{figures/tiny_mid_100.pdf}
%\vspace{-0.4cm}
\caption{CIFAR-100}
%\caption{1\% participation, 100 clients}
\end{subfigure}
\caption{
The convergence plots of FedACG and the baselines when the participation rate is low (1\%) for 500 clients on CIFAR-10 and CIFAR-100. The Dirichlet parameter is set to $0.3$ for the experiments.
}
%\vspace{0.05cm}
\label{fig:cifar_d_03}
\end{figure}
%%%%%%%%%%%%%%%%%%%%%%%%%%%%%%%%%%%%%%%%%%%%%%%%%%%%%%%%%%%%%%%%%%%%%%%%%%%%%%%%%%%%%%%%%%%%%%%%%%%%%%%%%%%%%%%

\subsubsection{Evaluation on dynamic client set}
Figure~\ref{fig:incre_curve} shows a convergence plot when the entire client's pool changes during training. 
\iffalse
%The total number of clients is 1000, which is divided into 10 bundles of 100 clients. 
%The Dirichlet parameter is set to 0.3.
%For the experiment, 100 new clients out of 1000 clients are added every 100 rounds 
%we first construct 1000 clients, which is divided into 10 bundles.
%We then the number of clients in the clients pool that can participate in learning is initially set to 100, and 100 clients are added to the clients pool every 100 global rounds over 10 stages.
%Clients participating in each global round are determined by sampling 5\% clients from a pool of the entire clients that can participate in learning. 
\fi
The result shows that FedACG outperforms the baselines in most learning sections.
Note that FedDyn shows worse performance than FedAvg in the overall section of learning, and only achieves FedAvg's performance at the end.
%This is partly because the local states required by FedDyn require a kind of warm-up period to contain useful information.
This is partly because it needs to store local states for local training in each client, which requires a kind of warm-up period for newly participating clients to contain useful information.
In contrast, FedACG, which is free from these restrictions, shows strength in a realistic federated learning scenario where the pool of entire clients changes during training.

%%%%%%%%%%%%%%%%%%%%%% Incremental learning scenario %%%%%%%%%%%%%%%%%%%%%%%%%%%%%%%%%%%%%%%%%%%%%%%%%%%%%%%%%%
\begin{figure*}[h!]
\centering
\begin{subfigure}[b]{0.45\linewidth}
\centering
\includegraphics[width=1\linewidth]{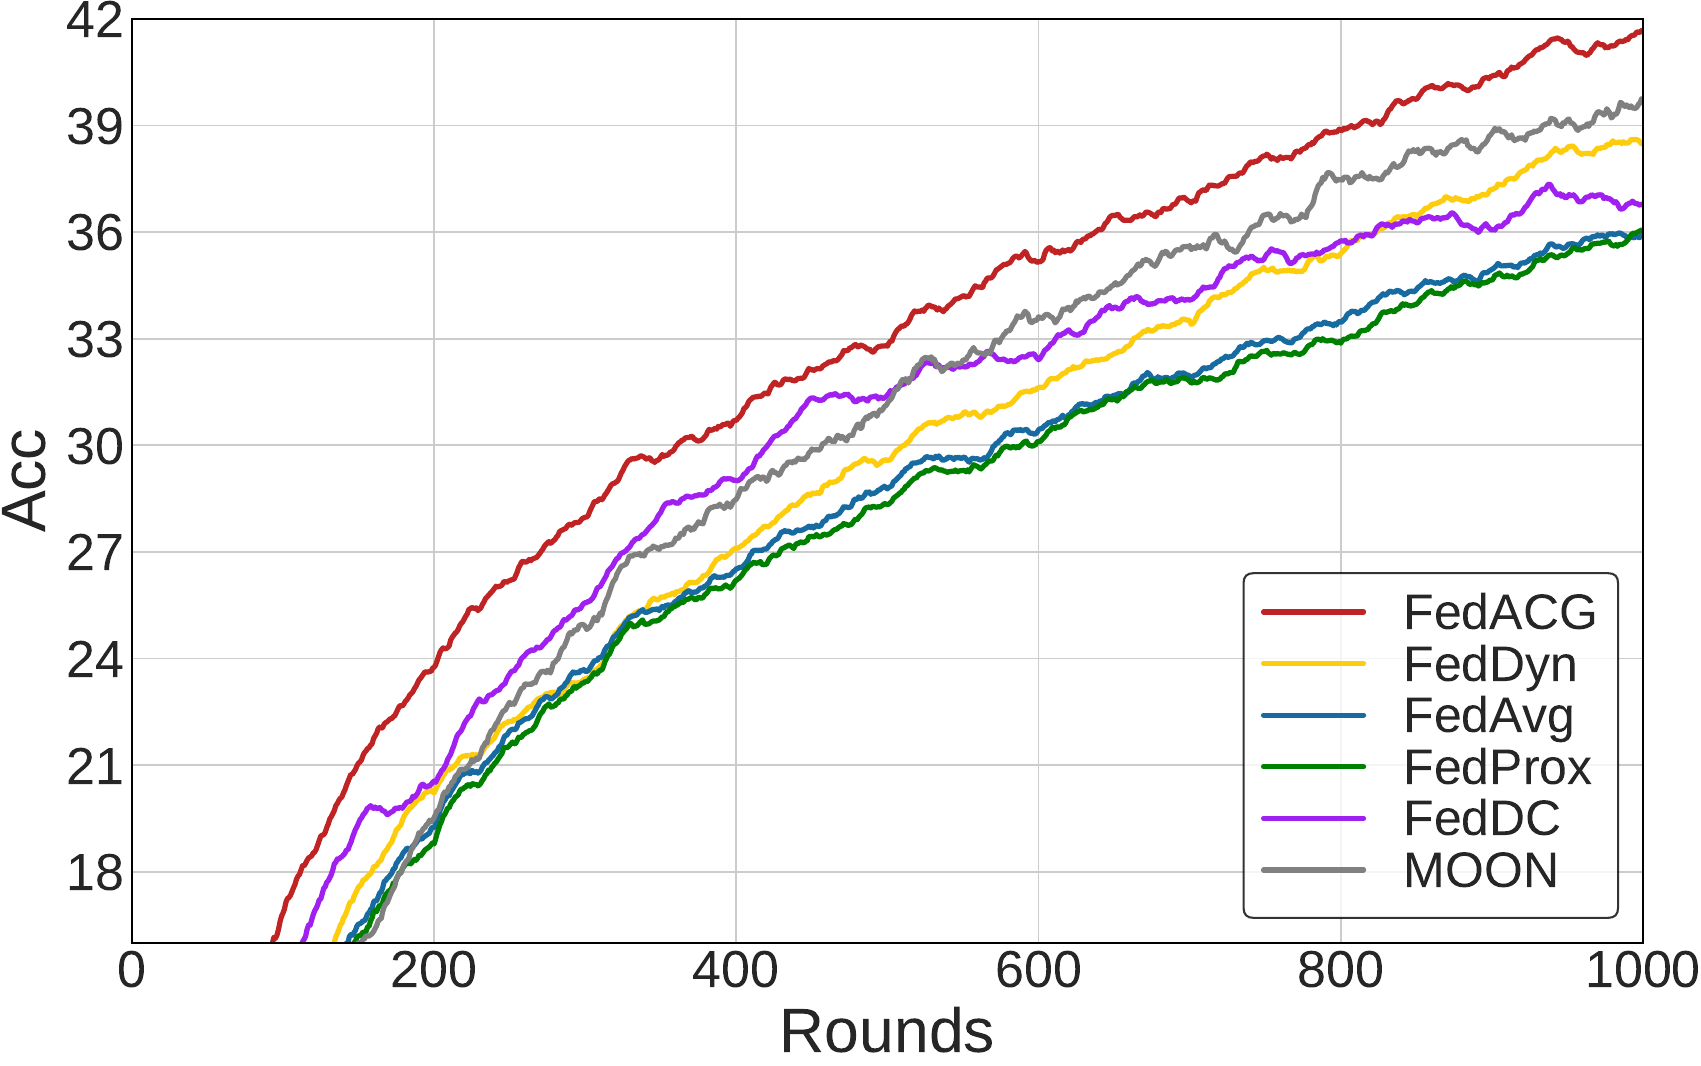}
%\vspace{-0.4cm}
%\caption{10\%}
\end{subfigure}
%\rulesep
\caption{
The convergence plots of FedACG, FedAvg, FedDyn, FedDC, and MOON on CIFAR-100 when the client set changes over dynamically: we sample 250 clients out of 500 clients as a candidate clients set at every 100 rounds over 10 stages on Dirichlet (0.3) split.
10 clients out of the sampled client set participate for the local training for each communication round. Dirichlet parameter is set to $0.3$.
}
%\vspace{-0.7cm}
\label{fig:incre_curve}
\end{figure*}

\subsection{Integration of FedACG with quantization techniques.}

To validate that FedACG algorithm can be integrated into quantization-based techniques,
we have conducted an experiment combining FedACG with FedPAQ~\citep{reisizadeh2020fedpaq}, one of the quantization methods in federated learning, on the CIFAR-100, using 8 bits for quantization. 
Table~\ref{tab:fedpaq} shows that our method works well even with quantization methods, surpassing both FedPAQ and FedAvg without quantization.

\begin{table}[h]
    \centering
    \caption{Accuracy of FedACG with the integration of FedPAQ at the 1K round on CIFAR-100.}
    \begin{tabular}{lcc}
        \toprule
        Method & \multicolumn{1}{c}{100 clients (5\% participation)} & \multicolumn{1}{c}{500 clients (2\% participation)} \\
        \midrule
        FedAvg & 47.83 & 38.11 \\
        FedPAQ & 41.99 & 30.21 \\
        FedACG + FedPAQ & \textbf{50.53} & \textbf{39.55} \\
        \bottomrule
    \end{tabular}
    \label{tab:fedpaq}
\end{table}

{\section{FedACG vs. FedAvgM and FedProx}}
\paragraph{FedAvgM~\citep{hsu2019measuring}}
The unique characteristic of FedACG lies in the initialization of client models. Although FedACG and FedAvgM use global momentum in common, FedACG broadcasts the accelerated global model by adding global momentum to the current global model ($\theta^{t-1} + \lambda m^{t-1}$) while FedAvgM broadcasts the current global model ($\theta^{t-1}$) to each client as the initial point of the local model.
Figure~\ref{fig:twostep} illustrates the difference in the server broadcasting and aggregation process of FedACG and FedAvgM, respectively.
Unlike FedAvgM, where the only server knows the global momentum, in FedACG, the clients, the actual learners, start their local training at the anticipated point $\theta^{t-1} + \lambda m^{t-1}$ and can make up for the previous global momentum $\lambda m^{t-1}$ through their local training. 
This difference in the initial point seems to allow FedACG to be trained more responsive way, letting it behave more stably than FedAvgM in many federated learning settings. 

\begin{figure}[h]
\centering
     \begin{subfigure}[b]{1.0\textwidth}
         \centering
         \includegraphics[width=0.768\textwidth]{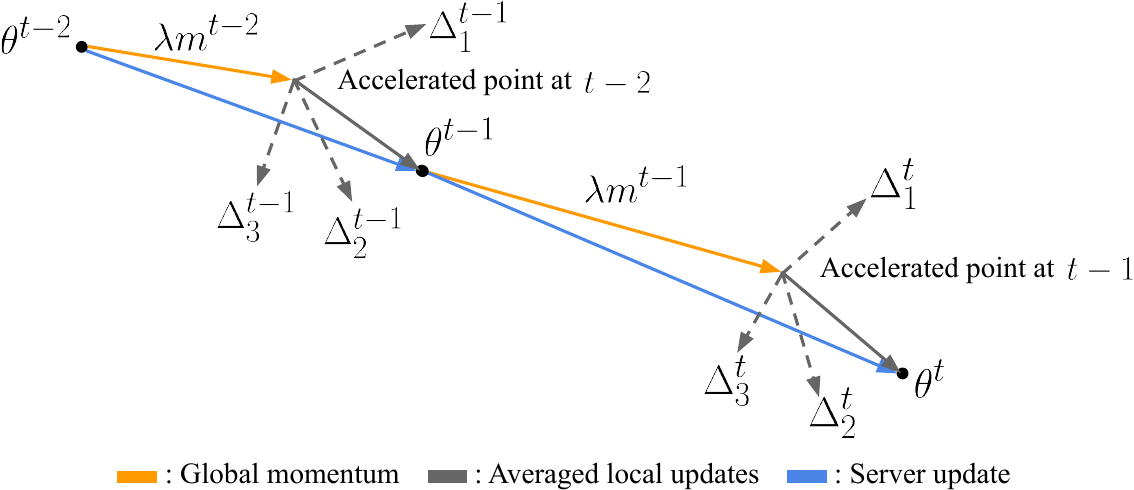}
         \caption{FedACG}
     \end{subfigure}
\centering
     \begin{subfigure}[b]{1.0\textwidth}
         \centering
         \includegraphics[width=0.6\textwidth]{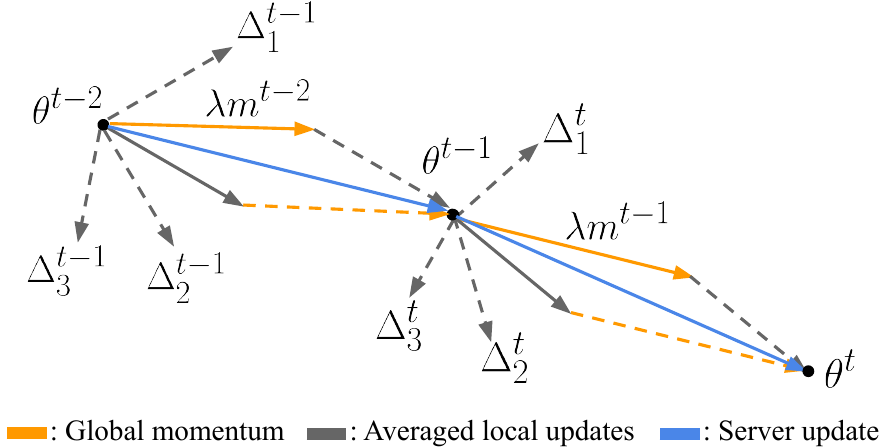}
         \caption{FedAvgM}
     \end{subfigure}
\caption{An illustration of the FedACG and FedAvgM during two communication rounds.}
\label{fig:twostep}
\end{figure}
%
\iffalse
%
\begin{figure}[h]
\centering
\includegraphics[width=0.6\textwidth]{figures/fedavgm_twostep.pdf}
\caption{An illustration of the FedAvgM during two communication rounds}
\label{fig:FedAvgM_twostep}
\end{figure}
%
\fi

\iffalse
\begin{table}[h!]
    \captionof{table}{Effect of local regularization term on different federtaed learning algorithms on CIFAR-10 and CIFAR-100 with 2\% participation and 500 clients.}
    %Ablation study on the components of FedACG on CIFAR-10 for the large-scale federated learning setting. The Dirichlet parameter used in the experiment is 0.3.}
    \label{tab:acceleration_ablation}
\begin{center}
    \scalebox{0.85}{
    \setlength\tabcolsep{5pt}
    \hspace{-0.2cm}
    \begin{tabular}{cccc || cc}
		%\hline
		\makecell{Method}&\makecell{Server update \\ w momentum} &\makecell{Accelerated client gradient} & \makecell{Local regularization} & CIFAR-10 & CIFAR-100 \\
		\hline
          FedAvg&&&  & 71.45 & 38.11  \\ %\hdashline
          FedProx&&& \checkmark &  70.75 & 36.16\\ %\hdashline
          FedAvgM&\checkmark&&  & 77.49 & 40.54  \\ %\hdashline
          FedAvgM w local reg&\checkmark&& \checkmark &  76.16 & 41.64\\ %\hdashline
          FedACG w/o local reg&\checkmark&\checkmark &  & 82.20  & 46.80\\ %\hdashline
          FedACG&\checkmark&\checkmark & \checkmark & \textbf{82.80}  & \textbf{48.40}  \\
        \hline                                     
	\end{tabular}
    }
\end{center}
%\vspace{-0.4cm}
\end{table}
\fi

\paragraph{FedProx~\citep{li2018federated}}
FedACG is a different method from FedProx for three principal reasons. First, FedACG utilizes the global momentum for server updates. 
Second, since FedACG uses client accelerated gradient, the local model's initial point is different from FedProx. 
From this, the third, objective function of FedACG regularizes the distance not between the local model and the previous global model (FedProx), but between the local model and the accelerated point.

\section{Convergence of FedACG}
\label{sec:convergence_proof}
We now present the theoretical convergence rate of FedACG.
We first state a few assumptions for the local loss functions $\mathcal{F}_i(\theta)$, which are commonly used in several previous works on federated
optimization~\citep{karimireddy2019scaffold,reddi2021adaptive,xu2021fedcm}.
First, the local function $\mathcal{F}_i(\cdot)$ is assumed to be $L$-smooth for all $i \in \{1,\dots,N\}$, \ie
\begin{align}
\|\nabla \mathcal{F}_i ({x}) -\nabla \mathcal{F}_i ({ y})\|\leq
L \|{ x} - { y}\|\ \ \forall { x}, { y}. 
\end{align}
if local functions $\{\mathcal{F}_i(\cdot)\}_{i=1}^N$ are convex, we additionally have
\begin{align}
& \forall { x}, \ \ \ \ \ \ \  \frac{1}{2LN}\sum_{i=1}^{N} \|\nabla \mathcal{F}_i ({x}) - \nabla \mathcal{F}_i({x}_*)\|^2 \leq \mathcal{F}({x})-\mathcal{F}({x}_*) ~~\text{and}
\label{as:smooth_convex_min}\\
& \forall { x}, { y}, { z}, \  \left\langle \nabla \mathcal{F}_i ({ x}), { z}- { y}\right\rangle \leq -\mathcal{F}_i({ z}) +\mathcal{F}_i({ y}) + \frac{L}{2} \|{ z} - { x}\|^2 ,
\label{as:smooth_convex_grad}
\end{align}
where $\mathcal{F}({ x}) = \frac{1}{N} \sum_{i=1}^N \mathcal{F}_i({ x})$ and $\nabla \mathcal{F}({ x}_*)={ 0}$.
Second, we assume the stochastic gradient of the local loss function $\nabla {f}_i(x) :=  \nabla \mathcal{F}_i(x; \mathcal{D}_i)$ is unbiased and possesses a bounded variance,~\ie $\mathbb{E}_{\mathcal{D}_i} \| \nabla f_i ({ x}) - \nabla \mathcal{F}_i(x) \| < \sigma^{2}$. Third, we assume the average norm of local gradients is bounded by a function of the global gradient magnitude as $\frac{1}{N} \sum_{i=1}^N\left\|\nabla \mathcal{F}_i(x)\right\|^2 \leq \sigma _{g}^2+B^2\|\nabla \mathcal{F}(x)\|^2$, where $\sigma_g \geq 0$ and $B \geq 1$.
% Second, we assume the local loss functions $\mathcal{F}_i({ x})$ have bounded variance,~\ie $\mathbb{E}_{\mathcal{D}_i} \| \nabla f_i ({ x}) - \nabla \mathcal{F}_i(x) \| < \sigma^{2}$ for all $x$.
% We adopt the bounded gradient dissimilarity assumption given by $\frac{1}{N} \sum_{i=1}^N\left\|\nabla \mathcal{F}_i(x)\right\|^2 \leq {\sigma _{g}}^2+B^2\|\nabla \mathcal{F}(x)\|^2$ to take account for data heterogeneity between clients.
%We assume that the local loss functions $\mathcal{L}_i({x})$ have bounded gradients, $\| \nabla \mathcal{L}_i({x}) \|<G \ \ \forall { x}$.
Based on the above assumptions, we derive the following asymptotic convergence bound of FedACG.
%Note that we make no further assumptions such as a form of bounded variance and gradients used in~\citet{karimireddy2019scaffold}, \citet{reddi2021adaptive}, and \citet{xu2021fedcm}.

\iffalse
\paragraph{Definition}
$\Delta^t_i =\theta_{i}^{t}-(\theta^{t-1} + \lambda m^{t-1}) =\sum_{k=0}^{K-1}-\eta\nabla f_{i}(\theta^{t}_{i,k})$.

$\Delta^t = \frac{1}{|\mathcal{S}_t|}\sum_{i \in \mathcal{S}_t}\Delta^t_i = 
\frac{1}{|\mathcal{S}_t|}\sum_{i \in \mathcal{S}_t}\sum_{k=0}^{K-1}-\eta\nabla f_{i}(\theta^{t}_{i,k})$.

$\delta^t = \frac{1}{N}\sum_{i \in [N]}\sum_{k=0}^{K-1}-\eta\nabla \mathcal{F}_{i}(\theta^{t}_{i,k})$.

$e^t =\Delta^t - \delta^t$.
Note that $\mathbb E[e^t] = 0$

$z^t = \theta^t + \frac{\lambda}{1 - \lambda} m^t$.
\fi

\subsection{Convergence of FedACG for non-convex functions}

\begin{theorem}\label{thm:1}
(Convergence of FedACG for non-convex functions) Suppose that local functions $  \lbrace \mathcal {F}_i \rbrace _{i=1}^{N}$ are non-convex and $L$-smooth.
Let $z^t = \theta^t + \frac{\lambda}{1 - \lambda} m^t$.
Then, by setting $\eta \leq \frac{1-\lambda}{100KL(B^2+1)}$, FedACG satisfies,
\begin{equation}
    \begin{aligned}
\min_{t=1, \ldots, T} \mathbb{E}\left\|\nabla \mathcal{F}\left(\theta^{t-1} + \lambda m^{t-1}\right)\right\|^2
& \leq 1000(B^2+1)\frac{Ld_0}{T}+ \sqrt {\frac{40 Ld_0}{T} \bigg(\psi_1  \sigma^2  + \psi_2 \sigma_g^2    \bigg) } \\
& \quad + \frac{1}{T^{\frac{2}{3}}}\left[800 L^{2}d_0^{2} \right. \left. A\left(\psi_3 \sigma^{2}+ \psi_4 \sigma_g^{2}\right)\right]^{\frac{1}{3}},\\
% \min_{t=0, \ldots, T-1} \mathbb{E}\left\|\nabla \mathcal{F}\left(\theta^t + \lambda m^t\right)\right\|^2 
% & \leq 1000(B^2+1)\frac{Ld_0}{T}+ \sqrt {\frac{40 Ld_0}{T} \bigg(C_1  \sigma^2  + C_2 \sigma_g^2    \bigg) } \\
% & + \frac{1}{T^{\frac{2}{3}}}\left[800 L^{2}d_0^{2} \right. \left. A\left(C_3 \sigma^{2}+ C_4 \sigma_g^{2}\right)\right]^{\frac{1}{3}},\\
%C_1 = AC_1 + C_2
%C_2 = AC_3 + C_4
    \end{aligned}
\end{equation}
where $d_0=\mathcal{F}(z^0)-\mathcal{F}(z^*) $, $A=1+\frac{4N}{(N-1)|S_t|}(1-\frac{|S_t|}{N})$, $\psi_1 = A(\frac{1-\lambda}{K} + \frac{1}{K})+ \frac{5}{2} + (1-\lambda)(\frac{5}{K}+2)$, $\psi_2 =A((1-\lambda)^2 + 4 ) + 10(1-\lambda)  $, $\psi_3 =\frac{1-\lambda}{20K}$, and $\psi_4 =\frac{(1-\lambda)^2}{10}$.
\begin{proof}
We start the proof from the result in~\cref{lem:converge_nonconvex},
\begin{align*}
\mathbb{E}\big[\mathcal{F}\left(z^{T}\right)-\mathcal{F}\left(z^{0}\right)\big] & \leq T \textrm{C}_8 \sigma^{2}+T \textrm{C}_{9} \sigma_g^{2}+\textrm{C}_{10} \sum_{t=1}^{T} \mathbb{E}\|\nabla \mathcal{F}\left(\theta_{0}^{t}\right)\|^{2}
\end{align*}
where $\textrm{C}_{8} \leq \left(\frac{\eta k}{1-\lambda}\right)^{2} L\left[(\frac{5}{2}+ (1-\lambda)(\frac{5}{K} + 2)) + \frac{1}{K}\left\{(1-\lambda) + 1 + \frac{\eta K L }{20}\right\}A \right]$, $\textrm{C}_{9}\leq (\frac{\eta K}{1-\lambda})^2 L\left[ 10(1-\lambda) +  \frac{\eta K}{1-\lambda}\frac{1-\lambda}{10}LA +  A\left((1-\lambda^2) +4 \right) \right]$, and $\textrm{C}_{10} \leq -\frac{\eta k}{10(1-\lambda)}$, respectively.

By rewriting the above inequalities,

% By summing the above inequalities for $t = 0,\dots,T$ and by noting that $\lambda < \frac{1-\lambda}{LK}$, 
\begin{align*}
\frac{1}{10} \frac{\eta K}{1-\lambda} \sum_{t=1}^T \mathbb{E}\|\nabla \mathcal{F}\left(\theta_0^t\right)\|^2 & \leq -\textrm{C}_{10} \sum_{t=1}^T \mathbb{E}\|\nabla \mathcal{F}\left(\theta_0^t\right)\|^2\\
&\leq \mathbb{E}[\mathcal{F}(z^0) - \mathcal{F}(z^*)] +T \textrm{C}_{8} \sigma^2+T \textrm{C}_{9} \sigma_g^2
\end{align*}
Then 
$$
\begin{aligned}
\frac{1}{T} \sum_{t=1}^T\mathbb{E}\|\nabla \mathcal{F}\left(\theta_0^t\right)\|^2  & \leq \frac{1-\lambda}{\eta K} \frac{10}{T} \left(\mathcal{F}\left(z^{0}\right)-\mathcal{F}\left(z^{*}\right)\right)  +\frac{1-\lambda}{\eta K} \textrm{C}_{8} \sigma^2+\frac{1-\lambda}{\eta K} \textrm{C}_{9} \sigma_g^2 \\
& \leq \frac{1-\lambda}{\eta } \frac{10}{T} \left(\mathcal{F}\left(z^{0}\right)-\mathcal{F}\left(z^{*}\right)\right) + \left(\frac{\eta K L}{1-\lambda}\right)\left[\left(\frac{5}{2}+(1-\lambda)\left(\frac{5}{K}+2\right)\right)\right. \\
& \quad +\left . \left(\frac{1 + (1-\lambda)}{K}\right) A \right]\sigma^2 
+ \eta^{2} \left(\frac{K L}{1-\lambda}\right)^{2} \frac{1-\lambda}{ 20 K } A \sigma^2 \\
& \quad +  \frac{\eta K L}{1-\lambda} \left[10(1-\lambda) + A \big(\left( 1-\lambda \right)^2 + 4 \big) \right] \sigma_g^2 
+   \frac{\eta^2 K^2 L^2}{10} A \sigma_g^2 \\
& \leq  \frac{10 L}{T } (\frac{1-\lambda}{ \eta KL}) \left(\mathcal{F}\left(z^{0}\right)-\mathcal{F}\left(z^{*}\right)\right) + \frac{\eta K L}{1-\lambda}\left[\left\{A \left(\frac{(1-\lambda)}{K}+\frac{1}{K}\right)\right.\right. \\
&\quad \left .  +\left(\frac{5}{2}+(1-\lambda)\left(\frac{5}{K}+2\right)\right) \sigma^2 +\left\{A\left((1-\lambda)^{2}+4\right)+(10(1-\lambda))\right\} \sigma_{g}^{2} \right] \\
& \quad +\left(\frac{\eta K L}{1-\lambda}\right)^{2}\left[A\left(\frac{1-\lambda}{20 K} \sigma^2+\frac{(1-\lambda)^2}{10} \sigma_g^2\right)\right]
\end{aligned}
$$

Similar to the proof of Lemma 2 of the SCAFFOLD~\citep{karimireddy2019scaffold}, if we choose $\eta_{\max } \leq \frac{1-\lambda}{100\left(B^{2}+1\right) K L} $, we can have
$$
\begin{aligned}
\frac{1}{T} \sum_{t=1}^{T}\mathbb{E} \|\nabla \mathcal{F}\left(\theta_{0}^{t}\right) \|^{2} & \leq \frac{1000\left(B^{2}+1\right) L}{T}\left(\mathcal{F}\left(z^{0}\right)-\mathcal{F}\left(z^{*}\right)\right) \\
& \quad +\frac{2}{\sqrt{T}}\left[\left(10 L (\mathcal{F}\left(z^{0}\right)-\mathcal{F}\left(z^{*}\right))\right) \right. \left[\{ A\left(\frac{2-\lambda}{K}\right) +\left(\frac{5}{2}+(1-\lambda)\left(\frac{5}{K}+2\right)\right)\} \sigma^2  \right .\\
& \quad\left.\left.+\left\{A\left((1-\lambda)^{2}+4\right)+(10(1-\lambda))\right\} \delta_{g}^{2}\right]\right]^{\frac{1}{2}}\\
& \quad + \frac{2}{T^{\frac{2}{3}}}\left(100 L^{2}\left(\mathcal{F}\left(z^{0}\right)-\mathcal{F}\left(z^{*}\right)\right)^{2} \right. \left.\left[A\left(\frac{1-\lambda}{20K} \sigma^2+\frac{(1-\lambda)^2}{10} \sigma_g^2\right]\right]\right)^{\frac{1}{3}}
\end{aligned}
$$

We then complete the proof by noting that $\theta_0^t = \theta^{t-1} + \lambda m^{t-1}$.
\end{proof}
\end{theorem}

% \begin{lemma}\label{lem:converge_nonconvex}

% \begin{proof}
% \end{proof}
% \end{lemma}

\begin{lemma}\label{lem:converge_nonconvex}
For proving~\cref{thm:1}, we first prove the key Lemma below.
Let $z^t = \theta^t + \frac{\lambda}{1 - \lambda} m^t$, $\Delta^t_i =\theta_{i}^{t}-(\theta^{t-1} + \lambda m^{t-1}) =\sum_{k=0}^{K-1}-\eta\nabla f_{i}(\theta^{t}_{i,k})$, $\delta^t = \frac{1}{N}\sum_{i \in [N]}\sum_{k=0}^{K-1}-\eta\nabla \mathcal{F}_{i}(\theta^{t}_{i,k})$, $e^t =\Delta^t - \delta^t$, and $\theta_0^t = \theta^{t-1} + \lambda m^{t-1}$,
%Note that $\mathbb E[e^t] = 0$
\begin{align*}
\mathbb{E}\big[\mathcal{F}\left(z^{T}\right)-\mathcal{F}\left(z^{0}\right)\big] & \leq T \textrm{C}_8 \sigma^{2}+T \textrm{C}_{9} \sigma_g^{2}+\textrm{C}_{10} \sum_{t=1}^{T} \mathbb{E}\|\nabla \mathcal{F}\left(\theta_{0}^{t}\right)\|^{2}
\end{align*}
where $\textrm{C}_{8} \leq \left(\frac{\eta k}{1-\lambda}\right)^{2} L\left[(\frac{5}{2}+ (1-\lambda)(\frac{5}{K} + 2)) + \frac{1}{K}\left\{(1-\lambda) + 1 + \frac{\eta K L }{20}\right\}A \right]$, $\textrm{C}_{9}\leq (\frac{\eta K}{1-\lambda})^2 L\left[ 10(1-\lambda) +  \frac{\eta K}{1-\lambda}\frac{1-\lambda}{10}LA +  A\left((1-\lambda^2) +4 \right) \right]$, and $\textrm{C}_{10} \leq- \frac{\eta k}{10(1-\lambda)}$, respectively.

\begin{proof} 
\begin{align*}
\mathcal{F}(z^{t+1}) 
&\leq \mathcal{F}(z^{t}) + \langle\nabla\mathcal{F}(z^{t}), z^{t+1} - z^{t} \rangle +\frac{L}{2}\|z^{t+1} - z^{t}\|^2 
\\&= \mathcal{F}(z^{t}) + \frac{1}{1-\lambda} \langle\nabla\mathcal{F}(z^{t}), \Delta^{t+1} \rangle +\frac{L}{2(1-\lambda)^2}\|\Delta^{t+1}\|^2
\\&= \mathcal{F}(z^{t}) + \frac{1}{1-\lambda} \langle\nabla\mathcal{F}(z^{t}), (e^{t+1}+\delta^{t+1}) + \eta K\nabla\mathcal{F}(\theta_0^{t+1}) - \eta K\nabla\mathcal{F}(\theta_0^{t+1}) \rangle \\ & \quad +\frac{L}{2(1-\lambda)^2}\|\Delta^{t+1}\|^2
\\&= \mathcal{F}(z^{t}) + \frac{1}{1-\lambda} \langle\nabla\mathcal{F}(z^{t}), e^{t+1}\rangle + \frac{1}{1-\lambda} \langle\nabla\mathcal{F}(z^{t}), \delta^{t+1}+\eta K\nabla\mathcal{F}(\theta_0^{t+1})\rangle
\\& \quad - \frac{\eta K}{1-\lambda} \langle\nabla\mathcal{F}(z^{t}), \nabla\mathcal{F}(\theta_0^{t+1})\rangle +\frac{L}{2(1-\lambda)^2}\|\Delta^{t+1}\|^2
\\& = \mathcal{F}(z^{t}) + \frac{1}{1-\lambda} \langle\nabla\mathcal{F}(z^{t}), e^{t+1}\rangle + \frac{1}{1-\lambda} \langle\nabla\mathcal{F}(z^{t}), \delta^{t+1}+\eta K\nabla\mathcal{F}(\theta_0^{t+1})\rangle
\\& \quad 
- \frac{\eta K}{1-\lambda} \langle\nabla\mathcal{F}(z^{t}) - \nabla\mathcal{F}(\theta_0^{t+1}), \nabla\mathcal{F}(\theta_0^{t+1})\rangle
- \frac{\eta K}{1-\lambda}\|\nabla\mathcal{F}(\theta_0^{t+1})\|^2 \\
& \quad +\frac{L}{2(1-\lambda)^2}\|\Delta^{t+1}\|^2
\end{align*}
First inequality comes from the $L$-smoothness of the loss function $\mathcal{F}$. Note that $\theta_0^{t+1}=\theta^{t} + \lambda m^{t}$ represents the accelerated global model and serves as the initial point for the local models of the participating local clients at the round $t+1$, meaning that $\theta_0^{t+1} =\theta_{i,0}^{t+1}$ holds for $\text{each client}~ i \in S_t$.
By taking expectation on both sides, we get following equation.
%Second equality comes from $z^{t+1}-z{t}= (\theta^{t+1}-\theta^t) + \frac{\lambda}{1-\lambda}(m^{t+1}-m^t)$.
\begin{align*}
\mathbb{E}[\mathcal{F}(z^{t+1}) -\mathcal{F}(z^{t})] 
& \leq \frac{1}{1-\lambda} \mathbb{E}\left[\left\langle\nabla \mathcal{F}\left(z^{t}\right), \delta^{t+1}+\eta K \nabla \mathcal{F}\left(\theta_{0}^{t+1}\right)\right\rangle\right] \\
& \quad -\frac{\eta K}{1-\lambda} \mathbb{E}\left[\left\langle\nabla \mathcal{F}\left(z^{t}\right)-\nabla \mathcal{F}\left(\theta_{0}^{t+1}\right), \nabla \mathcal{F}\left(\theta_{0}^{t+1}\right)\right\rangle\right] \\
& \quad -\frac{\eta K}{1-\lambda} \mathbb{E}\left\|\nabla \mathcal{F}\left(\theta_{0}^{t+1}\right)\right\|^{2}+\frac{L}{2(1-\lambda)^{2}} \mathbb{E}\left\|\Delta^{t+1}\right\|^{2} \\
& \leq \frac{K^{2} L}{2(1-\lambda)}\underbrace{ \mathbb{E}\left\|\eta \nabla \mathcal{F}\left(z^{t}\right)\right\|^{2}}_{\text{I}^*}+\frac{1}{2(1-\lambda) K^{2} L} \underbrace{\mathbb{E} \| \frac{1}{\eta}\left(\delta^{t+1}+\eta K \nabla \mathcal{F}\left(\theta_{0}^{t+1}\right) \right)\|^{2}}_{\text{II}^*} \\
& \quad +\frac{\eta K}{2(1-\lambda)} \underbrace{\mathbb{E}\left\|\nabla \mathcal{F}\left(z^{t}\right)-\nabla \mathcal{F}\left(\theta_{0}^{t+1}\right)\right\|^{2}}_{\text{III}^*} +\frac{\eta K}{1-\lambda}\left(\frac{1}{2}-1\right) \mathbb{E}\left\|\nabla \mathcal{F}\left(\theta_{0}^{t+1}\right)\right\|^{2} \\
& \quad +\frac{L}{2(1-\lambda)^{2}}
 \underbrace{\mathbb{E}\left\|\Delta^{t+1}\right\|^{2}}_{\text{IV}^*}\\ %+\underbrace{\mathbb{E}\left\|\delta^{t}\right\|^{2}}_{\text{V}^*}
\end{align*}

The first ineqaulity holds because $\mathbb{E}[e^{t+1}]=0$.
The second inequality comes from the \cref{lem:triangle}.
Now we have to find the upper bound of four terms depicted in the last inequality.
To do so, we will first define a few terms for our analysis.
\begin{align*}
C_{i}^{t} & =\mathbb{E}\left\|\sum_{k=0}^{K-1}-\eta \nabla \mathcal{F}_{i}\left(\theta_{i, k}^{t}\right)\right\|^{2} \! \! \!  , \ \ C^{t}=\frac{1}{N} \sum_{i \in N} C_{t}^{i}
\end{align*}

\begin{align*}
I_{i, k}^{t} =\mathbb{E}\|\theta_{i, k}^{t}-\theta_{i, 0}^{t}\|^{2}, \ \
I_{i}^{t}=\sum_{k=0}^{K-1} I_{i, k}^{t}, \ \
I^{t} =\frac{1}{N} \sum_{i \in N} I_{i}^{t}
\end{align*}

$C_{i}^{t}$ is the expectation of the local updates for each client $i$ at $t^{\text{th}}$ global round, and $I_{i,k}^{t}$ is the expectation of the parameter difference between local model and the initial point of a local model at each $k^{\text{th}}$ local iteration.
Using the above definition, the upper bound of $\text{I}^*$, $\text{II}^*$, $\text{III}^*$, and $\text{IV}^*$ are handled in \cref{lem:I_nonconvex}, \cref{lem:II_nonconvex}, \cref{lem:III_nonconvex}, and \cref{lem:IV_nonconvex}, respectively.
Substituting the upper bounds for the four items yields the following result.

\begin{align*}
\mathbb{E}[\mathcal{F}(z^{t+1}) -\mathcal{F}(z^{t})] & \leq \frac{K^{2} L}{2(1-\lambda)}\left\{\frac{2 \eta^{2} L^{2} \lambda^{4}}{(1-\lambda)^{2}} \mathbb{E}\left\|m^{t}\right\|^{2}+2 \eta^{2}\mathbb{E}\left\|\nabla \mathcal{F}\left(\theta_{0} ^{t+1}\right)\right\|^{2}\right\} +\frac{L}{2(1-\lambda) K} I^{t+1}\\
&\quad+\frac{\eta K}{2(1-\lambda)} \frac{\lambda^{4} L^{2}}{(1-\lambda)^{2}} \mathbb{E}\left\|m^{t}\right\|^{2} \\
& \quad - \frac{\eta K}{2(1-\lambda)} \mathbb{E}\left\|\nabla \mathcal{F}\left(\theta_{0}^{t+1}\right)\right\|^{2} +\frac{L}{2(1-\lambda)^{2}} \eta^{2} K^{2} \sigma^{2} +\frac{L}{2(1-\lambda)^{2}}AC^{t+1}\\
& =\frac{L^{2} \lambda^{4}}{(1-\lambda)^{2}}\left\{\frac{L \eta^{2} K^{2}}{1-\lambda}+\frac{\eta K}{2(1-\lambda)}\right\} \mathbb{E}\left\|m^{t}\right\|^{2}\\
&\quad+\frac{L}{2(1-\lambda) K} I^{t+1}+\frac{L}{2(1-\lambda)^{2}} \eta^{2} K^{2} \sigma^{2} \\
&\quad +\frac{L}{2(1-\lambda)^{2}}AC^{t+1} +\frac{\eta K}{1-\lambda}\left(-\frac{1}{2}+\eta K L\right) \mathbb{E}\left\|\nabla \mathcal{F}\left(\theta_{0}^{t+1}\right)\right\|^{2},\\
\end{align*}
where $A=1+\frac{4N}{(N-1)|S_t|}(1-\frac{|S_t|}{N})$. By substituting the upper bound of $I^{t}$ and $C^{t}$ handled in \cref{lem:I^t} and \cref{lem:C^t},

\begin{align*}
\mathbb{E}[\mathcal{F}(z^{t+1}) -\mathcal{F}(z^{t})] \leq \textrm{C}_{4} \mathbb{E}\|m^t\|^{2}+\textrm{C}_5 \sigma^2+\textrm{C}_6 \sigma_g^2+\textrm{C}_{7} \mathbb{E} \left\|\nabla \mathcal{F}\left(\theta_{0}^{t+1}\right)\right\|^{2}
\end{align*},
where $\textrm{C}_{4} = \frac{L^{2} \lambda^{4}}{(1-\lambda)^{2}}\left\{\frac{L \eta^{2} K^{2}}{1-\lambda}+\frac{\eta K}{2(1-\lambda)}\right\}$, $\textrm{C}_5 = \frac{\eta^2 K^2 L}{2(1-\lambda)^2} +   \frac{5 \eta^2 K L}{(1-\lambda)} + \frac{10 \eta^4 K^3 L^3}{(1-\lambda)^2}A$, $\textrm{C}_6 = \frac{10\eta^2 K^2 L}{1-\lambda} + \frac{20 \eta^4 K^4 L^3}{(1-\lambda)^2}A + \frac{\eta^2 K^2 L}{(1-\lambda)^2}A$, and $\textrm{C}_{7} = (\frac{10\eta^2 K^2 L}{1-\lambda} + \frac{20 \eta^4 K^4 L^3}{(1-\lambda)^2}A + \frac{\eta^2 K^2 L}{(1-\lambda)^2}A)B^2 + \frac{\eta K}{1-\lambda}\left( 
 -\frac{1}{2} + \eta K L\right)$, respectively.
By summing the above inequalities for $t = 0,\dots,T-1$, 
\begin{align*}
\mathbb{E}[\mathcal{F}\left(z^{T}\right)-\mathcal{F}\left(z^{0}\right)] =T\left(\textrm{C}_5 \sigma^2+\left(\textrm{C}_6 \sigma_g^2\right)+\textrm{C}_{7} \mathbb{E} \sum_{t=1}^{T}\left\|\nabla \mathcal{F}\left(\theta_{0}^{t}\right)\right\|^{2}\right) 
 +\textrm{C}_{4} \sum_{t=1}^{T} \mathbb{E}\left\|m^{t-1}\right\|^{2} ,
\end{align*}

By substituting the upper bound of $\sum\limits_{t=1}^{T} \mathbb{E}\left\|m^{t-1}\right\|^{2}$ handled in \cref{lem:m^t} and organizing the coefficients of each term, we can get following result.
\begin{align*}
\mathbb{E}\big[\mathcal{F}\left(z^{T}\right)-\mathcal{F}\left(z^{0}\right)\big] & \leq T \textrm{C}_8 \sigma^{2}+T \textrm{C}_{9} \sigma_g^{2}+\textrm{C}_{10} \sum_{t=1}^{T} \mathbb{E}\|\nabla \mathcal{F}\left(\theta_{0}^{t}\right)\|^{2}
\end{align*}
where 
\begin{align*}
\textrm{C}_{8} &=\left(\frac{\eta K}{1-\lambda}\right)^{2}\left(\frac{L}{2}+\frac{5 L}{K}(1-\lambda)
+\left(\frac{\eta K L}{1-\lambda}\right)^2 \frac{10 L (1-\lambda)}{K}A\right)\\
%+\frac{10 \eta^{2} K^{2} L^{3}}{K(1-\lambda)}A\right) \\
& \quad +\left(\frac{\eta K}{1-\lambda}\right)^{2} \frac{\lambda^{4}}{(1-\lambda)^{4}} L\left\{n K L+\frac{1}{2}\right\} (\eta K L (1 - \lambda) + 20 \frac{\eta^3 K^3 L^3}{K}A)
\end{align*}

\begin{align*}
\textrm{C}_{9} &= \frac{10 \eta^{2} K^{2} L}{(1-\lambda)} +\frac{20 \eta^{4} K^{4} L^{3}}{(1-\lambda)^{2}}A +\frac{\eta^{2} K^{2} L}{(1-\lambda)^{2}}A \\
& \quad +\frac{L^{2} \lambda^{4}}{(1-\lambda)^{4}}\left\{\frac{L^{2} \eta^2 K^{2}}{1-\lambda}+\frac{\eta K}{2(1-\lambda)}\right\} A (40 \eta^4 K^4 L^2 + 2 \eta^2 K^2)
\end{align*}
\begin{align*}
\textrm{C}_{10}&=\left[\frac{10 \eta^{2} K^{2} L}{(1-\lambda)} +\frac{20 \eta^{4} K^{4} L^{3}}{(1-\lambda)^{2}} A +\frac{n^{2} K^{2} L}{(1-\lambda)^{2}}A\right] B^{2}  +\frac{\eta K}{1-\lambda}\left(-\frac{1}{2}+\eta K L\right) \\
& \quad +\frac{L^{2} \lambda^{4}}{(1-\lambda)^{4}}\left[\left\{\frac{L \eta^{2} K^{2}}{1-\lambda}+\frac{\eta K}{2(1-\lambda)}\right\}B^2 A (40 \eta^4 K^4 L^2 + 2 \eta^2 K^2) \right]
\end{align*}
The optimal value of $\lambda$, which minimizes the upper bound of $\mathbb{E}\big[\mathcal{F}\left(z^{T}\right)-\mathcal{F}\left(z^{0}\right)\big]$, lies within the interval of 0 to 1.
Within the specified range defined by $\lambda^2 \leq 25(1-\lambda) \Rightarrow \lambda \leq 0.962 \approx 1$, and with the appropriate selection of $\eta$, an increase in $\lambda$ results in a decrease in the upper bound of $\mathbb{E}\big[\mathcal{F}\left(z^{T}\right)-\mathcal{F}\left(z^{0}\right)\big]$.
In the conditions described above, with respect to $\eta$ and $\lambda$,  we have following upper bounds for $\mathrm{C}_{8}$, $\mathrm{C}_{9}$, and $\mathrm{C}_{10}$,

\begin{align*}
\textrm{C}_{8} \leq \left(\frac{\eta k}{1-\lambda}\right)^{2} L\left[(\frac{5}{2}+ (1-\lambda)(\frac{5}{K} + 2)) + \frac{1}{K}\left\{(1-\lambda) + 1 + \frac{\eta K L }{20}\right\}A \right]
\end{align*}
\begin{align*}
\textrm{C}_{9}\leq (\frac{\eta K}{1-\lambda})^2 L\left[ 10(1-\lambda) +  \frac{\eta K}{1-\lambda}\frac{1-\lambda}{10}LA +  A\left((1-\lambda^2) +4 \right) \right]
\end{align*}
\begin{align*}
\textrm{C}_{10} \leq - \frac{\eta k}{10(1-\lambda)}
\end{align*}
which gives us the desired result.
\end{proof}
\end{lemma}

\begin{lemma}\label{lem:I_nonconvex}
$\mathbb{E}\|\eta \nabla \mathcal{F}\left(z^{t}\right)\|^{2}$ in the proof of \cref{lem:converge_nonconvex} has following bound.
\begin{align*}
\mathbb{E}\|\eta \nabla \mathcal{F}\left(z^{t}\right)\|^{2} \leq
2\eta^{2} L^{2}\frac{\lambda^{4}}{1-\lambda} \mathbb{E}\|m^{t}\|^{2}+2 \eta^{2}\mathbb{E}\|\nabla \mathcal{F}\left(\theta_{0}^{t+1}\right)\|^{2}
\end{align*}

\begin{proof}
\begin{align*}
\mathbb{E}\|\eta \nabla \mathcal{F}\left(z^{t}\right)\|^{2}&
=\mathbb{E}\|\eta \nabla \mathcal{F}\left(z^{t}\right) - \eta \nabla \mathcal{F}\left(
\theta_{i,0}^{t+1}\right) + \eta \nabla \mathcal{F}\left(
\theta_{i,0}^{t+1}\right)\|^{2} \\
& \leq 2 \eta^{2} L^{2}\mathbb{E}\|\frac{\lambda^{2}}{1-\lambda} m^{t}\|^{2}+2 \eta^{2}\mathbb{E}\|\nabla \mathcal{F}\left(\theta_{0}^{t+1}\right)\|^{2} \\
& \leq 2 \eta^{2} L^{2}\frac{\lambda^{4}}{(1-\lambda)^2} \mathbb{E}\|m^{t}\|+2 \eta^{2}\mathbb{E}\|\nabla \mathcal{F}\left(\theta_{0}^{t+1}\right)\|^{2} 
\end{align*}
\end{proof}
\end{lemma}

\begin{lemma}\label{lem:II_nonconvex}
 ${\mathbb{E}}\|\frac{1}{\eta}(\delta^{t+1}+\eta K\nabla\mathcal{F}(\theta_0^{t+1}))\|^2$ in the proof of \cref{lem:converge_nonconvex} has following bound.
\begin{align*}
{\mathbb{E}}\|\frac{1}{\eta}(\delta^{t+1}+\eta K\nabla\mathcal{F}(\theta_0^{t+1}))\|^2 \leq L^2 K I^{t+1}
\end{align*}
\begin{proof}

\begin{align*}
{\mathbb{E}\|\frac{1}{\eta}(\delta^{t+1}+\eta K\nabla\mathcal{F}(\theta_0^{t+1}))\|^2} &= {\mathbb{E}[\|\frac{1}{\eta}(\delta^{t+1}+\eta K\nabla\mathcal{F}(\theta^t+\lambda m^t))\|^2}
\\&= {\mathbb{E}\|\frac{1}{N}\sum_{i \in [N]}\sum_{k=0}^{K-1}\{-\nabla \mathcal{F}_{i}(\theta^{t+1}_{i,k})
+\nabla\mathcal{F}_i(\theta^t+\lambda m^t))\}\|^2}
\\& \leq \frac{K}{N}\sum_{i \in [N]}\sum_{k=0}^{K-1}{\mathbb{E}\|\{-\nabla \mathcal{F}_{i}(\theta^{t+1}_{i,k})
+\nabla\mathcal{F}_i(\theta^t+\lambda m^t))\}\|^2}
\\& \leq \frac{L^2 K}{N}\sum_{i \in [N]}\sum_{k=0}^{K-1}{\mathbb{E}\| \theta^{t+1}_{i,k}
-\theta^{t+1}_{i,0}\|^2}\\
& = L^2 K I^{t+1}
\end{align*}
Inequality in the third line comes from Jensen's inequality.
Inequality in the fourth line is derived by the smoothness of the objective function.
Equality in the last line use the definition of $I^{t}$.

\end{proof}
\end{lemma}

\begin{lemma}\label{lem:III_nonconvex}
$\mathbb{E} \| \nabla \mathcal{F}(z^t) - \nabla \mathcal{F}(\theta_0^{t+1}) \|^2$ in the proof of~\cref{lem:converge_nonconvex} has the following bound for any $0 \leq \lambda < 1$,
\begin{align*}
\mathbb{E} \| \nabla \mathcal{F}(z^t) - \nabla \mathcal{F}(\theta_0^{t+1}) \|^2 \leq \frac{\lambda^4 L^2}{(1-\lambda)^2} \mathbb{E} \| m^t \|^2
\end{align*}
\end{lemma}
\begin{proof}
\begin{align*}
\mathbb{E} \| \nabla \mathcal{F}(z^t) - \nabla \mathcal{F}(\theta^t + \lambda m^t) \|^2 & \leq L^2 \mathbb{E} \| \frac{\lambda^2}{1-\lambda} m^t\|^2 = \frac{\lambda^4 L^2}{(1-\lambda)^2} \mathbb{E} \| m^t \|^2 \\
\end{align*}
where the inequality comes from the $L$-smoothness of the global loss function $\mathcal{F}$.
\end{proof}

\begin{lemma}\label{lem:IV_nonconvex}
$\mathbb{E}\|\Delta^{t}\|^{2}$ in the proof of~\cref{lem:converge_nonconvex} has the following bound,
\begin{align*}
\mathbb{E}\|\Delta^{t}\|^{2} \leq \eta^{2} K^{2} \sigma^2+A C_{t},
\end{align*}
where $A=1+\frac{4N}{(N-1)|S_t|}(1-\frac{|S_t|}{N})$
\begin{proof}
$ \mathbb{E} \|\Delta^{t}\|^{2} =\mathbb{E} \| \delta^t \|^2 + \mathbb{E} \| \Delta^t - \delta^t \|^2$. 

For the first term $\mathbb{E} \| \delta^t \|^2$, we can derive upper bound as
\begin{align*}
\mathbb{E} \|\delta^t\|^2 =\mathbb{E} \| \frac{1}{N}\sum_{i \in [N]}\sum_{k=0}^{K-1}-\eta\nabla \mathcal{F}_{i}(\theta^{t}_{i,k})\|^2 \leq \frac{1}{N}\sum_{i \in [N]} \mathbb{E} \| \sum_{k=0}^{K-1}-\eta\nabla \mathcal{F}_{i}(\theta^{t}_{i,k})\|^2 = C^t,
\end{align*}
where the inequality from Jensen's inequality.

For the second term $\mathbb{E} \| \Delta^t - \delta^t \|^2$,
\begin{align*}
\mathbb{E} \| \Delta^t - \delta^t \|^2 & = \mathbb{E}\|\Delta^t + \frac{\eta}{|\mathcal{S}_t|} \sum_{i \in \mathcal{S}_t} \sum^{K-1}_{k=0} \nabla \mathcal{F}_i (\theta^t_{i, k}) - \frac{\eta}{|\mathcal{S}_t|} \sum_{i \in \mathcal{S}_t} \sum^{K-1}_{k=0} \nabla \mathcal{F}_i (\theta^t_{i, k}) + \frac{\eta}{N} \sum_{i \in [N]} \sum^{K-1}_{k=0} \nabla \mathcal{F}_i (\theta^t_{i, k}) \|^2 \\
& = \mathbb{E} \| \frac{\eta}{|\mathcal{S}_t|}\sum_{i \in \mathcal{S}_t}\sum_{k=0}^{K-1} \nabla f_i(\theta^{t}_{i,k}) - \nabla \mathcal{F}_i(\theta^t_{i,k})\|^2 + \mathbb{E} \| \frac{\eta}{|\mathcal{S}_t|} \sum_{i\in \mathcal{S}_t} \sum_{k=0}^{K-1} \nabla \mathcal{F}_i(\theta^t_{i,k}) - \delta^t \|^2 \\
& \leq  \frac{\eta^2}{|\mathcal{S}_t|} \sum_{i \in \mathcal{S}_t} \sum_{k=0}^{K-1} \mathbb{E}\|\nabla f_i(\theta^{t}_{i,k}) - \nabla \mathcal{F}_i(\theta^t_{i,k})\|^2 + \mathbb{E} \| \frac{\eta}{|\mathcal{S}_t|} \sum_{i\in \mathcal{S}_t} \sum_{k=0}^{K-1} \nabla \mathcal{F}_i(\theta^t_{i,k}) - \delta^t \|^2 \\
& = \eta^2K^2\sigma^2 + \underbrace{\mathbb{E} \| \frac{\eta}{|\mathcal{S}_t|} \sum_{i\in \mathcal{S}_t} \sum_{k=0}^{K-1} \nabla \mathcal{F}_i(\theta^t_{i,k}) - \delta^t \|^2}_{\text {(A)}} \\
\end{align*}
In (A), we take expectation with respect to $\mathcal{S}_t$ and total clients $N$.
For that, we use Lemma 4 of~\citep{reisizadeh2020fedpaq}.
Specifically, using Eq. (59) in~\citep{reisizadeh2020fedpaq}, we get:
\begin{align*}\
(\text{A}) & \leq \frac{\eta^2}{|\mathcal{S}_t|^2}\Big(\frac{|\mathcal{S}_t|}{N} - \frac{|\mathcal{S}_t|(|\mathcal{S}_t|-1)}{N(N-1)}\Big)\sum_{i \in [N]} \mathbb{E} \|\sum_{k=0}^{K-1} \nabla \mathcal{F}_i(\theta^t_{i, k}) - \frac{\delta^t}{\eta} \|^2 \\
& \leq \frac{\eta^2}{|\mathcal{S}_t|^2}\Big(\frac{|\mathcal{S}_t|}{N} - \frac{|\mathcal{S}_t|(|\mathcal{S}_t|-1)}{N(N-1)}\Big) \Big( 2 \sum_{i \in [N]} \mathbb{E}\| \sum_{k=0}^{K-1} \nabla \mathcal{F}_i(\theta)\|^2 + \frac{2}{N}\sum_{i\in[N]} \mathbb{E} \| \sum_{k=0}^{K-1} \nabla \mathcal{F}_i(\theta^t_{i, k}) \|^2 \Big) \\
& \leq \frac{4N}{|\mathcal{S}_t|^2}\Big(\frac{|\mathcal{S}_t|}{N} - \frac{|\mathcal{S}_t|(|\mathcal{S}_t|-1)}{N(N-1)}\Big)  \frac{1}{N}\sum_{i\in [N]} \mathbb{E} \| \sum_{k=0}^{K-1} -\eta \nabla \mathcal{F}_i(\theta^t_{i, k})\|^2 \\
& \leq \frac{4N}{|\mathcal{S}_t|^2}\Big(\frac{|\mathcal{S}_t|}{N} - \frac{|\mathcal{S}_t|(|\mathcal{S}_t|-1)}{N(N-1)}\Big)  C^t \\
&= \frac{4N}{(N-1)|S_t|}(1-\frac{|S_t|}{N})  C^t
\end{align*}
This gives us the desired result.
\end{proof}
\end{lemma}

\begin{lemma}\label{lem:I^t}
$I^{t}$ in the proof of~\cref{lem:converge_nonconvex} has the following bound 
\begin{align*}
I^{t} & \leq 20 \eta^{2} K^{3}\left(\delta_{g}^{2}+B^{2}\mathbb{E}\|\nabla \mathcal{F}\left(\theta_{i, 0}^{t}\right)\|^{2}\right)+10 \eta^{2} K^{2} \sigma^2
\end{align*}

\begin{proof} Initially, we commence by deriving an upper bound for the variable $I_{i,k}^t$ 
\begin{align*}
I_{i,k}^t
& =\mathbb{E}\|\theta_{i, k}^{t}-\theta_{i, 0}^{t}\|^{2} \\
& = \mathbb{E}\|\theta_{i, k-1}^{t}-\theta_{i, 0}^{t}-\eta \nabla {f}_{i}\left(\theta_{i, k-1}^{t}\right)\|^{2} \\
& = \mathbb{E}\|\theta_{i, k-1}^{t}-\theta_{i, 0}^{t} -\eta \nabla {\mathcal{F}}_{i}\left(\theta_{i, k-1}^{t}\right) +\eta \nabla {\mathcal{F}}_{i}\left(\theta_{i, k-1}^{t}\right) -\eta \nabla {f}_{i}\left(\theta_{i, k-1}^{t}\right)\|^{2} \\
& \leq \mathbb{E}\|\theta_{i, k-1}^{t}-\theta_{i, 0}^{t} -\eta \nabla {\mathcal{F}}_{i}\left(\theta_{i, k-1}^{t}\right) \|^{2} + \eta^{2}\sigma^2 \\
& \leq\left(1+\frac{1}{K-1}\right) \mathbb{E}\|\theta_{i, k-1}^{t}-\theta_{i, 0}^{t}\|^{2}+K \eta^{2}\mathbb{E}\|\nabla \mathcal{F}_{i}\left(\theta_{i, k-1}^{t}\right)\|^{2}+\eta^{2} \sigma^2 \\
\end{align*}
The inequality in the fourth line is established due to the stochastic bounded variance assumption, while the inequality in the fifth line holds as a consequence of the \cref{lem:triangle}.
Now, let us proceed to determine the upper bound for $\mathbb{E}\|\nabla \mathcal{F}_{i}\left(\theta_{i, k-1}^{t}\right)\|^{2}$.
\begin{align*}
\mathbb{E}\|\nabla \mathcal{F}_{i}\left(\theta_{i, k-1}^{t}\right)\|^{2} 
& = \mathbb{E}\|\nabla \mathcal{F}_{i}\left(\theta_{i, k-1}^{t}\right) - \nabla \mathcal{F}_{i}\left(\theta_{i, 0}^{t}\right) + \nabla \mathcal{F}_{i}\left(\theta_{i, 0}^{t}\right)\|^{2}\\
&\leq 2\mathbb{E}\|\nabla \mathcal{F}_{i}\left(\theta_{i, k-1}^{t}\right) - \nabla \mathcal{F}_{i}\left(\theta_{i, 0}^{t}\right)\|^{2} + 2\mathbb{E}\|\nabla \mathcal{F}_{i}\left(\theta_{i, 0}^{t}\right)\|^{2} \\
&\leq 2L^2\mathbb{E}\|\theta_{i, k-1}^{t} - \theta_{i, 0}^{t}\|^{2} + 2\mathbb{E}\|\nabla \mathcal{F}_{i}\left(\theta_{i, 0}^{t}\right)\|^{2}
\end{align*}
In the last inequality, we rely on the L-smoothness property of the local loss function for its validity. 
Substituting the derived upper bound for $\mathbb{E}\|\nabla \mathcal{F}_{i}\left(\theta_{i, k-1}^{t}\right)\|^{2}$ into our original expression,
\begin{align*}
I_{i,k}^t
& \leq\left(1+\frac{1}{K-1}+2 K \eta^{2} L^{2}\right) \mathbb{E}\|\theta_{i, k-1}^{t}-\theta_{i, 0}^{t}\|^{2}+2 K \eta^2\mathbb{E}\|\nabla \mathcal{F}_{i}\left(\theta_{i,0}^{t}\right)\|^{2}+\eta^{2} \sigma^2 \\
& \leq\left(1+\frac{1}{K-1}+2 K \eta^{2} L^{2}\right) I_{i, k-1}^t+2 K \eta^2\mathbb{E}\|\nabla \mathcal{F}_{i}\left(\theta_{i,0}^{t}\right)\|^{2}+\eta^{2} \sigma^2 \\
\end{align*}
Expanding the aforementioned recursion,
\begin{align*}
I_{i, k}^{t} 
\leq \sum_{r=0}^{k-1}\left(2 K \eta^{2} \mathbb{E}[\|\nabla \mathcal{F}_{i}\left(\theta_{i,0}^{t}\right)\|^{2}]+\eta^{2} \sigma^2\right)\left(1+\frac{3}{K-1}\right)^{r} 
\leq 10 K\left(2 K \eta^{2} \mathbb{E}\|\nabla \mathcal{F}_{i}\left(\theta_{i, 0}^{t}\right)\|^{2}+\eta^{2} \sigma^2\right)
\end{align*}
Utilizing the above results, we can sequentially derive the upper bounds for $I_{i}^t$ and $I^t$.
\begin{align*}
I_{i}^{t} & =\sum_{k=0}^{K-1} I_{i, k}^{t} \leq 10 K^{2}\left(2 K \eta^{2} \mathbb{E}\|\nabla \mathcal{F}_{i}\left(\theta_{i, 0}^{t}\right)\|^{2}+\eta^{2} \sigma^2\right) \\
& =20\eta^{2} K^{3}\mathbb{E}\|\nabla \mathcal{F}_{i}\left(\theta_{i, 0}^{t}\right)\|^{2}+10 \eta^{2} K^{2} \sigma^2
\end{align*}

\begin{align*}
I^{t} &= 20 \eta^{2} K^{3} \frac{1}{N} \sum_{i \in [N]} \mathbb{E}\|\nabla \mathcal{F}_{i}\left(\theta_{i, 0}^{t}\right)\|^{2}+ 10 \eta^{2} K^{2} \sigma^2 \\
& \leq 20 \eta^{2} K^{3}\left(\delta_{g}^{2}+B^{2}\mathbb{E}\|\nabla \mathcal{F}\left(\theta_{i, 0}^{t}\right)\|^{2}\right)+10 \eta^{2} K^{2} \sigma^2 \\
\end{align*}
The final inequality holds due to the assumption related to the averaged norm of the local gradient. This gives us the desired result.

\end{proof}
\end{lemma}

\begin{lemma}\label{lem:C^t}
$C^{t}$ in the proof of~\cref{lem:converge_nonconvex} has the following bound 
\begin{align*}
C^{t}
\leq 20 \eta^{4} K^{3} L^{2} \sigma^2+\left(40 \eta^{4} K^{4} L^{2}+2 \eta^{2} K^{2}\right)\left(\sigma_g^2+B^{2}\mathbb{E}\|\nabla \mathcal{F}\left(\theta_{i, 0}^{t}\right)\|^{2}\right)
\end{align*}

\begin{proof}
Initially, we commence by deriving an upper bound for the variable $C_{i}^t$ 
\begin{align*}
C_{i}^{t} & =\mathbb{E}\left\|\sum_{k=0}^{K-1}-\eta \nabla \mathcal{F}_{i}\left(\theta_{i, k}^{t}\right)\right\|^{2} \\
& \leq K \eta^{2} \sum_{k=0}^{K-1} \mathbb{E}\left\|\nabla \mathcal{F}_{i}\left(\theta_{i, k}^{t}\right)\right\|^{2} \\
& =K \eta^{2} \sum_{k=0}^{K-1} \mathbb{E}\left\|\nabla \mathcal{F}_{i}\left(\theta_{i, k}^{t}\right)-\nabla \mathcal{F}_{i}\left(\theta_{i, 0}^{t}\right)+\nabla \mathcal{F}_{i}\left(\theta_{i, 0}^{t}\right)\right\|^{2} \\
& \leq 2 K \eta^{2} \sum_{k=0}^{K-1}\big(\underbrace{\mathbb{E} \| \nabla \mathcal{F}_{i}\left(\theta_{i, k}^{t}\right) -\nabla \mathcal{F}_{i}\left(\theta_{i, 0}^{t}\right)}_{L \text { smooth }} \|^{2} +\mathbb{E}\| \nabla \mathcal{F}_{i}\left(\theta_{i, 0}^{t}\right)\|^{2}\big)  \\
& \leq 2 K \eta^{2} \sum_{k=0}^{K-1} \big( L^{2} \mathbb{E}\|\theta_{i, k}^{t}-\theta_{i, 0}^{t}\|^{2}+\mathbb{E}\|\nabla \mathcal{F}_{i}\left(\theta_{i, 0}^{t}\right)\|^{2} \big) \\
& =2 K \eta^{2}\left(L^{2} I_{i}^{t}+K \mathbb{E}[\|\nabla \mathcal{F}_{i}\left(\theta_{i, 0}^{t}\right)\|^{2}]\right)
\end{align*}
The initial and fourth line inequalities are established based on Jensen's inequality.
Using the aforementioned results, we can determine the upper bound for $C^{t}$.
\begin{align*}
C^{t} & = \frac{1}{N} \sum_{i \in N} C_{t}^{i} \leq \frac{1}{N} \sum_{i \in N}\left\{2 K \eta^{2}\left(L^{2} I_{i}^{t}+ K \mathbb{E}[\|\nabla \mathcal{F}_{i}\left(\theta_{i, 0}^{t}\right)\|^{2}]\right)\right\} \\
& =2 K \eta^{2} L^{2} I^{t}+2 \eta^{2} K^{2} \frac{1}{N} \sum_{i \in N} \mathbb{E}[\|\nabla \mathcal{F}_{i}\left(\theta_{i, 0}^{t}\right)\|^{2}] \\
& \leq 20 \eta^{4} K^{3} L^{2} \sigma^2+\left(40 \eta^{4} K^{4} L^{2}+2 \eta^{2} K^{2}\right)\left(\sigma_g^2+B^{2}\mathbb{E}[\|\nabla \mathcal{F}\left(\theta_{i, 0}^{t}\right)\|^{2}]\right)\\
\end{align*}
Where the last inequality is established based on the assumption related to the averaged norm of the local gradient and \cref{lem:I^t}.
\end{proof}
\end{lemma}

\begin{lemma}\label{lem:m^t}
$\sum\limits_{t=1}^{T} \mathbb{E}\left\|m^{t-1}\right\|^{2}$ in the proof of~\cref{lem:converge_nonconvex} has the following bound 
\begin{align*}
\sum\limits_{t=1}^{T} \mathbb{E}\left\|m^{t-1}\right\|^{2} 
\leq \frac{T}{(1-\lambda)^{2}}\left(\textrm{C}_{1} \sigma^2+\textrm{C}_2 \sigma_g^2\right) +\frac{1}{(1-\lambda)^{2}} \textrm{C}_{3} \mathbb{E} \sum_{t=1}^{T}\left\|\nabla \mathcal{F}\left(\theta_{0}^{t}\right)\right\|^{2},
\end{align*}
where $\textrm{C}_1=\eta^{2} K^{2} +20\eta^{4}K^{3}L^{2} A$, $\textrm{C}_2=A\left(40\eta^{4}K^{4}L^{2} + 2\eta^2K^{2}\right)$, and $\textrm{C}_3=B^{2}A\left(40\eta^{4}K^{4}L^{2} + 2\eta^2K^{2}\right)$.
\begin{proof}

\end{proof}
First, let's unrolling the recursion of the momentum $m^t$,~\ie $m^t = \sum_{r=0}^{t} \lambda^{t-r}\Delta^r$.
\begin{align*}
\mathbb{E}\left\|m^{t}\right\|^{2}&
=\mathbb{E} \| \sum_{r=0}^{t} \lambda^{t-r}\Delta^r \|^2
\end{align*}
Let $\Gamma_{t}=\sum_{r=0}^{t} \lambda^r=\frac{1-\lambda^t}{1-\lambda}$. For $0 \leq \lambda < 1$, $\Gamma_{t} \leq \frac{1}{1-\lambda}$. Then,
\begin{align*}
\mathbb{E}\| \sum_{r=0}^t \lambda^{t-r} \Delta^r \|^2 & =  \Gamma_t^2 \mathbb{E}\| \frac{1}{\Gamma_t} \sum_{r=1}^t \lambda^{t-r} \Delta^r\|^2 \\
& \leq  \Gamma_t \sum_{r=1}^{t} \lambda^{t-r} \mathbb{E} \| \Delta^r\|^2 \leq \frac{1}{1-\lambda} \sum_{r=1}^{t} \lambda^{t-r} \mathbb{E} \| \Delta^r\|^2
\end{align*}
Using above results, we can get 
\begin{align*}
\sum\limits_{t=1}^{T} \mathbb{E}\left\|m^{t-1}\right\|^{2}
&\leq \sum_{t=1}^{T-1} \sum_{r=1}^{t} \frac{\lambda^{t-r}}{1-\lambda}\mathbb{E} \| \Delta^r\|^2  \\
& \leq \sum_{t=1}^{T-1} \sum_{r=1}^{t} \frac{\lambda^{t-r}}{1-\lambda}\biggl( \underbrace{\left(\eta^{2} K^{2} +20\eta^{4}K^{3}L^{2} A\right)}_{\textrm{C}_1} \sigma^2 \\
& + \underbrace{A\left(40\eta^{4}K^{4}L^{2} + 2\eta^2K^{2}\right)}_{\textrm{C}_2} \sigma_g^2 \\
& + \underbrace{B^{2}A\left(40\eta^{4}K^{4}L^{2} + 2\eta^2K^{2}\right)}_{\textrm{C}_3}\mathbb{E} \left\|\nabla \mathcal{F}\left(\theta_{0}^{r}\right)\right\|^{2}\biggl) \\
& \leq \frac{T}{(1-\lambda)^{2}}\left(\textrm{C}_{1} \sigma^2+\textrm{C}_{2} \sigma_g^2\right) +\frac{1}{1-\lambda}\left(\textrm{C}_{3} \sum_{t=1}^{T-1} \sum_{r=1}^{t} \lambda^{t-r}\mathbb{E} \left\|\nabla \mathcal{F}\left(\theta_{0}^{r}\right)\right\|^{2}\right) \\
& \leq \frac{T}{(1-\lambda)^{2}}\left(\textrm{C}_{1} \sigma^2+\textrm{C}_2 \sigma_g^2\right) +\frac{1}{(1-\lambda)^{2}} \textrm{C}_{3} \mathbb{E} \sum_{t=1}^{T}\left\|\nabla \mathcal{F}\left(\theta_{0}^{t}\right)\right\|^{2}
\end{align*}
\end{lemma}
The inequality in the second line can be obtained by substituting the result of Lemma \ref{lem:C^t} into Lemma \ref{lem:III_nonconvex}.
The inequality in the six line can be obtained by summing the coefficients corresponding to each $\left\|\nabla \mathcal{F}(\theta_{0}^{t})\right\|^{2}$, respectively.
\begin{lemma}\label{lem:triangle}
(Relaxed triangle inequality).
For any $a>0$, $\left\|\boldsymbol{v}_1+\boldsymbol{v}_2\right\|^2 \leq(1+a)\left\|\boldsymbol{v}_1\right\|^2+\left(1+\frac{1}{a}\right)\left\|\boldsymbol{v}_2\right\|^2$
\begin{proof}
This lemma holds because when we organize the formulas on the right, we get $0 \leq {\|a \boldsymbol{v}_1 - \frac{\boldsymbol{v}_2}{a}\|}^2 $.
\end{proof}
\end{lemma}
