# Supplementary material for: Communication-Efficient Federated Learning with Accelerated Client Gradient
Source: arXiv:2201.03172 source file (2024-04-01)
Supplement: Supplementary file 2 [file supplementary.pdf]

# Communication-Efficient Federated Learning with Acceleration of Global Momentum: *Supplementary Material*

Anonymous CVPR submission

Paper ID 7205

## 1. Evaluation on Tiny-ImageNet

We found a small mistake in our implementation for the experiments on the Tiny-ImageNet dataset, and report the correct numbers in Tab. 1. Also, for consistency with the results on other datasets, we present the results at round 500 and 1000.

To validate the performance of the proposed method on a more realistic dataset, we compare FedAGM with the baselines on Tiny-ImageNet in the two federated settings: one with 100 total clients and 5% client participation, and the other with 500 clients and 2% client participation. In both settings, local epochs and local iterations are set to 5 and 50 respectively. Tab. 1 shows that FedAGM achieves the state-of-the-art performance for all cases. This validates that FedAGM not only works well on small datasets, but shows good performance on more realistic large-scale datasets. Fig. 1 also shows that FedAGM consistently outperforms the compared methods every communication rounds. Note that FedAGM shows a faster convergence rate, especially at the early stage of training, than other algorithms.

Table 1. Comparison of federated learning methods on Tiny-ImageNet with two different settings. Accuracy at the target round and the communication round to reach target test accuracy are based on running exponential moving average with parameter 0.9. The arrows indicate whether higher ( $\uparrow$ ) or lower ( $\downarrow$ ) is better. The best performance in each column is denoted by **bold**. Note that we put wrong results of FedAGM on Tiny-ImageNet of Tab. 1 and 2 in the main paper due to our mistake, and here are the correct results of FedAGM, which is denoted by an asterisk (\*). We apologize for the confusion.

| Method         | 5%,100 clients              |              |                             |            | 2%,500 clients              |              |                             |            |
|----------------|-----------------------------|--------------|-----------------------------|------------|-----------------------------|--------------|-----------------------------|------------|
|                | accuracy ( $\%, \uparrow$ ) |              | rounds ( $\#, \downarrow$ ) |            | accuracy ( $\%, \uparrow$ ) |              | rounds ( $\#, \downarrow$ ) |            |
|                | 500R                        | 1000R        | 35%                         | 38%        | 500R                        | 1000R        | 24%                         | 30%        |
| FedAvg [4]     | 33.94                       | 35.42        | 645                         | 1000+      | 23.63                       | 29.48        | 523                         | 1000+      |
| FedProx [3]    | 34.14                       | 35.53        | 613                         | 1000+      | 25.45                       | 31.71        | 445                         | 799        |
| FedAvgm [2]    | 36.32                       | 38.51        | 416                         | 829        | 26.75                       | 33.26        | 386                         | 687        |
| FedAdam [5]    | 33.22                       | 38.91        | 658                         | 945        | 21.88                       | 28.08        | 648                         | 1000+      |
| FedDyn [1]     | 38.86                       | 42.82        | 327                         | 440        | 27.74                       | 37.25        | 387                         | 580        |
| FedCM [6]      | 31.61                       | 37.87        | 694                         | 1000+      | 19.41                       | 24.09        | 975                         | 1000+      |
| FedAGM* (ours) | <b>42.26</b>                | <b>46.31</b> | <b>226</b>                  | <b>331</b> | <b>31.47</b>                | <b>38.48</b> | <b>246</b>                  | <b>447</b> |

## 2. Evaluation on Low Participation Rate with a Large Number of Clients

The low participation rate and the large number of clients are factors that make the convergence of federated learning difficult. To show the robustness to client heterogeneity and participation rates, we perform experiments when both factors are present, that is when the total number of clients is 500 and the participation rate is 1%. Local epochs and local iterations are set to 5 and 50, respectively. Note that this setting makes each client have a very small number of training examples and increases client heterogeneity significantly. Tab. 2 again shows that FedAGM has the best performance on all metrics. Note that the performance gap between FedAGM and its strongest competitor, FedDyn, becomes larger than when the participation rate is 2%: from 1.37%p to 1.68%p in CIFAR 10 and from 3.39%p to 4.76%p in CIFAR 100 at round 1000.

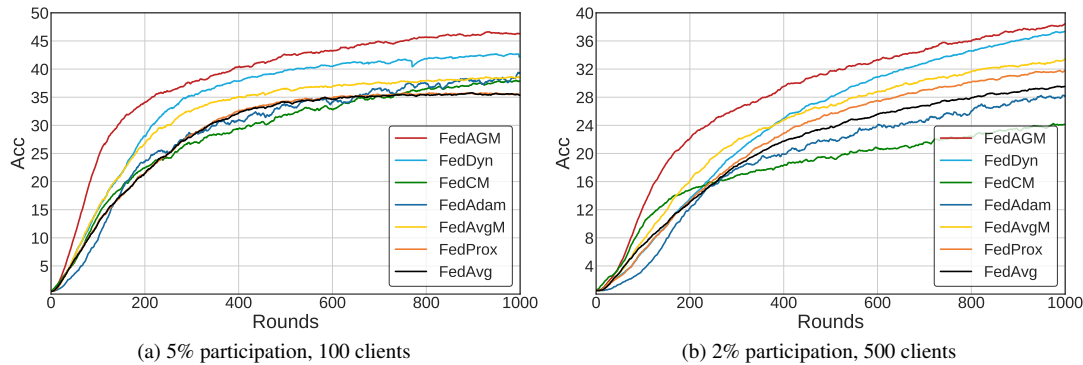

Figure 1. The convergence plot of FedAGM and the compared methods on Tiny-ImageNet with the different levels of client heterogeneity.

Table 2. Comparison of federated learning methods on CIFAR-10 and CIFAR-100 with the large number of clients (500): Dirichlet (0.3) split on low client participation (1%). Accuracy at the target round and the communication round to reach target test accuracy are based on running exponential moving average with parameter 0.9. The arrows indicate whether higher ( $\uparrow$ ) or lower ( $\downarrow$ ) is better. The best performance in each column is denoted by **bold**.

| Method        | CIFAR-10                       |              |                                |            | CIFAR-100                      |              |                                |            |
|---------------|--------------------------------|--------------|--------------------------------|------------|--------------------------------|--------------|--------------------------------|------------|
|               | accuracy ( $\%$ , $\uparrow$ ) |              | rounds ( $\#$ , $\downarrow$ ) |            | accuracy ( $\%$ , $\uparrow$ ) |              | rounds ( $\#$ , $\downarrow$ ) |            |
|               | 500R                           | 1000R        | 64%                            | 68%        | 500R                           | 1000R        | 30%                            | 35%        |
| FedAvg [4]    | 54.71                          | 68.96        | 792                            | 949        | 26.94                          | 35.69        | 636                            | 950        |
| FedProx [3]   | 55.18                          | 69.80        | 773                            | 919        | 26.92                          | 35.41        | 648                            | 963        |
| FedAvgm [2]   | 57.82                          | 71.12        | 669                            | 812        | 29.29                          | 39.36        | 530                            | 755        |
| FedAdam [5]   | 47.97                          | 55.11        | 1000+                          | 1000+      | 17.72                          | 23.92        | 1000+                          | 1000+      |
| FedDyn [1]    | 58.28                          | 74.77        | 621                            | 752        | 29.68                          | 40.42        | 512                            | 703        |
| FedCM [6]     | 49.21                          | 60.38        | 1000+                          | 1000+      | 16.32                          | 22.59        | 1000+                          | 1000+      |
| FedAGM (ours) | <b>63.70</b>                   | <b>76.45</b> | <b>509</b>                     | <b>618</b> | <b>31.74</b>                   | <b>45.18</b> | <b>458</b>                     | <b>581</b> |

### 3. Effect of More Local Iterations

The increase of local iterations under non-iid environments is prone to result in more divergence across client models and degraded performance of an algorithm. We evaluate the accuracy and communication-efficiency of the proposed method with aggravated client heterogeneity by varying the number of local iterations, *i.e.*,  $K \in \{50, 70, 100\}$ , on CIFAR-100. In this experiments, the number of clients, participation rate, and Dirichlet parameter is set to 100, 5% and 0.3, respectively. Tab. 3 presents that FedAGM outperforms the compared methods consistently for all cases in terms of accuracy and communication efficiency.

Table 3. Comparison of federated learning methods with three different local iterations on CIFAR-100: Dirichlet (0.3) split on 5% client participation out of 100 clients. Accuracy at the target round and the communication round to reach target test accuracy are based on running exponential moving average with parameter 0.9. The arrows indicate whether higher ( $\uparrow$ ) or lower ( $\downarrow$ ) is better. The best performance in each column is denoted in **bold**.

| Local iterations<br>Methods | $K = 50$                       |              |                                |            | $K = 70$                       |              |                                |            | $K = 100$                      |              |                                |            |
|-----------------------------|--------------------------------|--------------|--------------------------------|------------|--------------------------------|--------------|--------------------------------|------------|--------------------------------|--------------|--------------------------------|------------|
|                             | accuracy ( $\%$ , $\uparrow$ ) |              | rounds ( $\#$ , $\downarrow$ ) |            | accuracy ( $\%$ , $\uparrow$ ) |              | rounds ( $\#$ , $\downarrow$ ) |            | accuracy ( $\%$ , $\uparrow$ ) |              | rounds ( $\#$ , $\downarrow$ ) |            |
|                             | 500R                           | 1000R        | 47%                            | 53%        | 500R                           | 1000R        | 47%                            | 53%        | 500R                           | 1000R        | 47%                            | 53%        |
| FedAvg [4]                  | 41.88                          | 47.83        | 924                            | 1000+      | 42.45                          | 48.29        | 852                            | 1000+      | 41.92                          | 48.16        | 896                            | 1000+      |
| FedProx [3]                 | 42.43                          | 48.32        | 881                            | 1000+      | 43.31                          | 49.54        | 752                            | 1000+      | 42.01                          | 48.17        | 888                            | 1000+      |
| FedAvgm [2]                 | 46.98                          | 53.29        | 515                            | 936        | 46.17                          | 52.34        | 544                            | 1000+      | 45.72                          | 52.74        | 578                            | 1000+      |
| FedAdam [5]                 | 44.80                          | 52.48        | 691                            | 1000+      | 43.76                          | 49.19        | 756                            | 1000+      | 43.00                          | 47.51        | 994                            | 1000+      |
| FedDyn [1]                  | 52.66                          | 58.46        | 293                            | 504        | 52.85                          | 59.98        | 326                            | 509        | 51.98                          | 59.13        | 347                            | 532        |
| FedCM [6]                   | 52.44                          | 58.06        | 293                            | 572        | 48.30                          | 54.89        | 467                            | 812        | 46.90                          | 54.20        | 502                            | 893        |
| FedAGM (ours)               | <b>55.79</b>                   | <b>62.51</b> | <b>260</b>                     | <b>389</b> | <b>54.23</b>                   | <b>61.23</b> | <b>295</b>                     | <b>459</b> | <b>54.71</b>                   | <b>63.12</b> | <b>284</b>                     | <b>461</b> |

## 4. Sensitivity to $\lambda$

$\lambda$  controls how much the server projects the current model toward the global gradient to initialize the local update. To further analyze the effect of  $\lambda$  on the performance of FedAGM algorithms, we evaluate the accuracy of the proposed method with different client heterogeneity by varying  $\lambda$  as  $\{0.75, 0.8, 0.85, 0.9, 0.95\}$ , on CIFAR-10. Tab. 4 shows that the proposed algorithm outperforms most baselines regardless of  $\lambda$ , and the proposed method shows steady results in terms of the choices of  $\lambda$  for different client heterogeneity.

Table 4. Sensitivity to  $\lambda$  of FedAGM in terms of accuracy [%] at rounds 1000 on CIFAR-10. Three different levels of client heterogeneity are tested, and the number of clients and participation rate are set to 500 and 2%, respectively.

| $\lambda$       | 0.75  | 0.8   | 0.85  | 0.9   | 0.95  |
|-----------------|-------|-------|-------|-------|-------|
| Dirichlet (0.3) | 81.32 | 82.52 | 82.80 | 81.82 | 78.25 |
| Dirichlet (0.6) | 83.97 | 84.89 | 85.28 | 84.56 | 82.07 |
| IID             | 85.52 | 86.92 | 86.83 | 87.08 | 84.37 |

## 5. Hyperparameter Setting

Our hyperparameter setting is as follows. For the experiments on CIFAR-10 and CIFAR-100, we choose 5 as the number of local training epochs (50 iterations) and 0.1 as the local learning rate. We set the batch size of the local update to 50 and 10 for the 100 and 500 client participation, respectively. The learning rate decay parameter of each algorithm is selected from  $\{0.995, 0.998, 1\}$  to achieve the best performance. The global learning rate is set to 1, except for FedAdam, which is tested with 0.01. For the experiments on Tiny-ImageNet, we match the total local iterations of local updates with other benchmarks by setting the batch size of local update as 100 and 20 for the 100 and 500 client participation, respectively.

As for algorithm-dependent hyperparameters,  $\alpha$  in FedCM is selected from  $\{0.1, 0.3, 0.5\}$ ,  $\alpha$  in FedDyn is selected from  $\{0.001, 0.01, 0.1\}$ , and  $\alpha$  in FedAGM is selected from  $\{0.9, 1.0\}$ .  $\tau$  in FedAdam is set to 0.001.  $\beta$  in FedAvgM is selected from  $\{0.4, 0.6, 0.8\}$ , and  $\beta$  in FedProx and FedAGM is selected from  $\{0.1, 0.01, 0.001\}$ . For FedAGM,  $\lambda$  is selected from  $\{0.8, 0.85, 0.9\}$  and  $\tau$  is selected from  $\{0.2, 1.0\}$ .

**Reproducibility statement** More details for the implementation and hyperparameters are organized at the demo code in the supplementary material, and we will release the source code to facilitate the reproduction of our results.

## References

- [1] Durmus Alp Emre Acar, Yue Zhao, Ramon Matas, Matthew Mattina, Paul Whatmough, and Venkatesh Saligrama. Federated learning based on dynamic regularization. In *ICLR*, 2021. 1, 2
- [2] Tzu-Ming Harry Hsu, Hang Qi, and Matthew Brown. Measuring the effects of non-identical data distribution for federated visual classification. *arXiv preprint arXiv:1909.06335*, 2019. 1, 2
- [3] Tian Li, Anit Kumar Sahu, Manzil Zaheer, Maziar Sanjabi, Ameet Talwalkar, and Virginia Smith. Federated optimization in heterogeneous networks. In *MLSys*, 2020. 1, 2
- [4] Brendan McMahan, Eider Moore, Daniel Ramage, Seth Hampson, and Blaise Aguerre y Arcas. Communication-efficient learning of deep networks from decentralized data. In *AISTATS*, 2017. 1, 2
- [5] Sashank J Reddi, Zachary Charles, Manzil Zaheer, Zachary Garrett, Keith Rush, Jakub Konečný, Sanjiv Kumar, and Hugh Brendan McMahan. Adaptive federated optimization. In *ICLR*, 2021. 1, 2
- [6] Jing Xu, Sen Wang, Liwei Wang, and Andrew Chi-Chih Yao. Fedcm: Federated learning with client-level momentum. *arXiv preprint arXiv:2106.10874*, 2021. 1, 2
